# Supplementary material for: PersonaChatBench: Evaluating Chat Assistants with Diverse Simulated Users
Source: arXiv:2610.42060 source file (2026-10-30)
Supplement: Supplementary file 1 [file dataset_details.tex]

% Evidence freeze: PersonaChatBench 431476e2ca89d1989c0a618488cff953322d17d3.
% Every prose paragraph occupies one physical source line.
\section{Dataset Details and Development Results}
\label{app:dataset-details}
This appendix records the shared evidence freeze for the HelpBench and Travel adapters. Their task construction, persona banks, and development results appear in Appendices~\ref{app:helpbench} and~\ref{app:travel}. All counts and results are frozen at \bench repository commit \texttt{431476e2} (full identifier in the source comment), including the artifacts published with the scale-up readiness repairs. A task is a source question or authored scenario; an episode is one task--condition--trial conversation. Reusing a persona across tasks does not create new unique personas. \tabref{tab:development-inventory} separates historical evaluation from later functional checks: the latter verify the revised pipeline on small inputs and do not update the historical estimates. All experiments below use the recorded Azure deployment \texttt{gpt-6-astra} for the assistant, simulated user, and model-based judges, with low reasoning effort and an 8,192-token maximum output. The artifacts identify the deployment name rather than an independently pinned model-weights snapshot. Travel task rewards are computed deterministically, without a model judge.

\begin{table}[htbp]
\appendixtablestyle
\caption{Available evidence by protocol version. ``Valid'' means successfully graded and accepted by the simulator audit; it does not imply independently verified correctness. A condition includes a persona or a control. Every cohort has one trial per condition.}
\label{tab:development-inventory}
\begin{tabular}{@{}L{0.24\linewidth}L{0.17\linewidth}L{0.18\linewidth}L{0.10\linewidth}L{0.16\linewidth}@{}}
\toprule
Cohort & Selected tasks & Conditions per task & Planned & Valid graded \\
\midrule
HelpBench v2 & 450 source & 3 personas + 2 controls & 2,250 & 2,081 \\
HelpBench v3 check & 1 source & 3 personas & 3 & 3 \\
Travel v1.3 pilot & 5 source + 5 authored & 3 personas & 30 & 30 \\
Travel v1.4 check & 1 source development & 3 personas & 3 & 3 \\
\bottomrule
\end{tabular}
\end{table}
