# Supplementary material for: PersonaChatBench: Evaluating Chat Assistants with Diverse Simulated Users
Source: arXiv:2610.42060 source file (2026-10-30)
Supplement: Supplementary file 2 [file helpbench.tex]

\clearpage
\section{HelpBench: Security and Privacy Help-Seeking}
\label{app:helpbench}

\subsection{Source Tasks and Preparation}
HelpBench contains 450 English questions about digital privacy, safety, and security, with question-specific expert rubrics \citep{meiklejohn2026helpbench}. Our adapter imports the original question, criterion text, criterion identifiers, signed weights, topic metadata, and ordering metadata without rewriting them. The local snapshot has nine primary topics with 50 questions each (\tabref{tab:helpbench-topics}); a question can additionally carry multiple topic flags. The upstream dataset and autorater are obtained from the anonymous help-seeking repository, and their Apache-2.0 notice is retained in \path{helpbench-benchmark/references/HelpBench-LICENSE}. Because the anonymous repository is mutable, the imported source is identified by SHA-256 beginning \texttt{d1bc8ed2b43f1603}; the complete digest is recorded in the 350-task selection manifest.

The assistant answers the original help-seeking question, and a simulated user can request clarification or explanation in later turns. Persona attributes affect communication preferences; they do not authorize new incident facts, expertise, access rights, completed actions, or changes to the original question. The assistant receives the question and public dialogue, while the user receives the question, its private card, and the dialogue. Neither generation role receives the expert rubric. Rubric grading, need grading, and simulator auditing use separate calls with role-specific inputs. These boundaries support an evaluation of conversational advice, not a measurement of whether a real incident was resolved.

\begin{table}[htbp]
\appendixtablestyle
\caption{HelpBench v2 coverage by primary topic. Each row has 50 tasks and 250 planned conditions. Counts include both controls and all three personas.}
\label{tab:helpbench-topics}
\begin{tabular}{@{}L{0.48\linewidth}rr@{}}
\toprule
Primary topic & Completed conversations & Valid graded \\
\midrule
Accounts & 249 & 245 \\
Compromise & 250 & 243 \\
Data concerns & 250 & 238 \\
Harassment & 207 & 193 \\
Moderation tools & 245 & 240 \\
Platform actions & 245 & 234 \\
Privacy tools & 245 & 243 \\
Scams & 220 & 199 \\
Security tools & 250 & 246 \\
\midrule
Total & 2,161 & 2,081 \\
\bottomrule
\end{tabular}
\end{table}

\subsection{Persona Attributes and Needs}
The bank uses six deliberately authored binary attributes, giving $2^6=64$ possible combinations. Three combinations are prespecified and reused across tasks: careful learner, skeptical questioner, and concise pragmatist (\tabref{tab:helpbench-attributes}). A deterministic compiler maps the selected values to a coherent behavioral description and six assistant-facing need specifications, one per attribute. Explanation depth and terminology are the two designated critical needs. The bank contains three unique profiles, not 64 evaluated profiles or 1,350 independently designed people. The design follows the repository's attribute-composition approach; it is not an empirical distribution of users and does not infer demographic traits. For example, a preference for precise wording does not establish technical expertise, and a supportive tone preference does not establish distress. The schema is in \path{config/persona_dimensions.json}, assignments in \path{config/personas.json}, and the current canonical bank in \path{data/persona.json}, relative to \path{helpbench-benchmark/}. Independent human selection remains pending.

\begin{table}[htbp]
\appendixtablestyle
\caption{HelpBench persona assignments. The two starred attributes generate critical needs. All value labels describe communication preferences.}
\label{tab:helpbench-attributes}
\begin{tabular}{@{}L{0.25\linewidth}L{0.21\linewidth}L{0.21\linewidth}L{0.21\linewidth}@{}}
\toprule
Attribute & Careful learner & Skeptical questioner & Concise pragmatist \\
\midrule
Explanation depth$^*$ & Detailed & Detailed & Concise \\
Terminology$^*$ & Plain language & Precise terms & Plain language \\
Response structure & Stepwise & Answer first & Answer first \\
Evidence preference & Practical reason & Scrutinize assumptions & Practical reason \\
Tone & Supportive & Matter of fact & Matter of fact \\
Uncertainty presentation & Essential caveats & Explicit boundaries & Essential caveats \\
\bottomrule
\end{tabular}
\end{table}

\subsection{Historical v2 Protocol and Coverage}
The dataset-wide experiment consists of two disjoint cohorts of 100 and 350 tasks, using matching v2 prompts, persona definitions, code digests, and model settings. Each task has five planned conditions: a single-turn control, a neutral multi-turn control, and three persona multi-turn conditions. A cached first assistant reply to the same persona-free question is shared across those conditions. Multi-turn conditions permit at most three assistant replies, counting the shared opening. Under v2, the first continuing persona follow-up has a fixed disclosure prefix expressing all six communication preferences; a user can also stop after the opening without disclosure. This prompted disclosure differs materially from the current natural-expression protocol.

\tabref{tab:helpbench-attrition} accounts for all 2,250 planned conditions. All 450 task IDs were attempted, but only 430 tasks have all five conversations generated, 375 have all five successfully graded, and 370 have all five graded and model-audited valid. Seventeen tasks have no saved shared response, accounting for 85 missing conditions; three further tasks have partial conversations and four failed conditions. Of the completed conversations, 75 lack successful grades and five graded simulations are invalid. The older 100-task snapshot records a content-filter response during a recovery attempt for its three missing tasks. Detailed API errors were not retained for the 14 newly missing tasks, so their causes cannot be assigned retrospectively. Missing results are not silently assigned zero. Retry histories also differ: the first cohort includes bounded recovery, while grading of the second was interrupted and resumed without a complete retained history of overwritten failures.

\begin{table}[htbp]
\appendixtablestyle
\caption{HelpBench v2 attrition. Generation outcomes partition planned conditions; successful and failed grades partition completed conversations; valid and invalid audits partition successful grades.}
\label{tab:helpbench-attrition}
\begin{tabular}{@{}L{0.48\linewidth}rrr@{}}
\toprule
Outcome & First 100 & Remaining 350 & Combined \\
\midrule
Planned conditions & 500 & 1,750 & 2,250 \\
Completed conversations & 485 & 1,676 & 2,161 \\
Missing conversations & 15 & 70 & 85 \\
Failed conversations & 0 & 4 & 4 \\
Successfully graded & 470 & 1,616 & 2,086 \\
Failed grades & 15 & 60 & 75 \\
Model-audited invalid simulations & 1 & 4 & 5 \\
Valid graded conversations & 469 & 1,612 & 2,081 \\
\bottomrule
\end{tabular}
\end{table}

\subsection{Evaluation}
Let $w_j$ be the signed weight of rubric item $j$ and $y_j\in\{\mathrm{yes},\mathrm{no}\}$ indicate whether the described behavior occurs. HelpBench awards credit for a positive behavior being present and a negative behavior being absent:
\begin{equation}
T=\frac{\sum_{j:w_j>0}w_j\,\mathbb{1}[y_j=\mathrm{yes}]+\sum_{j:w_j<0}|w_j|\,\mathbb{1}[y_j=\mathrm{no}]}{\sum_j|w_j|}.
\label{eq:helpbench-credit}
\end{equation}
A negative item judged ``yes'' therefore earns no credit for that item; its absolute weight remains in the denominator. Unresolved judgments retain the full denominator and produce lower and upper bounds with no point score. The adapter stores two scopes. The final-response scope treats the last reply as a standalone answer to the original question. The trajectory scope allows maintained positive factual coverage to accumulate across replies and retains a negative behavior if it occurs in any reply, even if later corrected. The separate important-information-at-the-beginning criterion is evaluated on the first assistant reply using the source ordering rule; individual \texttt{at\_beginning} flags do not impose a new timing requirement on every factual item. Trajectory scoring is our multi-turn extension and supplies the task means below; these are not official leaderboard scores.

Historical v2 persona adherence assigns satisfied, partial, and unmet needs scores of 1, 0.5, and 0 and averages the six needs when all are judgeable after disclosure. It is unavailable for conversations ending before disclosure or with unresolved need judgments. The historical implementation also records a local persona pass requiring mean adherence at least 0.75 and fully satisfied critical needs, and a local advice pass requiring trajectory score at least 0.80 without negative factual behavior. These thresholds were not independently calibrated; \tabref{tab:helpbench-results} reports the continuous scores rather than presenting those legacy passes as native benchmark outcomes.

\subsection{Results and Interpretation}

\begin{table}[htbp]
\appendixtablestyle
\caption{HelpBench v2 episode-level means on valid grades, with metric-specific sample sizes. Percentages are rubric/need credit, not question accuracy. The final column is a paired trajectory-score change against the same task's single-turn reply, in percentage points (pp), with pair count. Controls have no persona score.}
\label{tab:helpbench-results}
\begin{tabular}{@{}L{0.28\linewidth}L{0.22\linewidth}L{0.22\linewidth}L{0.18\linewidth}@{}}
\toprule
Condition & Task score ($n$) & Persona adherence ($n$) & Paired change ($n$) \\
\midrule
Single-turn control & 79.77\% (427) & N/A & Reference \\
Neutral multi-turn & 81.82\% (417) & N/A & +1.98 pp (413) \\
Careful learner & 82.75\% (412) & 99.86\% (365) & +3.05 pp (408) \\
Concise pragmatist & 81.35\% (419) & 99.48\% (240) & +1.46 pp (416) \\
Skeptical questioner & 81.77\% (406) & 99.92\% (396) & +2.13 pp (403) \\
\bottomrule
\end{tabular}
\end{table}

The combined means are recomputed over individual episodes, not obtained by averaging the two cohort means. Paired comparisons include only tasks with valid grades in both relevant conditions, so they need not equal the difference between the displayed marginal means. These changes are descriptive: no significance test or confidence interval is supplied, and comparison with a single-turn baseline also changes the amount of interaction. Fifty careful, 187 concise, and ten skeptical completed conversations stop before disclosure, making their persona adherence unavailable. Consequently, near-ceiling adherence describes selected, explicitly disclosed opportunities rather than every planned task--persona episode. Missingness is also topic-dependent (\tabref{tab:helpbench-topics}). Three jointly varying profiles, one stochastic trial, and the same model across generation and judgment do not establish causal attribute effects or generalization to real users.

Conversation length is also limited in the observed data (\tabref{tab:helpbench-turns}). Among 1,728 completed conversations assigned to a multi-turn condition, 394 end after the shared opening, 1,320 contain two assistant replies, and only 14 contain three. These counts include completed conversations regardless of later grading or audit outcome. They support the conclusion that the v2 interaction is usually short; a larger allowed cap alone would not demonstrate longer or more complex dialogue.

\begin{table}[htbp]
\appendixtablestyle
\caption{HelpBench v2 assistant-reply counts, recomputed from completed transcripts in the two frozen cohorts. The shared opening counts as one reply in each condition. These denominators differ from the valid-graded score table.}
\label{tab:helpbench-turns}
\begin{tabular}{@{}L{0.35\linewidth}rrrrr@{}}
\toprule
Condition & Completed & 1 reply & 2 replies & 3 replies & Mean \\
\midrule
Single-turn control & 433 & 433 & 0 & 0 & 1.00 \\
Neutral multi-turn & 432 & 147 & 280 & 5 & 1.67 \\
Careful learner & 433 & 50 & 383 & 0 & 1.88 \\
Concise pragmatist & 432 & 187 & 241 & 4 & 1.58 \\
Skeptical questioner & 431 & 10 & 416 & 5 & 1.99 \\
\bottomrule
\end{tabular}
\end{table}

\subsection{Protocol Versions and Functional Check}
Protocol \texttt{helpbench-persona-v3-standard} composes the shared role prompts with domain instructions and freezes task, persona, prompt, model, and code information in manifests. The fixed disclosure prefix and required single-turn arm are removed; a neutral multi-turn arm is optional. The user responds in its own words to the actual answer, may leave needs undisclosed, and can stop immediately. The default cap is ten assistant replies, with cap/error outcomes retained as incomplete rather than successful primary evaluations. Resume and grading retries preserve matching completed work and archive failed attempts.

In v3, the adherence mean uses only needs judged satisfied, partially satisfied, or not satisfied, with credit 1, 0.5, or 0. Four other statuses---not disclosed, no response opportunity, inapplicable, and not observable---remain unscored and are counted separately. Every scored judgment must cite a public user follow-up and a later assistant response; the shared opening cannot demonstrate persona adaptation. Critical-need pass is true only if all applicable critical needs were expressed, answered, and satisfied; it is false if any answered critical need is partially met or unmet, otherwise unknown, and not applicable if no critical need applies. The legacy mean cutoff is removed. HelpBench has no native binary task-pass threshold, so v3 leaves advice pass and joint success undefined. Simulator validity is separately reported as valid, invalid, or uncertain.

This is the original shared critical-need pass rule, retained by both adapters documented here. The repository's later Coding analysis, \texttt{publicly-expressed-critical-needs-v1}, instead conditions pass on scored critical needs and does not let undisclosed needs block a pass on other scored critical needs. That analysis change does not automatically regrade HelpBench or Travel. Cross-domain tables must therefore identify the pass-rule version rather than treating these quantities as interchangeable.

The v3 functional check uses source task 203 with three personas, one trial, and no control. All three episodes complete in two assistant replies, are successfully graded, and have valid simulator audits. Each obtains trajectory credit $8/9=88.89\%$. Ten of 18 candidate needs are scored, all satisfied; eight remain undisclosed. Five of six applicable critical needs have response opportunities, yielding two true persona passes and one unknown pass (concise pragmatist). Thus a scored-need mean of 1.0 coexists with incomplete critical-need coverage. This three-episode check verifies the repaired workflow and is not a rerun of the 450-task experiment.

\subsection{Representative Case and Reproducibility}
Task 203 describes a Discord account that sent unwanted phishing messages while its password remained unchanged; the user asks how access could have occurred and reports not knowingly entering credentials on third-party sites. The simulator must preserve those facts and distinguish possible mechanisms from an established cause. Across profiles, follow-ups ask for accessible explanation, sharper evidential distinctions, or concise comparisons. All trajectories receive the same rubric credit, while final-reply-only scores are 75.56\% for careful learner, 62.22\% for skeptical questioner, and 44.44\% for concise pragmatist. A short clarification can omit advice already supplied, so this contrast illustrates why final-reply completeness and cumulative conversational advice are different measures; it is not evidence that shorter replies are intrinsically worse. The v2 union report is \path{helpbench-benchmark/examples/gpt6-astra-attributes-v2-450-task/}, with per-condition outcomes, paired comparisons, source pointers, and an offline recomputation script. Its disjoint 100- and 350-task sibling directories retain the dialogues and grades. The v3 check is \path{helpbench-benchmark/examples/gpt6-astra-standard-v3-smoke/}. Recorded v2 final artifacts contain 11,254 calls and 33,946,736 tokens, but omitted retries and failed/discarded attempts prevent interpreting these as billed totals.
