# Supplementary material for: PersonaChatBench: Evaluating Chat Assistants with Diverse Simulated Users
Source: arXiv:2610.42060 source file (2026-10-30)
Supplement: Supplementary file 3 [file law.tex]

Contract redlining requires an assistant to translate a business stakeholder's instructions into legally and commercially appropriate document changes. A useful explanation does not necessarily produce a correct redline, while a technically correct document may leave the stakeholder's questions unresolved. PersonaRedline evaluates these outcomes separately: the tested assistant acts as a lawyer, and a simulated internal deal stakeholder holds the persona. We preserve the source contract and task rubric while varying how the stakeholder seeks advice, expresses needs, and decides whether to continue the conversation.

\subsection{Source Tasks and Preparation}

We use 140 tasks from RedlineBench\footnote{\url{https://huggingface.co/datasets/crosbylegal/RedlineBench}}. These tasks cover 101 input groups across three commercial scenarios. They include related negotiation branches and rubric variants, rather than 140 independent transactions. The imported contracts, grounding documents, attorney references, and signed rubric weights remain unchanged.

Before the lawyer's first response, we record the task facts, represented side, permitted tools, initial question, persona cards, need criteria, model settings, and turn cap. A separate model-based review checks whether the five cards and their needs fit the task and the supplied facts. All five cards must be approved before any conversation for that task begins, including the neutral condition. This keeps the same task panel across conditions.

\subsection{Persona Attributes and Needs}

Five archetypes are instantiated for each task, producing 700 task-specific persona cards. Each card contains 20 attributes: six background attributes, ten behavioral attributes, and four task-priority attributes. The background describes the stakeholder's role, contract familiarity, organizational context, and review resources. The behavioral attributes describe trust in counsel, handling of disagreement, explanation preferences, uncertainty tolerance, risk sensitivity, decision autonomy, context sharing, willingness to revise a position, competing priorities, and planning preferences.

Within a task, the background and task-priority attributes are identical across the five cards. The behavioral configuration changes how the stakeholder approaches the conversation without changing the contract or supplied deal facts. These profiles are authored archetypes, not a sample of real clients.

Each card has three candidate needs, with three criteria per need. Table~\ref{tab:redline-personas} summarizes them. The task-specific criteria are fixed before the lawyer answers. Users can raise several needs together, explain a need over several messages, or stop without mentioning every need. We assess only the parts they express. For example, asking for a recommendation does not also require the lawyer to satisfy a private preference for a short approval note.

\begin{table}[htbp]
\appendixtablestyle
\caption{PersonaRedline archetypes and associated needs. Each task has these five personas and one neutral condition. The neutral user has no private persona card or assigned needs.}
\label{tab:redline-personas}
\begin{tabularx}{\linewidth}{@{}>{\raggedright\arraybackslash}p{0.29\linewidth} >{\raggedright\arraybackslash}X@{}}
\toprule
Persona & Associated needs \\
\midrule
P1: Collaborative planner
& Identify the next business choice and its dependencies; compare supported options across interacting clauses; draft a current internal decision or approval request. \\
P2: Anxious delegator
& Explain the concrete downside and limits of protection; recommend a manageable next step and when to hold or escalate; draft an escalation note that separates known facts from missing input and asks a clear question. \\
P3: Guarded autonomous requester
& Compare options against the stakeholder's priorities; address contrary evidence with precise support; state whether the available information is sufficient and provide a provisional direction or focused follow-up question. \\
P4: Assertive authority-seeker
& Address the actual counterparty objection and relevant contract terms; draft a usable counterparty response; distinguish the primary position from a fallback and preserve any stated order of steps. \\
P5: Trusting, time-pressed decision maker
& Lead with the decision and its priority; provide a self-contained handoff note; give compact supporting references and distinguish facts from assumptions or missing information. \\
\bottomrule
\end{tabularx}
\end{table}

\subsection{Interaction Protocol and Role Visibility}

For each approved task and trial, the initial question is identical across the five personas and the neutral user. We generate the lawyer's first reply once and reuse it unchanged across these six conditions. The neutral user has the same task information but no private persona or assigned needs.

The first lawyer reply has a 250-word target, with accuracy taking priority. This is a prompt instruction rather than a strict cutoff. Later replies and the final document have no general length target. A conversation can contain at most eight complete stakeholder--lawyer exchanges, including the opening pair. Stakeholders may stop earlier, and there is no minimum length or required disclosure of needs. A nonempty closing stakeholder message receives a lawyer reply before the conversation ends.

The lawyer receives the public task context, source contract, authorized grounding materials, and public dialogue. It does not receive the private persona card, need criteria, task rubric, attorney reference redline, or judge feedback. The simulator receives its persona, plain-language needs, authorized stakeholder facts, and the public conversation, but not hidden rubrics, reference answers, or evaluation feedback.

Once the conversation ends, we ask the same model to prepare the final redline from the dialogue and task materials. It returns edit instructions, which our editor applies to the Word contract. This is a separate request after the conversation, so it does not count as another answer to the stakeholder's conversational needs.

The reported documents are built from the saved edit instructions. The main editor applies valid plans while retaining supported tracked changes and comments. A separate recovery procedure handles plans containing unusable requests: it applies valid edits individually, keeps existing wording when an identical replacement can be verified, and skips edits whose target text cannot be found. We retain the applied, skipped, and failed requests for each document. The two procedures have separate records because a complete file under the recovery procedure does not necessarily include every originally requested edit. Neither procedure regenerates the conversation or asks the model for new wording.

\subsection{Evaluation}

\paragraph{Native document performance.}
The document judge evaluates the saved redline against the original RedlineBench rubric. Let $w_{ei}$ be the signed weight of rubric item $i$ for conversation $e$, and let $z_{ei}=1$ when the item receives a \texttt{PASS} verdict. The normalized document score is
\begin{equation}
D_e =
\operatorname{clip}_{[0,1]}
\left(
\frac{\sum_i w_{ei}z_{ei}}
     {\sum_{i:w_{ei}>0}w_{ei}}
\right).
\label{eq:redline-document}
\end{equation}
A positive-weight \texttt{PASS} earns credit; a negative-weight \texttt{PASS} identifies a prohibited pattern and incurs a penalty. We report document scores on a 0--100 scale. The source rubric defines no binary task-pass threshold, so we report continuous scores rather than a task pass or joint pass.

We grade Word documents that pass the document checks, even if some requested edits are unfinished. Editing errors are recorded separately. A partial document can therefore contribute to the average, whereas an absent document or an unresolved grading request has no score. Document performance reflects both the lawyer's proposed work and the editor's ability to apply it. Our multi-turn setup and fixed judge model also differ from the source benchmark's evaluation, so these scores are not directly comparable to official RedlineBench leaderboard results.

\paragraph{Expressed persona needs.}
A criterion is scored only after the stakeholder expresses the relevant request in a message following the shared opening and the lawyer has a chance to answer. A one-time request is assessed in its immediate answer. A continuing preference is also assessed in later replies whenever it still applies, until the stakeholder changes or withdraws it. For example, a request for plain language can apply across topics, whereas a request about a particular decision need not be repeated after that decision is settled. Purely social acknowledgments and unrelated replies are excluded, but a reply that omits requested information still counts as an answer to be judged. Changing or withdrawing a request does not remove its earlier assessments.

Requests for later document changes are separate from requests for an explanation in the conversation. If the stakeholder asks for an explanation now and a Word edit later, we score the explanation in the chat. A promise to make the edit does not satisfy that request, and the final document cannot add conversational credit. Needs that remain private or receive no opportunity for an answer are not scored as failures.

We report sustained needs satisfaction, which averages credit across the relevant replies to each expressed criterion. Each reply receives 1 for satisfied, 0.5 for partially satisfied, or 0 for unmet. For criterion $c$ in conversation $e$, let $x_{ecr}$ be its credit at relevant reply $r$, with $m_{ec}$ such replies. Its sustained credit is
\begin{equation}
\bar{x}_{ec} = \frac{1}{m_{ec}}\sum_{r=1}^{m_{ec}}x_{ecr}.
\end{equation}
Let $\mathcal C_{en}$ contain the scored criteria for need $n$, and let $\mathcal N_e$ contain the needs with at least one scored criterion. The conversation score is
\begin{equation}
S_e = \frac{1}{|\mathcal N_e|}
\sum_{n\in\mathcal N_e}
\frac{1}{|\mathcal C_{en}|}
\sum_{c\in\mathcal C_{en}}\bar{x}_{ec}.
\label{eq:redline-needs}
\end{equation}
We first average criteria within each need, then average the scored needs within a conversation. Each scored conversation contributes equally to the reported mean, which is shown on a 0--100 scale. A conversation with no scored criteria has no needs score. If a required judgment is missing or cannot be resolved from the evidence, the conversation's aggregate remains unavailable. We do not report a binary persona pass.

Some needs concern a requested word limit. A numerical limit is scored only when the stakeholder states it publicly and the parser recognizes it. A private preference for a 35-word note, or a request merely to be concise, does not impose that limit. We count whitespace-separated words, including headings and references. The whole reply is counted unless the user explicitly asks for an uncapped explanation and a separately capped note. Numerical compliance receives 1 or 0.

\paragraph{Simulator validity.}
A separate audit checks whether the simulated stakeholder follows the persona, preserves the authorized facts, respects information boundaries, and stops appropriately. The audit assesses the simulation, not the lawyer's performance. Both document and needs averages include only completed conversations with a valid audit and an available score. The judges cite the relevant evidence, and automated checks verify output structure, quoted passages, and score arithmetic. All planned conversations remain in the coverage counts, including those that were not run or could not be scored.

\subsection{Experimental Setup and Coverage}

GPT-6 Luna with medium reasoning is used for every model role: the lawyer, simulator, preparation reviewer, document finalizer, document judge, needs judge, and simulator auditor. These roles use separate contexts. The study has one trial:
\[
140\ \text{tasks}
\times (5\ \text{personas}+1\ \text{neutral})
=840\ \text{planned conversations}.
\]
This gives 700 assigned persona conversations and 140 neutral conversations.

The preparation reviewer approved 128 task--persona sets and rejected 12. In ten of the rejected sets, it flagged P4 for assuming existing counterparty objections even though the task began with a clean first markup. One of these also contained an unsupported description of the stakeholder's professional background. The other two sets introduced approval steps or an internal organizational role that the reviewer did not find in the task materials. These decisions were made before the lawyer answered. Since each task had five persona conditions and one neutral condition, the 12 exclusions left $12\times6=72$ planned conversations unrun: 60 persona and 12 neutral. The remaining 128 tasks produced 768 completed conversations.

Among the completed conversations, 591 were simulator-valid, 8 invalid, 21 uncertain, and 148 had no accepted audit. Of the 591 valid conversations, 497 were persona conversations and 94 were neutral. There were 767 natural stops, one turn-cap stop, and no recorded chat errors.

Document production yielded 402 complete files and 355 partial files; 11 conversations have no document. Of the 402 complete files, three were produced under the separate recovery procedure and are not claimed to contain every originally requested edit. The other 399 were complete applications under the main editor's rules.

Document grades are available for 750 completed conversations. Of these, 579 contribute to the reported average. The other 171 are excluded because their simulator audit was missing (143), uncertain (20), or invalid (8). Eighteen completed conversations have no document grade: 11 have no Word file, six have unresolved comment evidence, and one grading request has an unknown outcome. Twelve of these 18 conversations are otherwise simulator-valid. Missing grades are not counted as zero.

Needs judgments are available for 522 of the 640 generated persona conversations. Among the 497 valid persona conversations, 442 have a needs score. The remaining 55 have missing judgments, unresolved evidence, or no expressed criteria to score. Table~\ref{tab:redline-results} reports both the averages and their scoring coverage.

\begin{table}[htbp]
\appendixtablestyle
\caption{GPT-6 Luna medium results on a 0--100 scale. Counts show scored conversations out of those planned and those with a valid simulator audit. Document scores include all six conditions; needs scores include persona conditions only.}
\label{tab:redline-results}
\begin{tabularx}{\linewidth}{@{}Xrrr@{}}
\toprule
Measure & Mean & Scored / planned & Scored / valid \\
\midrule
Document score & 45.78 & 579/840 & 579/591 \\
Sustained needs satisfaction & 88.65 & 442/700 & 442/497 \\
\bottomrule
\end{tabularx}
\end{table}

\subsection{Results and Interpretation}

\paragraph{Expressed needs and document quality.}
The average document score is 45.78, while sustained needs satisfaction is 88.65. The two scores measure different outcomes and use different sets of scored conversations. Meeting the stakeholder's expressed needs does not guarantee that the final contract satisfies the source task rubric.

For example, task \texttt{redline-s1-t3-g13a} with P1 received full needs credit on nine criteria across three needs, but its document score was zero. The lawyer provided the requested comparison of liability and indemnity terms and drafted an internal approval request. The document judge nevertheless marked required contract changes as missing. This example shows why we evaluate the conversation and the document separately.

\paragraph{Results by persona.}
Table~\ref{tab:redline-persona-results} reports document and sustained needs scores for each persona and the neutral user. Every condition has 140 planned and 128 completed conversations. The numbers in parentheses give the conversations included in each average.

\begin{table}[htbp]
\appendixtablestyle
\caption{PersonaRedline scores on a 0--100 scale. Parentheses give the number of scored conversations. All averages require a valid simulator audit and an available score.}
\label{tab:redline-persona-results}
\begin{tabularx}{\linewidth}{@{}Xrr@{}}
\toprule
Condition & Document & Sustained needs \\
\midrule
P1: Collaborative planner & 44.70 (94) & 90.58 (83) \\
P2: Anxious delegator & 46.94 (100) & 86.45 (101) \\
P3: Guarded autonomous requester & 46.63 (103) & 92.10 (92) \\
P4: Assertive authority-seeker & 44.65 (93) & 93.09 (89) \\
P5: Trusting, time-pressed decision maker & 46.76 (96) & 80.21 (77) \\
Neutral & 44.81 (93) & --- \\
\midrule
Overall & 45.78 (579) & 88.65 (442) \\
\bottomrule
\end{tabularx}
\end{table}

P4 has the highest needs average, 93.09, while P5 has the lowest, 80.21. Document averages vary less, from 44.65 to 46.94, with the neutral condition at 44.81. P4 has the lowest document average despite its high needs score. The personas ask for different kinds of help, and each average includes a different set of valid, graded conversations. These descriptive differences do not establish that a persona caused better or worse performance.

\paragraph{Scope of the conclusions.}
The study uses authored profiles, related task branches, one trial, and one model for all roles. Human semantic and legal review was not performed. The results describe this task panel and model configuration rather than real-client behavior or a model ranking. High needs scores also do not mean that every private need was expressed or met. Only 34 of the 497 valid persona conversations contained a later relevant reply to an already expressed criterion, so repeated adherence was tested in relatively few conversations.

Document scores depend on the model's proposed edits, the Word editor, and the evidence presented to the judge. Some Word structures and comment contexts remain difficult to process. Automated checks can confirm that a quoted passage appears in the record, but not that its interpretation is legally correct. Two P4 criteria both assess how a clause provides protection; this overlap remains in the reported average. The word-limit parser also has gaps, particularly for some numerical expressions and requests combining an uncapped explanation with a capped note. These limitations should be considered together with the scoring coverage.
