# Supplementary material for: PersonaChatBench: Evaluating Chat Assistants with Diverse Simulated Users
Source: arXiv:2610.42060 source file (2026-10-30)
Supplement: Supplementary file 6 [file coding.tex]

% Coding domain appendix. Every number is taken from data/ in this repository;
% protocol facts follow the benchmark checkout listed in data/domain_facts.json.
% Main cohort only for comparisons; marked configurations are described as such.

The Coding domain evaluates a tested assistant that helps a simulated developer solve competitive programming problems from LiveCodeBench~\citep{jain2024livecodebench}.
The task and its native task grade are unchanged: the assistant's final submission is run against the hidden tests of the source problem.
What varies is the developer who continues the conversation after the shared first reply.

\subsection{Source and Task Panel}
\label{app:coding-panel}

\paragraph{Task panel.}
The panel contains 100 questions from the hard split of LiveCodeBench.
% src: data/tables_key_numbers.json domains.coding.tasks=100; data/domain_facts.json domains.coding.task_note
They were selected using the outcomes of earlier model runs on a larger question set: questions were ranked by whether saved runs showed a correctness difference between a neutral and a persona conversation that shared the same first reply, or a correct submission accompanied by an unmet expressed need.
The panel is therefore a case-study panel enriched for the mechanisms that the benchmark studies; it is neither a random sample nor a held-out test set, and its scores do not estimate performance on LiveCodeBench as a whole.
Only the question identifiers select source records, and the selection reasons are never shown to the tested assistant or to the simulated developer.

\paragraph{Roles and protocol.}
Each question is run once under six persona conditions and once under the neutral condition, which gives 700 planned conversations per model.
% src: data/tables_key_numbers.json domains.coding (persona_conditions=6, neutral_trials=1, episodes_per_model=700)
The public problem statement is the opening question, and the shared first reply is generated once per question and reused by all seven conditions.
The simulated developer then reads each reply and either sends a follow-up or stops; the opening counts as the first turn, and the conversation ends after at most five assistant turns.
% src: data/domain_facts.json domains.coding.turn_cap=5, turn_cap_unit
After the conversation ends, the runner sends a separate final-submission request, and only the reply to it is graded.
That reply must contain exactly one complete Python program between the lines \texttt{\#\#\# submission} and \texttt{\#\#\# end of submission}; missing or malformed markers fail the task, and code shown earlier in the conversation is never used as a fallback.
The tested assistant sees the problem, the conversation and the final-submission request and has no execution tools.
The simulated developer sees the problem, the conversation, the persona description, the recorded traits and the need texts.
Neither sees the hidden tests or the acceptance criteria; the needs judge sees the conversation and the frozen acceptance criteria, and it sees the final submission only for needs that concern properties of the delivered code.

\paragraph{Cohort.}
The main cohort in Coding comprises 14 models: the 12 models that belong to the main cohort in every domain, together with Grok~4.6 and Fable~5.1.
% src: data/coding_cells.csv main_cohort (14 True); data/models.csv n_main_cohort_domains; data/tables_key_numbers.json scorecard.main_n.coding
Claude Opus~5.5 used GPT-5.6 Sol at high effort for the supporting roles, and the five remaining GPT packages are registered as partial because many of their judge calls failed and were left missing (Appendix~\ref{app:cohort}).
% src: data/coding_cells.csv notes (captured judge failures left missing; registry status partial)

\subsection{Persona Bank and Needs}
\label{app:coding-personas}

\paragraph{Cards.}
The six cards are derived from records of the MatrAIx persona dataset~\citep{li2026matraix}, whose recorded traits include coding skill, preferred level of detail, comment style, dependency preferences, tone and trust (\tabref{tab:coding-personas}).
All six cards passed automated screening, and human selection is pending.
% src: output/panels/coding/persona.json (screening eligible; selection pending)

\paragraph{Needs and criticality.}
Each card carries six needs that the benchmark authors wrote as interpretations of its traits.
A need is labeled either persona-specific, such as type annotations, docstrings or an example walkthrough, or generic-quality, such as a rationale for a questioned correctness claim or public test cases; only persona-specific needs enter the persona-needs score, and generic-quality needs serve as diagnostics.
% src: output/panels/coding/persona.json (six needs per card; category persona_specific / generic_quality; screening eligible; selection pending)
Before any assistant answer, the acceptance requirements of every need are copied deterministically into a grading-criteria snapshot; no planner selects or rewrites needs, and every need of a card remains available on every question.
Coding assigns no criticality and computes no persona pass or joint pass.

\begin{table}[!tb]
% src: data/persona_effects.csv (domain=coding, main_cohort=True: task_value, needs_value, delta_vs_neutral_task, delta_ci_excludes_zero, paired_tasks); data/coding_needs.csv needs_expressed_rate; output/panels/coding/persona.json
\centering\footnotesize\setlength{\tabcolsep}{3pt}\renewcommand{\arraystretch}{1.15}
\begin{tabularx}{\linewidth}{@{}>{\raggedright\arraybackslash}p{3.3cm}>{\raggedright\arraybackslash}Xrrrrrr@{}}
\toprule
Condition & Persona-specific needs & Expr. & Needs & Pass & $\Delta$ & Below & Above \\
\midrule
Neutral & none & -- & -- & 87.1 & -- & -- & -- \\
495132: Detailed typed professional & detailed explanation; docstrings; modular structure; standard-library tools; type annotations & 81.5 & 96.4 & 77.9 & $-$10.3 & 7 & 0 \\
518717: Performance-focused student & custom implementation; detailed explanation; extensive comments; performance improvement; type annotations & 79.8 & 94.2 & 84.8 & $-$2.5 & 3 & 0 \\
690429: Deadline-driven technologist & code before explanation; custom implementation; docstrings; minimal test exposition; plain language; readability & 56.3 & 91.2 & 86.4 & $-$0.2 & 0 & 0 \\
809272: Examples-first minimalist & concise explanation; example walkthrough; no comments; straightforward structure & 57.8 & 91.2 & 89.0 & $+$1.6 & 0 & 0 \\
835253: Plain-language technologist & decision trade-offs; extensive comments; low complexity; minimal test exposition; plain language; supportive tone & 69.4 & 87.8 & 87.6 & $-$0.1 & 0 & 0 \\
992645: Examples-first learner & compact names; example walkthrough; object-oriented structure; plain language; supportive tone & 68.2 & 82.8 & 88.1 & $+$0.5 & 0 & 0 \\
\midrule
All personas pooled & & 67.0 & 91.3 & 85.6 & $-$1.9 & 2 & 0 \\
\bottomrule
\end{tabularx}
\captionsetup{position=bottom}
\caption{\textbf{Coding persona conditions in the main cohort.}
\emph{Persona-specific needs} lists the needs that enter the persona-needs score; generic-quality needs are omitted.
Numeric columns other than \emph{Below} and \emph{Above} are unweighted means of per-model values over the 14 main-cohort models, in percent except $\Delta$.
\emph{Expr.}: share of persona-specific needs expressed, among eligible persona conversations with a saved needs judgment.
\emph{Needs}: persona-needs score.
\emph{Pass}: native pass rate.
$\Delta$: paired persona-minus-neutral change in pass rate, in percentage points, over 48 to 99 questions per model.
\emph{Below}/\emph{Above}: number of models whose 95\% task-cluster bootstrap interval lies entirely below or above zero.
Pooled row: each model's persona conditions combined into one paired contrast.}
\label{tab:coding-personas}
\end{table}

\subsection{Native Task Grade, Persona-Needs Score and Simulator Audit}
\label{app:coding-grading}

\paragraph{Native task grade.}
The native task grade is the pass rate: confirmed passes of the hidden tests by the final submission, divided by all eligible conversations, including neutral ones.
A conversation is eligible when it completed, the simulator audit judged it valid, and it passed the analysis and integrity checks.
Every eligible conversation without a confirmed pass counts as a failure, including submission-format failures and unresolved evaluator outcomes.
% src: data/domain_facts.json domains.coding.task_metric, task_population; data/cells.csv task_population (domain=coding)
\tabref{tab:domain-coding} also reports the pass rate over all 700 planned conversations, with non-generated conversations counted as failures.
% src: data/coding_cells.csv task_value_all_planned, task_den_all_planned=700

\paragraph{Persona-needs score.}
The judge assesses each acceptance criterion of a need against what the developer publicly requested and derives the need's status from its expressed criteria: full credit if all are satisfied, no credit if all are unmet, and half credit otherwise.
The conversation score is the mean over expressed persona-specific needs, and a conversation has no score if no persona-specific need was expressed, if an expressed need remains unscored, or if a required judgment is missing.
The persona-needs score of a model is the mean over eligible persona conversations with a score.
% src: data/domain_facts.json domains.coding.needs_metric, needs_scope; data/cells.csv needs_population (domain=coding: "scoreable persona episodes among eligible (completed & simulator-valid) episodes")

\paragraph{Simulator audit.}
The audit returns valid, invalid or uncertain with quoted evidence.
Coding is the only domain in which the simulator audit filters the native task headline: invalid, uncertain and unaudited conversations leave the task population.
% src: data/domain_facts.json domains.*.audit_filters_headline (coding true; customer_service true, but only for needs: data/cells.csv task_population all_planned); data/cells.csv task_population (only coding filters on simulator validity)
Among audited conversations, the valid share in the main cohort ranged from 91.7\% for MiniMax~M3 to 99.1\% for Claude Sonnet~5.5.
% src: data/cells.csv sim_valid_rate (domain=coding, main_cohort=True): MiniMax M3 483/527, Claude Sonnet 5.5 693/699
Invalid verdicts did not concentrate in particular conditions: pooled over the main cohort, the invalid share was between 1.2\% and 3.6\% for every persona and 2.6\% for the neutral condition.
% src: data/coding_episodes.csv.gz sim_status by condition, main cohort pooled (invalid / audited)

\subsection{Per-Model Results}
\label{app:coding-results}

\input{tables/domain_coding}

\paragraph{Task.}
\tabref{tab:domain-coding} reports every model.
In the main cohort, the pass rate ranged from 67.6\% for MiniMax~M3 to 95.5\% for Fable~5.1, followed by Claude Sonnet~5.5 at 94.7\%.
% src: data/cells.csv task_value (domain=coding, main_cohort=True)
GLM~5.3 Flash and Qwen~3.8 Flash had high pass rates over their eligible conversations, 92.0\% and 91.2\%, but they generated only 443 and 364 of the 700 planned conversations; over all planned conversations, their pass rates were 58.1\% and 47.4\%.
% src: data/coding_cells.csv generated, task_value (GLM 5.3 Flash, Qwen 3.8 Flash)
% src: data/coding_cells.csv task_value_all_planned (GLM 5.3 Flash 0.581, Qwen 3.8 Flash 0.474)
The two lowest-scoring models also reached the turn cap most often: 378 MiniMax~M3 conversations and 314 Muse Glimmer 30B conversations stopped there, against 19 to 139 for each of the other main-cohort models.
% src: data/coding_cells.csv turn_cap_stops (main cohort)

\paragraph{Needs.}
Persona-needs scores ranged from 85.7\% for MiniMax~M3 to 95.2\% for Qwen~3.8 27B, but they rest on widely different numbers of conversations.
% src: data/cells.csv needs_value, needs_den (domain=coding, main_cohort=True)
Pooled over the main cohort, only 2,829 of the 6,958 eligible persona conversations have a needs score, mostly because a required needs judgment is missing in 4,111 of them.
% src: data/coding_needs.csv condition=persona_pooled, main cohort: scored_episodes=2829, eligible_episodes=6958, judgment_missing_episodes=4111
The Fable~5.1, Claude Haiku~5.5 and Claude Sonnet~5.5 packages recovered missing judgments through bounded corrective judgments and citation repairs recorded per conversation, so their needs scores rest on 585 to 590 conversations, against 19 to 190 for the other 11 main-cohort models.
% src: data/coding_cells.csv repaired_judges, needs_den (Fable 5.1 585, Claude Haiku 5.5 590, Claude Sonnet 5.5 586; others 19 to 190)
For the two Gemini models, the original validation rejected 540 and 525 needs judgments, which leaves 54 and 64 scored conversations; the raw-judge score update published in their packages would give 578 and 584.
% src: data/coding_cells.csv Gemini 3.7 / 3.8 Flash repaired_judges and notes
Across all 20 packages, the number of scored conversations ranges from 19 to 591, depending on how each package handled judge validation (Appendix~\ref{app:judge-policy}).
% src: data/cells.csv needs_den (domain=coding): min 19 (MiniMax M3, GPT-6 Astra), max 591 (Claude Opus 5.5)
Cross-model comparisons of the Coding needs score may therefore reflect judge-validation handling as well as assistant behavior, and we do not interpret Coding needs rankings.
For completeness, the rank correlation between pass rate and needs score across the main cohort was weak and not significant, $\rho=0.22$ ($n=14$, $p=0.46$).
% src: data/task_vs_needs.csv coding main_cohort spearman_rho=0.2176, spearman_p_perm=0.4618

\subsection{Persona Effects}
\label{app:coding-effects}

\paragraph{Direction and consistency.}
Pooled over the six personas, the persona-minus-neutral change in pass rate averaged $-1.9$ percentage points across the main cohort, and the interval excluded zero for two of the 14 models.
% src: data/persona_effects.csv coding persona_pooled main cohort (mean delta -0.0192; below 2, above 0)
Four personas had mean changes between $-0.2$ and $+1.6$ percentage points, and no model's interval excluded zero for them (\tabref{tab:coding-personas}).
% src: data/persona_effects.csv coding matraix_r690429, r809272, r835253, r992645 (main cohort)
The performance-focused student lowered the pass rate by 2.5 percentage points on average, with intervals below zero for three models.
% src: data/persona_effects.csv coding matraix_r518717 (mean -0.0255; below 3)
The detailed typed professional lowered it by 10.3 percentage points on average, with intervals below zero for seven of the 14 models; the largest decreases were 30.0, 26.9 and 20.0 percentage points for Grok~4.6, Qwen~3.8 Flash and Qwen~3.8 27B, respectively.
% src: data/persona_effects.csv coding matraix_r495132 (mean -0.1025; below 7; Grok 4.6 -0.300, Qwen 3.8 Flash -0.269, Qwen 3.8 27B -0.200)

\paragraph{Mechanism: a harness artifact.}
The two personas with mean decreases larger than one percentage point are the only two that ask for type annotations.
In the released final submissions of all 20 packages, all 242 submissions whose code contained the line \texttt{from \_\_future\_\_ import annotations} received a failing grade, 213 of them outside the Claude Opus~5.5 package and 191 in main-cohort cells; such submissions occurred only under these two personas and were most frequent under the detailed typed professional.
% src: benchmark repo output/results/coding/<model>/ final_code in data.jsonl.gz, evidence.jsonl.gz (Claude Haiku/Sonnet 5.5) and source/evidence.tar.gz (Claude Opus 5.5, 29 submissions; count as in appendix/cases.tex), joined by model_key and episode_id with data/coding_episodes.csv.gz task_outcome: 213 outside Opus, all fail; 191 in main-cohort cells (data/coding_cells.csv main_cohort), 179 of them eligible; only conditions matraix_r495132 and matraix_r518717 -- benchmark checkout, counts not in data/
The LiveCodeBench harness prepends a block of standard imports to every submitted program, and Python accepts a \texttt{\_\_future\_\_} import only at the beginning of a module, so such a submission fails before any test runs.
These failures therefore arise from an interaction between a requested code style and the evaluation harness, and the grade does not show whether the algorithms of the affected submissions are correct.
The released grade records do not separate this artifact from other failures, so the values in \tabref{tab:coding-personas} are unadjusted.
We reanalyzed the 179 such submissions in the eligible main-cohort population in two ways: dropping them with their neutral pairs changed the mean effects of the detailed typed professional and the performance-focused student to $+0.7$ and $+1.3$ percentage points, respectively, and counting them as passes changed both to $+1.8$.
% src: same join as above; paired persona-minus-neutral pass rate per main-cohort model over eligible episodes (reproduces data/persona_effects.csv when the submissions are kept as fails: -10.25, -2.55), mean over 14 models; dropped pairs: +0.73, +1.28; counted as pass: +1.85, +1.80 -- recomputed, not stored in data/
Because the dropped submissions had all failed, the first reanalysis conditions on the outcome; the effect after a regrade with the import moved lies between the unadjusted value and the all-pass value, and only such a regrade could locate it.
Without the detailed typed professional, the mean changes ranged from $-2.5$ to $+1.6$ percentage points, and we do not interpret its decrease as evidence that the assistants solved fewer problems for users who ask for typed code.
% src: data/persona_effects.csv coding (main-cohort mean delta per condition)

\paragraph{Needs by persona.}
Needs scores were lowest for the two novice personas that ask for plain language and a supportive tone, 87.8\% for the plain-language technologist and 82.8\% for the examples-first learner, and highest for the detailed typed professional, 96.4\%.
% src: data/persona_effects.csv coding needs_value, main-cohort mean per condition
These differences rest on the judged subset of conversations described in Appendix~\ref{app:coding-results}.

\subsection{Domain-Specific Failures and Caveats}
\label{app:coding-caveats}

\paragraph{Generation failures.}
Qwen~3.8 27B returned an empty or incomplete answer in 117 conversations; 112 of these were lost shared first replies on 16 questions, which removed all seven conditions of each question.
% src: data/failures.csv coding Qwen 3.8 27B empty_answer=117; data/coding_cells.csv notes (112 lost shared first replies on 16 tasks)
GLM~5.3 Flash and Qwen~3.8 Flash lost 250 and 329 conversations to failed requests after two resumptions at an unchanged 32,768-token cap.
% src: data/failures.csv coding tool_transport; data/coding_cells.csv notes and output_budget_tokens
MiniMax~M3 and Kimi~K3 had 24 and 15 model errors without a recorded reason.
% src: data/failures.csv coding other (MiniMax M3 24, Kimi K3 15)

\paragraph{Submission format.}
Claude Haiku~5.5 produced 99 final submissions that failed the required format, and Muse Glimmer 30B produced 74.
% src: data/coding_cells.csv submission_format_failures
For Muse Glimmer 30B, 55 of these had no markers at all and 18 began directly with a Python fence without the start marker.
% src: data/muse_tool_diagnosis.md section 6; data/coding_cells.csv notes (missing_submission_markers 55, missing_submission_start_marker 18)
Token accounting against the local serving logs shows that these replies are the model's complete answer-channel output, so the failures reflect the model's adherence to the format rather than content lost in serving.
The same model also had 18 empty outputs; for the 17 empty answers in the serving ledger, the turn ended inside the reasoning channel.
% src: data/muse_tool_diagnosis.md section 6 (17 ledger empty answers = reasoning + 4 tokens); data/failures.csv coding Muse Glimmer 30B empty_answer=18

\paragraph{Output budgets and judge policy.}
In a recorded recovery, Gemini~3.7 Flash, Gemini~3.8 Flash, Claude Haiku~5.5 and Claude Sonnet~5.5 reran failed generations with the output budget raised from 32,768 to 65,536 tokens (Appendix~\ref{app:judge-policy}).
% src: data/coding_cells.csv output_budget_tokens (Gemini: "32768, raised to 65536 for recovery (manifest.generation_recovery)"; Claude Haiku/Sonnet 5.5: "32768 tested ... 65536 tested only in bounded recovery")
For the Claude Haiku~5.5, Claude Sonnet~5.5 and Claude Opus~5.5 packages, the task grades come from an isolated LiveCodeBench run on the unchanged final submissions, because the original packages had no native grades; the five GPT packages were graded in the same way after capture.
% src: data/coding_cells.csv notes (native_supplement; native tests run post hoc on captured final submissions)
GPT-6 Astra lacks a simulator audit for 631 of its 700 completed conversations, so its pass rate of 100.0\% rests on 68 eligible conversations and is not comparable with the main cohort.
% src: data/coding_cells.csv GPT-6 Astra notes (631 lack audit), task_den=68

\paragraph{Self-judging.}
In the GPT-6 Luna cell, the tested model is also the developer simulator and every judge, which is a self-evaluation caveat for its needs score~\citep{panickssery2024selfpreference}.
