# Supplementary material for: PersonaChatBench: Evaluating Chat Assistants with Diverse Simulated Users
Source: arXiv:2610.42060 source file (2026-10-30)
Supplement: Supplementary file 8 [file finance.tex]

% Finance domain appendix. Every number is taken from data/ in this repository;
% protocol facts follow the benchmark checkout listed in data/domain_facts.json.
% Main cohort only for comparisons; marked configurations are described as such.

The Finance domain evaluates a tested assistant that acts as a financial advisor in conversations with a simulated client.
It turns single-turn questions from PRBench-Finance~\citep{akyurek2025prbench} into conversations while keeping the question and the expert rubric unchanged; the scores are a multi-turn adaptation of PRBench and are not official PRBench scores.
What varies is the client who follows up after the shared first reply.

\subsection{Source and Task Panel}
\label{app:finance-panel}

\paragraph{Task panel.}
The panel contains 97 questions from the finance hard split of PRBench, all single-turn and without attachments.
% src: data/tables_key_numbers.json domains.finance.tasks=97; data/domain_facts.json domains.finance.task_note
The questions were selected in three earlier rounds: a question was kept only if the rubric scores of different persona conditions differed substantially for both of two earlier tested assistants and the difference repeated under a per-question permutation test, and two further questions were removed because every persona obtained a near-perfect score.
The selection used the size of the spread, never which persona scored highest.
% src: finance-benchmark/README.md "How the 97 tasks were chosen"; finance-benchmark/examples/persona-trials/README.md (round 1 for both models; repeat test per task) -- benchmark checkout, not data/
The selection rounds tested GPT-5.6 Sol and GPT-6 Astra, which are also evaluated here, under a different simulator, different judges and an earlier needs specification; none of the runs reported here took part in the selection.
The panel is therefore a case-study panel on which persona effects are expected to be larger than on PRBench-Finance as a whole.

\paragraph{Task preparation.}
The original question is used verbatim as the opening message.
A private user-side part lists the facts that the client may disclose, an initial impression of the problem and the facts that the client does not know, which the client must answer with ``I do not know'' when asked; the expert rubric remains private to the task judge.

\paragraph{Roles and protocol.}
Each question is run once under 12 conditions, which gives 1,164 planned conversations per model: a neutral condition, six shared presets and five task-specific personas (D1--D5) designed for that question.
% src: data/tables_key_numbers.json domains.finance (persona_conditions=11, neutral_trials=1, episodes_per_model=1164); data/domain_facts.json domains.finance.condition_note
The assistant answers the opening once, and every condition of the question reuses this shared first reply.
The client then follows up in character or leaves, and the conversation ends after at most eight assistant turns, including the shared first reply.
% src: data/domain_facts.json domains.finance.turn_cap=8, turn_cap_unit
The tested assistant has no tools and never sees the persona card.

\paragraph{Cohort.}
The main cohort in Finance comprises 18 models: the 12 models that belong to the main cohort in every domain, Fable~5.1, and GPT-5.5, GPT-5.6 Sol, GPT-5.6 Terra, GPT-6 Astra and GPT-6 Sol, which have full dialogue packages in this domain.
% src: data/finance_cells.csv main_cohort (18 True); data/tables_key_numbers.json scorecard.main_n.finance
Grok~4.6 and Claude Opus~5.5 used GPT-5.6 Sol at high effort for the simulator and judges.
% src: data/finance_cells.csv support_sol_high (Grok 4.6, Claude Opus 5.5)

\subsection{Persona Bank and Needs}
\label{app:finance-personas}

\paragraph{Shared presets.}
Three communication presets ask for a style: the careful learner, the skeptical questioner and the concise pragmatist.
Three pressure presets press on the content of the advice without adding facts: the decisive pusher wants a single answer, the confident contrarian disagrees on instinct, and the reassurance seeker wants confirmation of a half-decided plan.
All six presets passed automated screening, and human selection is pending.
% src: output/panels/finance/persona.json (screening eligible, selection pending)

\paragraph{Task-specific personas.}
For every question, a model that sees the question but not the rubric writes five personas on a shared scheme of common and question-specific attributes, each set to a low, middle or high value; a deterministic check requires every pair of personas to differ substantially, with opposite extremes on some attributes.
The needs are not written by the model but follow from a fixed mapping of extreme attribute values to needs, for example from low domain familiarity to plain language or from high risk sensitivity to risks stated first.
Each task-specific persona carries two or three needs, of which the first two are critical; under the strict specification, one of them concerns content.

\paragraph{Needs and criticality.}
All runs reported here use the strict needs specification, not the earlier needs that the panel's shared persona file still lists; under it, each preset carries three needs, two of them critical: one about style and one about content (\tabref{tab:finance-personas}).
A content need asks whether the conclusion and the condition it depends on survive in the form the client requested; correctness belongs to the native task grade.
Each need has frozen criteria for satisfied, partially satisfied and not satisfied, and a scope that covers either every later reply or only replies that give the same kind of content again; length limits of about 150 words are measured by a program.
% src: finance-benchmark/data/need_criteria.json (max_words 150) -- benchmark checkout, not data/
Criticality is recorded in the preset definitions before any conversation, and the client states its needs in its own words.

\begin{table}[!tb]
% src: data/persona_effects.csv (domain=finance, main_cohort=True); data/finance_needs.csv (row_type=condition) needs_expressed_rate; data/finance_episodes.csv.gz assistant_turns (generated); finance-benchmark/data/presets_strict.json (critical needs)
\centering\footnotesize\setlength{\tabcolsep}{3pt}\renewcommand{\arraystretch}{1.15}
\begin{tabularx}{\linewidth}{@{}>{\raggedright\arraybackslash}p{3.3cm}>{\raggedright\arraybackslash}Xrrrrrrr@{}}
\toprule
Condition & Critical needs & Expr. & Needs & Turns & Rubric & $\Delta$ & Below & Above \\
\midrule
Neutral & none & -- & -- & 1.81 & 43.6 & -- & -- & -- \\
\addlinespace[2pt]
\multicolumn{9}{@{}l}{\emph{Communication presets}} \\
Careful learner & plain language; keeps the substance & 92.5 & 74.0 & 3.06 & 43.9 & $+$0.4 & 0 & 3 \\
Skeptical questioner & grounded reasoning; calibrated uncertainty & 96.1 & 81.5 & 3.96 & 44.8 & $+$1.6 & 0 & 4 \\
Concise pragmatist & focused response; essential caveats & 72.0 & 67.0 & 2.55 & 43.2 & $-$0.3 & 1 & 0 \\
\addlinespace[2pt]
\multicolumn{9}{@{}l}{\emph{Pressure presets}} \\
Decisive pusher & clear recommendation; essential caveats & 89.3 & 73.9 & 2.51 & 45.9 & $+$2.4 & 0 & 9 \\
Confident contrarian & responsive explanation; grounded reasoning & 95.8 & 78.8 & 4.21 & 46.2 & $+$2.6 & 0 & 8 \\
Reassurance seeker & focused response; essential caveats & 82.6 & 70.4 & 2.46 & 43.8 & $+$0.4 & 1 & 2 \\
\addlinespace[2pt]
\multicolumn{9}{@{}l}{\emph{Task-specific personas}} \\
D1 & varies by question & 59.6 & 70.3 & 2.75 & 44.2 & $+$0.7 & 0 & 2 \\
D2 & varies by question & 68.1 & 68.8 & 4.18 & 47.6 & $+$4.3 & 0 & 13 \\
D3 & varies by question & 60.9 & 70.5 & 3.36 & 47.1 & $+$3.6 & 0 & 12 \\
D4 & varies by question & 60.0 & 69.6 & 3.35 & 46.8 & $+$3.4 & 0 & 12 \\
D5 & varies by question & 57.0 & 68.8 & 3.60 & 46.6 & $+$3.2 & 0 & 11 \\
\midrule
Six presets pooled & & -- & 74.4 & -- & 44.6 & $+$1.2 & 0 & 5 \\
Task-specific pooled & & -- & 69.6 & -- & 46.5 & $+$3.0 & 0 & 13 \\
All personas pooled & & -- & 72.3 & -- & 45.4 & $+$2.0 & 0 & 11 \\
\bottomrule
\end{tabularx}
\captionsetup{position=bottom}
\caption{\textbf{Finance persona conditions in the main cohort.}
\emph{Critical needs} gives the two critical needs of each preset under the strict specification; the task-specific personas D1--D5 are written separately for each question, so their needs vary.
Numeric columns other than \emph{Below} and \emph{Above} are unweighted means of per-model values over the 18 main-cohort models.
\emph{Expr.}: share of pre-recorded needs expressed, in percent, among completed conversations whose simulator audit was not invalid.
\emph{Needs}: persona-needs score, in percent.
\emph{Turns}: mean assistant turns per generated conversation.
\emph{Rubric}: rubric percent.
$\Delta$: paired persona-minus-neutral change in rubric percent, in percentage points, over 65 to 97 questions per model.
\emph{Below}/\emph{Above}: number of models whose 95\% task-cluster bootstrap interval lies entirely below or above zero.
Pooled rows: each model's persona conditions in a group combined into one paired contrast.}
\label{tab:finance-personas}
\end{table}

\subsection{Native Task Grade, Persona-Needs Score and Simulator Audit}
\label{app:finance-grading}

\paragraph{Native task grade.}
Because PRBench rubrics were written for a single response, each rubric item was assigned, before any conversation, a rule for aggregating evidence across turns: most items earn credit if any assistant message supplies the content, some judge only the position held at the end, and penalty items count if the behavior occurs anywhere.
The judge grades every item once and must quote the conversation; judgments whose quotations are not exact substrings of the cited message fail validation and are excluded from the task mean.
The native task grade is rubric percent, the share of attainable rubric points earned, and the headline averages it over all recorded conversations of the 12 conditions, including the neutral condition, that have a valid advice grade.
% src: data/domain_facts.json domains.finance.task_metric, task_population; data/cells.csv task_population (domain=finance)
The advice pass in \tabref{tab:domain-finance} is not a PRBench measure: it uses a local threshold of 50\% of rubric points, which the Finance benchmark package declared in advance, and is computed over persona conditions only.
% src: tables/domain_finance.tex caption (advice pass: rubric percent >= 50, persona conditions only); data/verification.md addendum item 2; finance-benchmark/VALIDATION.md ("The 50% advice pass mark is our choice") and chatsim/arms.py ADVICE_PASS_PERCENT -- benchmark checkout

\paragraph{Persona-needs score.}
Each need earns 1, $\tfrac12$ or 0 against its frozen criteria, and every applicable reply after the need is voiced is judged, so a need met once and later abandoned is at most partially satisfied.
The conversation score is the mean over scoreable needs, and the persona-needs score of a model is the mean over persona conversations with at least one scoreable need, whatever their audit verdict.
The persona pass requires every critical need to be expressed, answered and satisfied, and the joint pass requires both the advice pass and the persona pass.
% src: data/domain_facts.json domains.finance.needs_metric, needs_scope; data/cells.csv needs_population (domain=finance)

\paragraph{Simulator audit.}
The audit returns valid, invalid or uncertain with quoted evidence and does not filter the headline; it counts a client as leaking the answer only when the client supplies the correct principle, figure, method or conclusion and the assistant adopts it.
% src: data/domain_facts.json domains.finance.audit, audit_filters_headline=false; finance-benchmark/prompts/simulator_audit_strict.md (answer_leak) -- benchmark checkout
Invalid verdicts concentrated in two presets: pooled over the main cohort, 21.9\% of audited careful-learner conversations and 10.1\% of audited concise-pragmatist conversations were invalid, against 0.7\% to 4.4\% for the other persona conditions and 1.5\% for the neutral condition.
% src: data/finance_episodes.csv.gz sim_audit_status by condition, main cohort pooled (careful_learner 376/1718, concise_pragmatist 173/1720, neutral 26/1721)

\subsection{Per-Model Results}
\label{app:finance-results}

\input{tables/domain_finance}

\paragraph{Task and needs.}
\tabref{tab:domain-finance} reports every model.
In the main cohort, rubric percent ranged from 35.4 for Muse Glimmer 30B to 57.1 for Fable~5.1, followed by Claude Sonnet~5.5 at 52.3.
% src: data/cells.csv task_value (domain=finance, main_cohort=True)
Persona-needs scores ranged from 55.4\% for MiniMax~M3 to 90.1\% for GPT-6 Luna, and the three GPT-6 models had the highest needs scores.
% src: data/cells.csv needs_value (domain=finance, main_cohort=True): GPT-6 Luna 0.901, GPT-6 Astra 0.900, GPT-6 Sol 0.888
Rubric percent and needs score showed no significant rank association across the main cohort, $\rho=0.13$ ($n=18$, $p=0.61$).
% src: data/task_vs_needs.csv finance main_cohort spearman_rho=0.1269, spearman_p_perm=0.6115
Joint pass rates were low for every model, from 3.9\% for Gemini~3.7 Flash to 32.9\% for GPT-6 Astra.
% src: data/cells.csv joint_pass_rate (domain=finance, main_cohort=True)

\paragraph{Reply length and the two grades.}
Across models, longer replies are associated with higher rubric scores and, more weakly, with lower persona pass rates.
The median length of the shared first reply ranged from 268 words for GPT-6 Sol to 749 words for MiniMax~M3.
% src: data/previews/mechanisms_values.csv (panel_domain=finance, x_words, main cohort)
It was correlated with rubric percent, $r=0.62$ ($n=18$, $p=0.006$), and negatively but not significantly with the persona pass rate, $r=-0.40$ ($n=18$, $p=0.10$).
% src: data/previews/mechanisms_stats.csv panels c and d, finance, main_cohort (pearson_r 0.6216, p_perm 0.0060; -0.3985, p_perm 0.0999)
This pattern is consistent with a rubric that rewards coverage of many points and therefore favors exhaustive answers, and with focus and plain-language needs that penalize them (\figref{fig:mechanisms}).
Conversation length shows the same split, from about two assistant turns per conversation for the GPT-6 models to more than 4.5 for the two Gemini models and MiniMax~M3.
% src: data/finance_cells.csv mean_assistant_turns_generated (GPT-6 Luna 2.12, GPT-6 Astra 1.96, GPT-6 Sol 2.14; Gemini 3.7 4.63, Gemini 3.8 4.54, MiniMax M3 4.57)
Across the 18 main-cohort models, the mean number of assistant turns per generated persona conversation was strongly negatively associated with the persona-needs score, $r=-0.93$ ($n=18$, $p<0.001$), and with the persona pass rate, $r=-0.91$ ($n=18$, $p<0.001$).
% src: data/previews/mechanisms_stats.csv supp, finance, persona_turns_mean vs needs_value (pearson_r=-0.9265, p_perm=0.0001) and vs y_persona_pass (pearson_r=-0.9097, p_perm=0.0001), main_cohort
The six OpenAI models had the six shortest persona conversations, 2.04 to 2.73 assistant turns, and held needs ranks 1 to 6, so the Finance needs ranking cannot be separated from conversation length and from the simulated client's decision to stop.
% src: data/finance_episodes.csv.gz assistant_turns (generated, condition != neutral), per-model mean, main cohort (GPT-6 Astra 2.04 to GPT-5.5 2.73; all other main-cohort models 2.88 to 4.80); data/cells.csv finance needs_rank_main_cohort (OpenAI models 1-6)

\subsection{Persona Effects}
\label{app:finance-effects}

\paragraph{Direction and consistency.}
In Finance, 10 of the 11 persona conditions raised the native task grade on average relative to the neutral condition, in contrast to Travel and Customer Service, where persona conditions mostly lowered it (\tabref{tab:finance-personas}).
% src: data/persona_effects.csv (main_cohort=True, condition_kind=persona) mean delta_vs_neutral_task: finance 10 of 11 positive (concise_pragmatist -0.29); travel 5 of 5 negative; customer_service 7 of 8 negative
Pooled over all 11 persona conditions, rubric percent rose by 2.0 percentage points relative to the neutral condition, and the interval lay above zero for 11 of the 18 models.
% src: data/persona_effects.csv finance pooled:all_personas, main cohort (mean +1.98; above 11)
The task-specific personas raised it more than the shared presets, by 3.0 against 1.2 percentage points, with intervals above zero for 13 and 5 models, respectively.
% src: data/persona_effects.csv finance pooled:designed (+2.98; above 13), pooled:shared_presets (+1.16; above 5)
Among the presets, the two pressure presets that challenge or press for a commitment had the largest gains, 2.6 percentage points for the confident contrarian and 2.4 for the decisive pusher.
% src: data/persona_effects.csv finance confident_contrarian (+2.63; above 8), decisive_pusher (+2.40; above 9)

\paragraph{Confound: conversation length.}
These gains cannot be separated from conversation length.
Neutral clients usually stopped after the shared first reply: pooled over the main cohort, 1,030 of 1,716 neutral conversations ended there, against 1,252 of 17,771 persona conversations.
% src: data/finance_cells.csv natural_one_reply_neutral_num/den and natural_one_reply_persona_num/den, summed over main cohort (60.0% and 7.0%)
Neutral conversations therefore averaged 1.81 assistant turns, against 2.46 to 4.21 for the persona conditions.
% src: data/finance_episodes.csv.gz assistant_turns (generated), main cohort, per-model condition means averaged over 18 models
Because most rubric items earn credit if the content appears in any assistant message, every additional message gives the assistant another opportunity to cover a rubric point.
Within each model, the conditions that lengthened the conversation most tended to have the largest rubric gains: the rank correlation over the 11 conditions was positive for all 18 models, with a mean of 0.51, which we report descriptively because each model's comparisons share the same neutral conversations.
% src: data/finance_episodes.csv.gz (turn difference vs neutral per model and condition) and data/persona_effects.csv delta_vs_neutral_task; Spearman over 11 conditions per model, 18 of 18 positive, mean 0.506
The positive Finance persona effects should therefore not be read as evidence that personas elicit better advice; they are consistent with an effect of longer conversations under a rubric that accumulates credit across turns, and the large gain of the decisive pusher despite short conversations suggests a second route through items judged on the final position.

\paragraph{Needs by persona.}
Among the presets, the concise pragmatist and the reassurance seeker, whose critical needs include a focused response, had the lowest needs scores, 67.0\% and 70.4\%, and the skeptical questioner the highest, 81.5\%.
% src: data/persona_effects.csv finance needs_value, main-cohort mean per condition

\subsection{Domain-Specific Failures and Caveats}
\label{app:finance-caveats}

\paragraph{Generation failures.}
For Qwen~3.8 Flash and GLM~5.3 Flash, every role, including the GPT-6 Luna simulator and judges, ran with a single 10,000-token cap, under which the shared first replies to 18 and 3 questions, respectively, were incomplete because reasoning exhausted the cap.
All 12 conditions of these questions failed, and a recovery at 32,768 tokens is reported separately and never pooled.
% src: data/finance_cells.csv notes (single MAX_OUTPUT_TOKENS knob; Qwen 3.8 Flash 18 of 97 tasks, 216 records; GLM 5.3 Flash 3 of 97 tasks, 36 records)
Muse Glimmer 30B had 170 terminal generation failures, which the failure table classifies as \status{other} and the run manifest records as API-error stops: 169 on the tested model and one on the simulator.
Of these conversations, 162 were graded on their recorded turns under the native rule.
% src: data/failures.csv finance Muse Glimmer 30B other=170; data/finance_cells.csv Muse Glimmer 30B notes (169 assistant ModelError, 1 user_simulator; 162 of 170 api_error conversations graded)
After an interruption, the two locally served models resumed under the benchmark's native resume rule, which regenerated every question without a completed summary, five for Qwen~3.8 27B and eight for Muse Glimmer 30B, and kept only the final attempt (Appendix~\ref{app:local-serving}).
% src: output/results/finance/{qwen-3-8-27b,muse-glimmer-30b}/*/manifest.json notes (regenerated tasks; native_resume) -- benchmark checkout, not data/
Two other packages also contain generation amendments.
The Claude Haiku~5.5 package regenerated two conversations in a generation-gap recovery.
In the Claude Opus~5.5 package, which is outside the main cohort, the shared first reply had been blocked for three questions; their 36 conditions were regenerated with up to 65,536 tokens, and 30 transport-failed conversations received a separately recorded bounded continuation, so its Finance results combine two output budgets.
% src: data/finance_cells.csv repaired_judges and regenerated_episodes (Claude Haiku 5.5: 2 episodes regenerated; Claude Opus 5.5: 3 blocked tasks / 36 conditions rerun at 65,536 tokens, 30 transport-failed episodes with bounded continuation) and notes (1,128 conditions at 12,288 tokens, 36 at 65,536: combined-budget panel); output/results/finance/claude-opus-5-5/*/source/README.md (PROTOCOL_AMENDMENT.json: failed shared replies) -- benchmark checkout

\paragraph{Judge policy.}
Advice judgments that failed evidence validation are excluded from the task mean: 196 for MiniMax~M3, whose task population falls to 965 conversations, and 95 and 68 for the two Gemini models.
% src: data/finance_cells.csv advice_validation_errors (MiniMax M3 196, Gemini 3.7 Flash 95, Gemini 3.8 Flash 68); task_den (MiniMax M3 965)
The Gemini packages publish a headline that bypasses the Python validation and word-count caps, whereas the values here use the original validated grades.
The Claude Haiku~5.5 and Claude Sonnet~5.5 packages contain a published citation repair of 28 and 40 graded conversations; Appendix~\ref{app:judge-policy} lists these and the other package-specific repairs.
% src: data/finance_cells.csv repaired_judges (Gemini 3.7 / 3.8 Flash raw-judge bypass; Claude Haiku 5.5 28, Claude Sonnet 5.5 40)

\paragraph{Self-judging.}
In the GPT-6 Luna cell, the tested model is also the client simulator and every judge, a self-evaluation caveat for its rubric grade and for its needs score, the highest in the main cohort~\citep{panickssery2024selfpreference}.
