# Supplementary material for: PersonaChatBench: Evaluating Chat Assistants with Diverse Simulated Users
Source: arXiv:2610.42060 source file (2026-10-30)
Supplement: Supplementary file 9 [file health.tex]

% Health domain appendix. Every number is taken from data/ in this repository;
% protocol facts follow the benchmark checkout listed in data/domain_facts.json.
% Main cohort only for comparisons; marked configurations are described as such.

The Health domain evaluates a tested assistant that acts as a doctor in medical consultations with a simulated user who plays a patient or caregiver.
It retains the cases and the native inquiry criteria of MedDialogRubrics~\citep{gong2026meddialogrubrics}.
What varies is how the simulated patient communicates after the shared first reply, the doctor's answer to the opening question that every condition of a case reuses.

\subsection{Source and Task Panel}
\label{app:health-panel}

\paragraph{Task panel.}
The panel contains 200 MedDialogRubrics cases with inquiry rubrics, and every tested model runs on the same cases.
% src: data/tables_key_numbers.json domains.health.tasks; data/domain_facts.json domains.health.task_note
It reuses the approved case plans and task policies of an earlier public export, whose approval records are automated evidence rather than human adjudication.

\paragraph{Task preparation.}
Before any dialogue, the preparation step behind these plans translated the opening, the case facts and the native criteria into English and separated the facts that a patient may disclose from evaluator-only references.
The same step retrieved or proposed a minimal shared background, such as the age of a patient or the relationship of a caregiver, which is recorded as synthetic and audited for compatibility, and it generated and reviewed a task policy that interprets the native criteria for a whole dialogue.
Symptoms, histories and examination results come only from the source case.

\paragraph{Roles and protocol.}
Each case is run once under five persona conditions, in which the simulated patient follows a private persona card, and once under a neutral condition without a card, which gives 1,200 planned conversations per model.
% src: data/tables_key_numbers.json domains.health (persona_conditions=5, neutral_trials=1, episodes_per_model=1200)
A conversation ends when the patient stops or after 20 doctor replies, including the shared first reply.
% src: data/domain_facts.json domains.health.turn_cap=20, turn_cap_unit
The cap was almost never binding: one of the 22,800 planned conversations in the 19 Health runs ended there, and the others ended with a patient stop or a failure.
% src: data/health_episodes.csv.gz ending_kind (doctor_turn_cap = 1 of 22,800 rows; 19 runs x 1,200)
The tested assistant sees only the public conversation and general consultation instructions.
The simulated patient sees the authorized case facts, the shared background, its persona card and its applicable needs, but never the hidden reference or the rubric; there are no tools.

\paragraph{Cohort.}
As in every domain, the main cohort contains the runs with the frozen panel, GPT-6 Luna at medium effort in every supporting role and full dialogue evidence (\secref{sec:cohorts}); in Health it comprises 12 models.
% src: data/health_cells.csv main_cohort (12 True); data/tables_key_numbers.json scorecard.main_n.health
Grok~4.6 and Claude Opus~5.5 used GPT-5.6 Sol at high effort for some or all supporting roles; GPT-5.5, GPT-5.6 Sol, GPT-5.6 Terra, GPT-6 Astra and GPT-6 Sol were delivered as score-only packages without transcripts; and Fable~5.1 has no Health run (Appendix~\ref{app:cohort}).
% src: data/health_cells.csv cohort_exclusion_reason (20 rows: 12 main cohort, 7 marked runs, Fable 5.1 without a run); data/models.csv main_cohort_health

\subsection{Persona Bank and Needs}
\label{app:health-personas}

\paragraph{Attributes and cards.}
The five persona cards combine binary values of five interaction attributes: medical familiarity, initial trust in the doctor, privacy concern, patience and information initiative (\tabref{tab:health-personas}).
The attributes describe communication behavior and do not change the case facts that the patient knows.
P4 and P5 form matched pairs with P3 and P2, respectively; each pair differs only in initial trust and carries the same needs.
The neutral condition is an ordinary cooperative patient with no assigned attributes and no private needs, not a sixth persona with intermediate values.
All five cards passed automated screening, and human selection is pending.
% src: output/panels/health/persona.json (screening eligible; selection pending)

\paragraph{Needs and criticality.}
Each card carries two needs, written as conditional requests so that a need can be scored only after the patient makes it public.
P1 asks for plain explanations of unfamiliar terms and for specific, manageable questions; P2 and P5 ask why a question or interpretation matters and how certain it is; P3 and P4 ask for the purpose of sensitive questions and for focused progress.
The applicability and criticality of each need are fixed per case in the approved plans before the shared first reply, and the needs judge cannot change them.
The conversation records contain a binary persona pass derived from the critical needs, but we do not report it for Health.
% src: output/panels/health/persona.json (two needs per card; screening eligible; selection pending); healthbench-benchmark/medsim/fixed5v3/runtime.py score_needs (persona_pass); data/cells.csv persona_pass_rate empty for health

\begin{table}[!tb]
% src: data/persona_effects.csv (domain=health, main_cohort=True: task_value, needs_value, delta_vs_neutral_task, delta_ci_excludes_zero, paired_tasks);
% src: data/health_needs.csv (level=condition, needs_expressed_rate); data/health_episodes.csv.gz (fact_acquisition, active_fact_acquisition, attribute_demonstration), per-model means then mean over models;
% src: output/panels/health/persona.json (dimensions, needs)
\centering\footnotesize\setlength{\tabcolsep}{3pt}\renewcommand{\arraystretch}{1.15}
\begin{tabularx}{\linewidth}{@{}>{\raggedright\arraybackslash}p{2.55cm}c>{\raggedright\arraybackslash}Xrrrrrrrrr@{}}
\toprule
Condition & Attributes & Needs & Expr. & Score & Facts & Asked & Demo. & Cov. & $\Delta$ & Below & Above \\
\midrule
Neutral & -- & none & -- & -- & 65.4 & 28.9 & -- & 39.9 & -- & -- & -- \\
P1: Receptive novice & L\,H\,L\,H\,L & plain language; concrete questions & 35.8 & 91.7 & 55.0 & 27.1 & 48.6 & 37.0 & $-$2.9 & 8 & 0 \\
P2: Informed questioner & H\,L\,L\,H\,H & explain rationale; state uncertainty & 70.7 & 92.3 & 70.0 & 28.4 & 67.3 & 42.1 & $+$2.2 & 0 & 6 \\
P3: Private, time-conscious novice & L\,H\,H\,L\,L & purpose of sensitive questions; focused progress & 27.2 & 75.4 & 54.2 & 26.4 & 30.7 & 36.0 & $-$3.8 & 12 & 0 \\
P4: Guarded, time-conscious novice & L\,L\,H\,L\,L & purpose of sensitive questions; focused progress & 31.0 & 74.5 & 55.1 & 26.5 & 16.1 & 36.7 & $-$3.2 & 11 & 0 \\
P5: Receptive, informed contributor & H\,H\,L\,H\,H & explain rationale; state uncertainty & 60.3 & 92.2 & 69.5 & 28.3 & 77.3 & 42.0 & $+$2.1 & 0 & 8 \\
\midrule
All personas pooled & & & -- & 86.5 & -- & -- & -- & 38.7 & $-$1.1 & 5 & 0 \\
\bottomrule
\end{tabularx}
\captionsetup{position=bottom}
\caption{\textbf{Health persona conditions in the main cohort.}
Attributes give low (L) or high (H) values of medical familiarity, initial trust, privacy concern, patience and information initiative, in that order.
Numeric columns other than \emph{Below} and \emph{Above} are unweighted means of per-model values over the 12 main-cohort models, in percent except $\Delta$.
\emph{Expr.}: share of applicable need items that the patient expressed.
\emph{Score}: persona-needs score.
\emph{Facts}: share of authorized case facts that became public.
\emph{Asked}: share of authorized facts elicited by a direct or broad doctor question.
\emph{Demo.}: share of attributes with an observation opportunity that the simulated patient demonstrated, from the advisory audit evidence.
\emph{Cov.}: inquiry coverage.
$\Delta$: paired persona-minus-neutral change in inquiry coverage, in percentage points, over 180 to 200 cases per model.
\emph{Below}/\emph{Above}: number of models whose 95\% task-cluster bootstrap interval lies entirely below or above zero.
Pooled row: each model's persona conditions combined into one paired contrast.}
\label{tab:health-personas}
\end{table}

\subsection{Native Task Grade, Persona-Needs Score and Simulator Audit}
\label{app:health-grading}

\paragraph{Native task grade.}
The native task grade is inquiry coverage: the share of applicable source inquiry criteria that a task judge finds fully met over the whole conversation, interpreted through the reviewed task policy.
The task policies distinguish criteria that require the doctor to ask, criteria that require only that the information be covered, and explicitly requested assessments.
Partly met criteria earn no credit in the headline and half credit in a separate diagnostic.
The headline population is every planned conversation with a task score, including neutral conversations and the graded partial dialogues of conversations in which a role failed; missing scores are not imputed.
% src: data/domain_facts.json domains.health.task_metric, task_population; data/cells.csv task_population (domain=health)
\tabref{tab:domain-health} also reports coverage over all 1,200 planned conversations with failures scored zero, and fact acquisition, the share of authorized case facts that became public, which excludes synthetic background and records the route by which each fact became public.
% src: tables/domain_health.tex caption (Fail=0 over 1,200 planned)

\paragraph{Persona-needs score.}
A need item earns 1, $\tfrac12$ or 0 when it is satisfied, partially satisfied or not satisfied, and it is scored only if the patient expressed it, the doctor had a later reply and the evidence is observable.
The conversation score is the mean over its scored items, and the persona-needs score of a model is the mean over persona conversations with at least one scored item; the neutral condition has no needs.
The expression rate and the response-opportunity rate are reported beside the score.
% src: data/domain_facts.json domains.health.needs_metric, needs_scope; data/cells.csv needs_population (domain=health)

\paragraph{Simulator audit.}
Health replaces the shared valid, invalid or uncertain verdict with an evidence-only simulator audit of the simulated patient.
For each attribute, the audit records whether there was an opportunity to show it and whether it was demonstrated, compatible but not demonstrated, contradicted or unobservable; it also records factual deviations and stopping evidence.
It assigns no conversation-level validity label and does not filter the headline.
In the main cohort, the patient simulator and all three judges are GPT-6 Luna at medium effort.
% src: data/domain_facts.json domains.health.audit, audit_filters_headline=false; data/health_cells.csv support_roles
P3 and P4, the personas with the largest coverage decreases, were also those whose simulated patients demonstrated their attributes least often, in 30.7\% and 16.1\% of opportunities, against 67.3\% and 77.3\% under P2 and P5 (\tabref{tab:health-personas}).
% src: data/health_episodes.csv.gz attribute_demonstration, main cohort, per-model condition means averaged over 12 models
Because the audit has no validity label, these conversations remain in every headline, and the P3 and P4 contrasts in Appendix~\ref{app:health-effects} compare simulated behaviors that only partly match their cards.

\subsection{Per-Model Results}
\label{app:health-results}

\input{tables/domain_health}

\paragraph{Task and needs.}
\tabref{tab:domain-health} reports every model together with the secondary Health metrics.
Among the 12 main-cohort models, inquiry coverage ranged from 27.0\% for GPT-6 Luna to 46.8\% for MiniMax~M3, with a mean of 38.9\%.
% src: data/cells.csv task_value (domain=health, main_cohort=True); data/tables_key_numbers.json scorecard.main_mean health.task=0.389
MiniMax~M3 generated 932 of its 1,200 planned conversations, so its headline rests partly on graded partial dialogues; with failures scored zero, its coverage is 44.5\%.
% src: data/health_cells.csv MiniMax M3 generated=932, task_den=1140, task_value_planned_failzero=0.4446; tables/domain_health.tex Fail=0 column
Among the main-cohort models that generated at least 80\% of their conversations, Muse Glimmer 30B had the highest coverage, 46.3\%.
% src: data/cells.csv Muse Glimmer 30B health task_value=0.4633, generated=1164
Persona-needs scores ranged from 77.4\% for Qwen~3.8 Flash to 96.5\% for GPT-6 Luna.
% src: data/cells.csv needs_value (domain=health, main_cohort=True)
GPT-6 Luna thus combined the highest needs score with the lowest coverage, and its patients expressed the fewest need items: 24.6\% of applicable items, against 39.7\% to 57.2\% for the other 11 models.
% src: tables/domain_health.tex Expr. column; data/health_cells.csv needs_items_expressed / needs_items_applicable
Across the main cohort, coverage and needs score were not significantly correlated, $\rho=-0.25$ ($n=12$, $p=0.45$).
% src: data/task_vs_needs.csv health main_cohort spearman_rho=-0.2517, spearman_p_perm=0.445

\paragraph{Questioning and coverage.}
Across models, coverage is associated with how many questions the doctor asks.
The mean number of questions in the shared first reply, counted as question marks, ranged from 2.28 for GPT-6 Luna to 7.98 for MiniMax~M3 and was correlated with coverage across the main cohort, $r=0.86$ ($n=12$, $p<0.001$).
% src: data/previews/mechanisms_values.csv (panel_domain=health, x_questions); data/previews/mechanisms_stats.csv panel a, health, main_cohort: pearson_r=0.8605, pearson_p_perm=0.0002
Part of this association is shared with reply length: after both variables were residualized on the median length of the first reply, the partial correlation was $r=0.52$ ($n=12$, $p=0.08$).
% src: data/previews/mechanisms_stats.csv supp, health, "x_questions | first_reply_words_median": pearson_r=0.5210, pearson_p_perm=0.0809
This pattern suggests that the Health headline measures the breadth of history-taking more than the quality of individual answers, which is consistent with Health ranking models differently from the other domains (\figref{fig:mechanisms}).

\subsection{Persona Effects}
\label{app:health-effects}

\paragraph{Direction and consistency.}
Three persona conditions lowered inquiry coverage relative to the neutral condition, and two raised it (\tabref{tab:health-personas}).
P3 lowered coverage by 3.8 percentage points on average, and the interval lay below zero for all 12 main-cohort models.
% src: data/persona_effects.csv health p3 main cohort: mean delta=-0.0384, below=12 of 12
P4 and P1 lowered it by 3.2 and 2.9 percentage points, respectively, with intervals below zero for 11 and 8 of the 12 models.
% src: data/persona_effects.csv health p4 (mean -0.0323, below 11), p1 (mean -0.0294, below 8)
P2 and P5 raised it by 2.2 and 2.1 percentage points, with intervals above zero for six and eight models, respectively.
% src: data/persona_effects.csv health p2 (mean +0.0216, above 6), p5 (mean +0.0210, above 8)
The matched pairs that differ only in initial trust produced similar changes.
This similarity does not show that initial trust is unimportant: the simulated patients demonstrated their attributes in only 30.7\% and 16.1\% of opportunities under P3 and P4 (Appendix~\ref{app:health-grading}), so the trust contrast may have been only partly realized, at least in the novice pair.
% src: data/health_episodes.csv.gz attribute_demonstration, main cohort, per-model condition means averaged over 12 models (p3 30.7, p4 16.1), as in tab:health-personas Demo. column; per-attribute demonstration rates are not in data/

\paragraph{Mechanism: disclosure.}
The two conditions that raised coverage are those with high information initiative, which also have high medical familiarity, and the three that lowered it have low values of both attributes.
Fact acquisition shows the same split: 70.0\% and 69.5\% of authorized facts became public under P2 and P5, 65.4\% under the neutral condition and 54.2\% to 55.1\% under P1, P3 and P4.
% src: data/health_episodes.csv.gz fact_acquisition, main cohort, per-model condition means averaged over 12 models
The share of facts elicited by a direct or broad doctor question stayed between 26.4\% and 28.9\% in every condition, so most of the difference comes from facts that became public without an eliciting question, which the audit records as volunteered or of uncertain route.
% src: data/health_episodes.csv.gz active_fact_acquisition (direct_or_broad_question_rate), same aggregation; routes: healthbench-benchmark/medsim/fixed5v3/prompting.py (shared_opening, direct_question, broad_question, spontaneous, uncertain, none)
Because some native criteria require only that the information be covered, a patient who volunteers facts can raise the doctor's coverage without any change in the doctor's questioning.
The paired contrast estimates the total effect of the user condition on the continuation, which comprises the patient's messages and stopping as well as the doctor's responses to them; disclosure is a pathway associated with this effect, and the data do not separate it from changes in how the doctor adapts.

\paragraph{Needs by persona.}
P3 and P4 had the lowest needs scores, 75.4\% and 74.5\%, against 91.7\% to 92.3\% for the other personas.
% src: data/persona_effects.csv health needs_value, main-cohort mean per condition
The focused-progress need accounts for this difference: pooled over the main cohort, it was expressed in 40.2\% of applicable items under P3 and 44.8\% under P4, and it earned 66.4\% and 64.3\% of the available credit, mostly through partial satisfaction.
% src: data/health_needs.csv level=need, main cohort, pooled: p3/focused_progress expressed 939/2337, credit (312+0.5*585)/910; p4/focused_progress expressed 1046/2337, credit (316+0.5*657)/1002
The need to explain sensitive questions was rarely expressed, in 13.9\% and 16.9\% of applicable items, and nearly always satisfied when it was.
% src: data/health_needs.csv level=need, main cohort, pooled: p3 326/2337, p4 396/2337; satisfied 294/310 and 362/383

\subsection{Domain-Specific Failures and Caveats}
\label{app:health-caveats}

\paragraph{Generation failures.}
Most Health generation failures with a recorded code are protocol failures, in which the doctor's reply did not match the structured object that the runner requires or, rarely, was not in English.
Claude Haiku~5.5 had 543 such failures and generated 657 of its 1,200 planned conversations.
% src: data/failures.csv health Claude Haiku 5.5 protocol_format=543, generated=657; data/health_cells.csv failure_codes (object_fields_mismatch, invalid_json_object_no_resample, actor_not_english)
A separate recovery of these conversations with a strict doctor schema reached 39.7\% coverage over all 543 and a needs score of 92.8\% over 299 of them; it is not pooled with the primary outcome.
% src: data/health_cells.csv Claude Haiku 5.5 notes (cap20 recovery task=0.3974 n=543, needs=0.9281 n=299)
Qwen~3.8 Flash had 182 such failures, Qwen~3.8 27B 129, GLM~5.3 Flash 78 and Claude Sonnet~5.5 69; the Claude Sonnet~5.5 failures were recovered in the same way and are likewise not pooled.
% src: data/failures.csv health protocol_format (Qwen 3.8 Flash 182, Qwen 3.8 27B 129, GLM 5.3 Flash 78, Claude Sonnet 5.5 69); data/health_cells.csv Claude Sonnet 5.5 notes (cap20 recovery n=69, not pooled)
MiniMax~M3 had 268 failures, 265 of them on the doctor role, and its package does not publish per-conversation failure codes.
% src: data/failures.csv health MiniMax M3 unknown=268; data/health_cells.csv notes (failed roles doctor 265)
Each locally served model also had eight conversations that were in flight during an unplanned server stop; the runner recorded them as interrupted and did not resample them.
% src: data/health_cells.csv failure_breakdown interrupted=8, failure_codes interrupted_inflight_no_resample=8 (Qwen 3.8 27B, Muse Glimmer 30B)

\paragraph{Output budgets and judge policy.}
The doctor output cap was the runner's default of 12,000 tokens for GLM~5.3 Flash and Qwen~3.8 Flash; for the two locally served models, the doctor requested 12,000 tokens and the local router enforced 65,536 (Appendix~\ref{app:local-serving}).
% src: data/health_cells.csv output_budget_tokens and notes ("doctor request 12000 / enforced 65536")
All main-cohort packages use the same judge-acceptance policy, \texttt{llm\_judgment\_v1}, which accepts any interpretable judge label without checking the cited evidence (Appendix~\ref{app:judge-policy}); for the two Gemini models, the raw-judge score update published in their packages gives the same headline values.
% src: data/health_cells.csv headline_judge_policy, notes; tables/domain_health.tex caption; data/health_episodes.csv.gz score_policy; healthbench-benchmark/medsim/fixed5v3/revision_runtime.py JUDGE_ACCEPTANCE_POLICY and tests/test_llm_judgment_acceptance.py -- benchmark checkout
The score-only GPT packages report the package headline under a stricter native acceptance policy and cannot be regraded, because they contain no item-level judgments.
% src: data/health_cells.csv notes (score-only report_row; native-strict acceptance)

\paragraph{Marked configurations.}
The Grok~4.6 and Claude Opus~5.5 packages judged a third, verification-related need for P1, P2 and P5, so their needs scores cover a different set of needs.
% src: data/health_cells.csv notes (extra judged needs verify_shared_information, verify_understanding)
In the Claude Opus~5.5 package, the simulator and judges differ by condition: GPT-6 Luna at medium effort for P3 and P4 and GPT-5.6 Sol at high effort for the other conditions; its persona-minus-neutral differences for P3 and P4 are therefore confounded with the simulator model.
% src: data/health_cells.csv Claude Opus 5.5 notes (mixed support roles per condition)

\paragraph{Self-judging.}
In the GPT-6 Luna cell, the tested model is also the patient simulator and every judge, so its needs score, the highest in the main cohort, carries a self-evaluation caveat~\citep{panickssery2024selfpreference}.
