# Supplementary material for: PersonaChatBench: Evaluating Chat Assistants with Diverse Simulated Users
Source: arXiv:2610.42060 source file (2026-10-30)
Supplement: Supplementary file 11 [file law.tex]

\label{app:law-redlining}

Contract redlining requires an assistant to translate a business stakeholder's instructions into legally and commercially appropriate document changes. A useful explanation does not necessarily produce a correct redline, while a technically correct document may leave the stakeholder's questions unresolved. PersonaRedline evaluates these outcomes separately: the tested assistant acts as a lawyer, and a simulated internal deal stakeholder holds the persona. We preserve the source contract and native task rubric while varying how the stakeholder seeks advice, expresses needs, and decides whether to continue the conversation.

\subsection{Source Tasks and Preparation}

We use 140 exact tasks from RedlineBench\footnote{ \url{https://huggingface.co/datasets/crosbylegal/RedlineBench}}. These tasks cover 101 input groups across three commercial scenarios. They include related negotiation branches and rubric variants, rather than 140 independent real-world transactions. The imported contracts, grounding documents, attorney references, and signed rubric weights remain unchanged.

Before generating the lawyer's first response, we freeze the task facts, represented side, permitted tools, initial question, persona cards, need criteria and criticality, and turn cap. A separate model-based review checks whether each task's five persona cards and associated needs are coherent, source-grounded, and appropriate for this current task.

\subsection{Persona Attributes and Needs}

Five authored archetypes are instantiated for each task, producing 700 task-specific persona cards. Each card contains 20 attributes: six background attributes, ten behavioral attributes, and four source-grounded task-priority attributes. Background attributes describe the stakeholder's role, contract familiarity, organizational context, and available review resources. The personas differ in how much they trust the lawyer, how they handle disagreement, and how much detail they want in an explanation. They also differ in how comfortable they are with uncertainty, how concerned they are about contract risks, and how much control they want over decisions. Other differences include how much background information they share, how willing they are to change their position, how they balance different business goals, and how they prefer to plan contract changes.

Within a task, the six background attributes and four task-priority attributes are identical across the five cards. The behavioral configuration varies, preserving the substantive task while changing the interaction. These profiles are synthetic archetypes, not a representative sample of real clients.

Each card has three candidate needs: two designated critical and one secondary. Table~\ref{tab:redline-personas} summarizes their communication focus. The exact task-specific criteria and criticality are recorded before the lawyer answers.

\begin{table}[htbp]
\appendixtablestyle
\caption{Redlining persona archetypes and associated need families, plus an additional neutral persona, resulting in a total of six personas. An asterisk marks a critical need.}
\label{tab:redline-personas}
\begin{tabularx}{\linewidth}{p{0.22\linewidth} X X}
\toprule
Persona & Interaction profile & Associated needs \\
\midrule
P1: Collaborative planner
& Organized and conditionally trusting; seeks a coherent decision plan.
& Prioritized recommendation*; explicit assumptions and unknowns*;
  reasons supported by contract provisions. \\
P2: Anxious delegator
& Concerned about adverse outcomes; relies on counsel for guidance.
& Clear counsel recommendation*; calibrated, plain-language risk
  explanation*; manageable immediate next steps. \\
P3: Guarded autonomous requester
& Skeptical and terse; limits context sharing and retains decision control.
& Explanation of why additional context matters*;
  document-grounded analysis*; preservation of stakeholder autonomy. \\
P4: Assertive authority seeker
& Blunt and attached to a position; expects precise support before revising it.
& Pinpoint contractual basis*; direct advice without unwarranted agreement*;
  primary position and approval-dependent fallback. \\
P5: Time-pressed decision maker
& Wants an actionable bottom line with little conversational overhead.
& Bottom-line recommendation first*; prioritized action or edit sequence*;
  compact supporting rationale. \\
\bottomrule
\end{tabularx}
\end{table}

Users can bring up several needs at once, explain a need over several messages, or stop without mentioning every need. The lawyer must still give accurate advice, use the supplied facts, and avoid assuming that a proposed term has been approved. These rules apply even when the user asks for a shorter, simpler, or more direct answer.

\subsection{Interaction Protocol and Role Visibility}

For each task, lawyer model, and trial, we use the same opening question for all six groups. We generate the lawyer's first reply once and reuse it unchanged for the five personas and the neutral user. The neutral user has no persona card or assigned persona needs. Each lawyer model generates its own shared opening for all personas.

The reported study uses a brief-opening instruction targeting 250 words for the first lawyer reply only, with accuracy taking priority. Note that this is an instruction to the lawyer model, not an exact threshold. Later replies and final documents have no length target. The maximum is eight complete stakeholder--lawyer exchanges, including the opening pair. Stakeholders may stop naturally earlier; there is no minimum length or forced disclosure requirement. A nonempty closing stakeholder message receives a lawyer reply before the conversation ends.

The lawyer receives the public task context, source contract, authorized grounding materials, public dialogue, and permitted editing tools. It does not receive the private persona card, need-grading criteria, hidden task rubric, attorney reference redline, or judge feedback. The simulator receives its persona, plain-language needs, authorized stakeholder facts, and the public conversation, but not hidden rubrics, reference answers, or evaluation feedback.

After the dialogue ends, a separate finalization step asks the same lawyer to produce a tracked-change Word document. A structured edit plan is applied through a document editor. Finalization is recorded separately and does not create another conversational response opportunity for persona-needs grading.

\subsection{Evaluation}

\paragraph{Native document performance.}
The document judge evaluates the saved redline against the rubric from the original RedlineBench. Let $w_i$ be the signed weight of rubric item $i$, and let $z_{ei}=1$ when episode $e$ receives a \texttt{PASS} verdict on that item. The normalized document score is
\begin{equation}
D_e =
\operatorname{clip}_{[0,1]}
\left(
\frac{
\sum_{i:w_i>0} w_i z_{ei}
-
\sum_{i:w_i<0} |w_i| z_{ei}
}{
\sum_{i:w_i>0} w_i
}
\right).
\label{eq:redline-document}
\end{equation}
A positive-weight \texttt{PASS} earns credit; a negative-weight \texttt{PASS} identifies a prohibited pattern and incurs a penalty. The source rubric defines no binary task-pass threshold, so we do not invent a task pass or joint pass.

We grade Word documents that pass the source benchmark's document checks, even if some requested edits are unfinished. We record editing errors separately; they do not automatically mean that the conversation failed or that the document cannot be graded. The editing tool cannot handle some Word features, including nested tracked changes and comment links. These are tool limitations, not temporary connection problems. Document scores therefore reflect both the lawyer's work and the editing tool, not just legal reasoning. Our study uses multi-turn conversations and one fixed judge model, so the scores might not be directly comparable to the official RedlineBench leaderboard scores.

\paragraph{Expressed persona needs.}
A need becomes scoreable only when its relevant scope is public and the lawyer subsequently has an opportunity to answer. The judge cites the relevant messages and scores the lawyer's latest answer or update to the user's request. Observable needs receive $1$ for satisfied, $0.5$ for partially satisfied, and $0$ for unmet. For the set $\mathcal{O}_e$ of scored needs,
\begin{equation}
S_e = \frac{1}{|\mathcal{O}_e|}
      \sum_{j\in\mathcal{O}_e} s_{ej}.
\label{eq:redline-needs}
\end{equation}

Undisclosed, inapplicable, unobservable, and no-response-opportunity needs are not included in this score. A request exclusively about future document work is not treated as an unanswered present-chat request. Conversely, promising future work does not satisfy an explanation requested now. Mixed requests are assessed only over their publicly expressed conversational scope. The final Word document cannot retrospectively add conversational need credit.

A separate frozen critical-needs indicator requires every applicable critical need to be expressed, answered, and fully satisfied. An answered partial or unmet critical need produces failure; unresolved critical evidence otherwise remains unknown. This indicator is distinct from the continuous satisfaction mean.

\paragraph{Simulator validity.}
A separate audit checks factual consistency, persona fidelity, information boundaries, and stopping behavior. Its validity judgment is not an assistant-performance score. All planned episodes remain in the evidence, including invalid simulations and missing judgments. Primary score means include only completed, simulator-valid episodes with a non-null saved score.

\subsection{Experimental Setup and Coverage}

The tested lawyers are GPT-5.6 Luna and GPT-6 Astra. GPT-5.6 Luna is fixed as the simulator and primary evaluator, with separate role contexts and low reasoning effort. The study uses one trial:
\[
140\ \text{tasks}
\times 2\ \text{lawyers}
\times (5\ \text{personas}+1\ \text{neutral})
= 1{,}680\ \text{episodes}.
\]
 Each lawyer therefore has 840 assigned episodes, including 700 persona episodes and 140 neutral episodes. All conversations are retained in the data, including those with invalid simulations, editing errors, low scores, or missing judgments.

Of all the 1,680 conversations completed, 1,633 were simulator-valid and 1,647 had saved document grades. Persona judgments were available for 1,385 of 1,400 assigned persona episodes. Among 1,362 completed, simulator-valid persona episodes, 1,114 had a non-null needs score. All conversations stopped naturally without reaching the eight round cap.

Table~\ref{tab:redline-results} reports conditional episode-level means on a 0--100 scale. Document means pool all six conditions; needs means include persona conditions only. We first calculate a score for each conversation, then average those scores. Each scored conversation counts equally, regardless of how many grading items its task has or how many needs the user expressed.

\begin{table}[htbp]
\appendixtablestyle
\caption{Completed redlining study. Parentheses give scored episodes over assigned episodes for each metric. The final column gives needs scoring coverage among completed, simulator-valid persona episodes. We report average scores for valid, graded conversations, not the percentage of conversations that passed. We report missing scores separately.}
\label{tab:redline-results}
\begin{tabularx}{\linewidth}{l X X X}
\toprule
Tested lawyer
& Document score
& Needs satisfaction
& Scoreable / eligible personas \\
\midrule
GPT-5.6 Luna
& 45.1 (796/840)
& 90.5 (544/700)
& 544/676 \\
GPT-6 Astra
& 47.5 (804/840)
& 96.8 (570/700)
& 570/686 \\
Combined
& 46.3 (1,600/1,680)
& 93.7 (1,114/1,400)
& 1,114/1,362 \\
\bottomrule
\end{tabularx}
\end{table}

A check of the saved conversation files found 33 missing document grades and 15 missing persona judgments. Missing grades are reported separately, not counted as zero, and do not mean that the conversations were unfinished. There were no recorded chat errors and 927 recorded editing errors. Documents could still be graded even when some edits failed.

\subsection{Results and Interpretation}

\paragraph{Expressed needs and document quality are distinct.}
The average expressed-needs scores are 90.5 for Luna and 96.8 for Astra, whereas their document scores are 45.1 and 47.5. These metrics measure different outcomes and use different sets of scored conversations. Meeting a user's expressed communication needs does not mean that the final contract will receive a high document score.

\paragraph{Results by persona.}
Table~\ref{tab:redline-persona-results} reports the scores for each persona and the neutral user. Each condition has 140 conversations per lawyer model. The averages include only valid conversations with an available score.

\begin{table}[htbp]
\appendixtablestyle
\caption{PersonaRedline scores on a 0--100 scale for each persona.}
\label{tab:redline-persona-results}
\begin{tabular}{@{}lrrrr@{}}
\toprule
& \multicolumn{2}{c}{Luna}
& \multicolumn{2}{c}{Astra} \\
Condition & Document & Needs & Document & Needs \\
\midrule
P1: Collaborative planner
& 45.0 (131) & 89.9 (116) & 47.6 (137) & 97.8 (121) \\
P2: Worried decision-maker
& 46.2 (134) & 91.9 (120) & 47.1 (135) & 97.6 (123) \\
P3: Skeptical, independent user
& 45.3 (133) & 91.8 (108) & 47.6 (132) & 97.8 (124) \\
P4: Assertive user
& 46.3 (135) & 87.7 (121) & 46.8 (136) & 96.0 (128) \\
P5: Trusting, time-pressed user
& 44.3 (131) & 91.5 (79) & 47.5 (133) & 93.5 (74) \\
Neutral
& 43.7 (132) & --- & 48.2 (131) & --- \\
\bottomrule
\end{tabular}
\end{table}

\paragraph{Which needs were easier to meet?}
Luna's highest needs scores occur for P2 and P3. Astra scores similarly highly for P1, P2, and P3, with averages of 97.6--97.8. These personas ask for clear recommendations, supporting reasons, or explanations of what remains unknown. Such requests may help the lawyer focus on a specific concern.

P4 has lower needs scores than P1--P3 for both models. This persona asks for exact contract support, a direct assessment of a proposed position, and a defensible fallback. Meeting these requests may require more precise answers than giving a general recommendation. P5 combines a preference for short answers with requests for priorities and compact contract references. This combination may help explain Astra's lower P5 score. These are possible explanations, not demonstrated causes of the differences.

\paragraph{No persona consistently produces the best document.}
Among the five personas, document averages range from 44.3 to 46.3 for Luna and from 46.8 to 47.6 for Astra. P4 has Luna's highest document average, despite having its lowest needs average. For Astra, the neutral condition has the highest document average. There is therefore no consistent pattern in which one persona produces the best documents across both models. Different sets of valid, graded tasks and editing-tool limitations may also affect these comparisons.

A selected illustration is task \texttt{redline-s1-t4-g01a}, Luna, P4. The simulator-valid conversation received full credit on all three expressed needs, including contract-grounded advice and an approval-dependent fallback. Its complete Word document nevertheless received a document score of zero: the saved native judge found required source-task changes omitted or incorrect. This example illustrates the separation between conversational accommodation and document performance.

\paragraph{Scope of the conclusions.}
High needs scores do not mean that every private need was expressed or met. The personas also ask for different things, so their needs scores do not measure an identical set of requests. The authored archetypes, related source-task branches, single trial, and single primary judge configuration limit claims about real-client behavior, reproducibility, and model ranking. These descriptive differences do not establish that a persona caused a higher or lower score. Distinguishing requests for advice now from requests for later document changes also needs further analysis.
