# Supplementary material for: PersonaChatBench: Evaluating Chat Assistants with Diverse Simulated Users
Source: arXiv:2610.42060 source file (2026-10-30)
Supplement: Supplementary file 12 [file math.tex]

% Math domain appendix. Every number is taken from data/ in this repository;
% protocol facts follow the benchmark checkout listed in data/domain_facts.json.
% Main cohort only for comparisons; marked configurations are described as such.

The Math domain evaluates a tested assistant that acts as a tutor in conversations with a simulated student about a mathematics problem.
The native task is to reach a correct and well-supported solution, and the native task grade is the correctness of the solution that the tutor gives or explicitly endorses at the end of the conversation.
What varies is the student: six learner profiles that differ in how they want explanations and help, and a neutral student, all with the same mathematical starting knowledge for a given problem.

\subsection{Source and Task Panel}
\label{app:math-panel}

\paragraph{Task panel.}
The panel contains 205 problems from three sources: 37 school-level competition problems from the tutoring component of SimulatorArena~\citep{dou2025simulatorarena}, which are drawn from MATH~\citep{hendrycks2021math}; 139 short-answer competition problems from HARP~\citep{yue2024harp}; and 29 olympiad proof problems from IMO-ProofBench~\citep{luong2025imoproofbench}.
% src: data/tables_key_numbers.json domains.math.tasks=205, tasks_by_kind (arena 37, harp 139, imo 29); data/domain_facts.json domains.math.sources
The three sources form Easy, Medium and Hard tiers that describe relative difficulty within this panel.
The problems were selected from development conversations for simulation stability, observable persona behavior and interpretable grading, without using task grades or need scores; the panel is therefore a development set rather than an independent held-out test set.

\paragraph{Roles and protocol.}
Each problem is run once under six persona conditions and once under the neutral condition, which gives 1,435 planned conversations per model.
% src: data/tables_key_numbers.json domains.math (persona_conditions=6, neutral_trials=1, episodes_per_model=1435)
Within a problem, every condition shares a reviewed description of the student's mathematical knowledge and initial difficulty, so learners with different preferences start from the same preparation.
Math departs from the shared protocol in one respect that matters for the comparisons below: the student opens the conversation in character, and the opening and the tutor's first reply are generated separately for every condition, so Math has no shared first reply.
A conversation ends naturally or after 25 tutor replies; near the cap the tutor may consolidate the remaining explanation, and the student has one final attempt after it.
% src: data/domain_facts.json domains.math.turn_cap=25, turn_cap_unit
The cap was rarely reached: 14 of the 21,525 main-cohort conversations stopped at it.
% src: data/math_episodes.csv.gz stop_reason=max_turns (14 of 21,525 main-cohort rows)
A completed conversation requires the student to state a conclusion and the tutor to confirm it; whether the conclusion is correct is graded separately.
The tutor sees only the problem and the public conversation, and the student sees its learner view and its persona; reference solutions and rubrics are used only by the judges, and there are no tools.

\paragraph{Cohort.}
The main cohort in Math comprises 15 models: the 12 models that belong to the main cohort in every domain, together with Grok~4.6, Fable~5.1 and Claude Opus~5.5.
% src: data/math_cells.csv main_cohort (15 True); data/tables_key_numbers.json scorecard.main_n.math
The five remaining GPT packages contain item-level judgments but no transcripts, and their judges ran at high effort while the student simulator's effort is unrecorded.
Their task identifiers match the frozen panel, but their task hashes differ from it, so an exact panel match cannot be verified; these packages are therefore reported separately (Appendix~\ref{app:cohort}).
% src: data/math_cells.csv notes (deliver3 package; panel_match unverified, task hashes differ from frozen panel; panel_identity_match=True; judges GPT-6 Luna high, student effort unrecorded)

\subsection{Persona Bank and Needs}
\label{app:math-personas}

\paragraph{Attributes and cards.}
The persona vocabulary has nine attributes adapted from MatrAIx~\citep{li2026matraix}, with local additions for the order of presentation, the preferred kind of help and the clarification of the problem statement.
The attributes are explanation detail, presentation order, tone, terminology, reasoning style, help preference, initial emotion, specific concerns and problem clarification.
Six fixed cards combine four to six of these attributes into learner types (\tabref{tab:math-personas}); unselected attributes are omitted rather than set to a middle value.
The neutral student uses the same problem, starting knowledge and protocol without any assigned attribute.
All six cards passed automated screening, and human selection is pending.
% src: output/panels/math/persona.json (dimensions, needs, screening eligible, selection pending); data/persona_labels.csv (P1-P6 labels)

\paragraph{Needs and criticality.}
Each selected attribute is paired with one need and with satisfied, partially satisfied and not satisfied anchors that are fixed before generation.
Help preference concerns who performs the current step: a hint leaves the move to the learner, whereas a demonstration performs it.
Problem clarification concerns the objects, conditions and quantifiers of the original problem, and terminology support concerns unfamiliar mathematical language.
Emotional responsiveness applies only when the student shows anxiety or discouragement that affects participation.
A persistent preference applies to all later relevant teaching, whereas a local request applies only to its object.
Math assigns no criticality and computes no persona pass.

\begin{table}[!tb]
% src: data/persona_effects.csv (domain=math, main_cohort=True); data/math_needs.csv needs_expressed_rate (disclosed / known_disclosure); output/panels/math/persona.json; data/persona_labels.csv
\centering\footnotesize\setlength{\tabcolsep}{3pt}\renewcommand{\arraystretch}{1.15}
\begin{tabularx}{\linewidth}{@{}>{\raggedright\arraybackslash}p{3.6cm}>{\raggedright\arraybackslash}Xrrrrrr@{}}
\toprule
Condition & Needs & Expr. & Score & Correct & $\Delta$ & Below & Above \\
\midrule
Neutral & none & -- & -- & 91.2 & -- & -- & -- \\
P1: Concise independent learner & compact detail; principles first; direct tone; logical reasoning; hints before trying & 57.7 & 82.0 & 91.6 & $+$0.6 & 1 & 0 \\
P2: Detail-oriented checker & full detail; principles first; explained terms; demonstration before trying; specific concerns & 64.7 & 85.3 & 92.8 & $+$1.7 & 0 & 1 \\
P3: Example-led explorer & examples first; supportive tone; explained terms; hints before trying; problem clarification & 62.6 & 80.3 & 91.4 & $+$0.3 & 0 & 1 \\
P4: Intuitive demonstration seeker & examples first; direct tone; intuitive reasoning; demonstration before trying & 76.8 & 81.3 & 91.2 & $+$0.1 & 1 & 0 \\
P5: Anxious starter & compact detail; supportive tone; explained terms; demonstration before trying; emotional responsiveness; problem clarification & 46.9 & 81.4 & 90.6 & $-$0.6 & 0 & 0 \\
P6: Frustrated learner & full detail; direct tone; intuitive reasoning; hints before trying; emotional responsiveness & 75.2 & 80.8 & 91.9 & $+$0.7 & 0 & 0 \\
\bottomrule
\end{tabularx}
\captionsetup{position=bottom}
\caption{\textbf{Math persona conditions in the main cohort.}
\emph{Needs} lists the needs derived from each card's attributes.
Numeric columns other than \emph{Below} and \emph{Above} are unweighted means of per-model values over the 15 main-cohort models, in percent except $\Delta$.
\emph{Expr.}: share of applicable needs that the student expressed.
\emph{Score}: persona-needs score.
\emph{Correct}: tutor correctness over the condition's conversations with a tutor grade.
$\Delta$: persona-minus-neutral change in tutor correctness, in percentage points, paired by problem over 114 to 205 problems per model; because openings and first replies are generated per condition in Math, $\Delta$ includes the effect of the opening.
\emph{Below}/\emph{Above}: number of models whose 95\% task-cluster bootstrap interval lies entirely below or above zero.}
\label{tab:math-personas}
\end{table}

\subsection{Native Task Grade, Persona-Needs Score and Simulator Audit}
\label{app:math-grading}

\paragraph{Native task grade.}
The native task grade is 1 when the tutor's final or explicitly endorsed solution satisfies the problem and is supported by a valid mathematical argument, and 0 otherwise.
The judge reads the complete dialogue with the source references and accepts equivalent answers and alternative proofs.
Errors made along the way are recorded separately, and a strict variant requires the solution to be correct and free of errors.
For short-answer problems, the student's final answer is also graded as a separate learner outcome.
The headline population is the persona conversations with a tutor grade, pooled over the three sources with equal weight per graded conversation; neutral conversations are reported separately, and ungraded or failed conversations are excluded.
% src: data/domain_facts.json domains.math.task_metric, task_population; data/cells.csv task_population (domain=math)

\paragraph{Persona-needs score.}
A needs judge reads the whole public dialogue, the frozen needs and their anchors, and the specific checks of the mathematics judge, but not the task grade or the audit result.
It scores each need that the student expressed and the tutor had an opportunity to answer with 1, $\tfrac12$ or 0.
The conversation score is the mean over scored needs, and the persona-needs score of a model is the mean over persona conversations with at least one scored need; conversations in which a citation failed validation keep their other scored needs.
% src: data/domain_facts.json domains.math.needs_metric; data/cells.csv needs_population (domain=math)

\paragraph{Simulator audit.}
The audit checks the student's persona, knowledge boundaries, problem facts and ending, and it returns valid or invalid.
A student who, uninvited, develops the key route through the main difficulty and completes the remaining derivation alone is judged to have taken over the teaching, which is invalid.
The audit does not filter the headline.
% src: data/domain_facts.json domains.math.audit, audit_filters_headline=false
In the main cohort, the valid share ranged from 97.0\% for MiniMax~M3 to 99.9\% for DeepSeek~V4.1 Flash, and the invalid share was between 0.4\% and 0.9\% in every condition.
% src: data/cells.csv sim_valid_rate (domain=math, main_cohort=True); data/math_episodes.csv.gz sim_status by condition, main cohort pooled

\subsection{Per-Model Results}
\label{app:math-results}

\input{tables/domain_math}

\paragraph{Task.}
\tabref{tab:domain-math} reports every model, with the headline split by source.
In the main cohort, tutor correctness ranged from 80.8\% for MiniMax~M3 to 97.7\% for Qwen~3.8 Flash.
% src: data/cells.csv task_value (domain=math, main_cohort=True)
The value for Qwen~3.8 Flash, and to a lesser degree that for GLM~5.3 Flash, rests on a population without most IMO-ProofBench conversations.
Both models ran with a 10,000-token tutor cap and lost 443 and 284 conversations to truncation, so only 26 and 35 of their IMO-ProofBench persona conversations were graded, against 101 to 174 for the other main-cohort models.
% src: data/failures.csv math truncated (Qwen 3.8 Flash 443, GLM 5.3 Flash 284); data/math_cells.csv output_budget_tokens, task_den_imo
Counting every planned persona conversation without a grade as incorrect, their correctness was 65.5\% and 75.2\%.
% src: data/math_cells.csv task_value_all_planned_lb (Qwen 3.8 Flash 0.655, GLM 5.3 Flash 0.752)
Among the models with most of their conversations graded, Claude Opus~5.5 and Fable~5.1 had the highest correctness, 97.4\% and 96.4\%.
% src: data/cells.csv task_value (Claude Opus 5.5 0.974, Fable 5.1 0.964)
The sources differ in how much they separate models: correctness on SimulatorArena problems was between 97.7\% and 100.0\% for every main-cohort model, whereas on IMO-ProofBench it ranged from 36.8\% for Muse Glimmer 30B to 93.6\% for Claude Opus~5.5 among the models with at least 100 graded conversations.
% src: data/math_cells.csv task_num/den_arena and task_num/den_imo (main cohort)
The strict, error-free rate separates models further: it ranged from 22.6\% for MiniMax~M3 to 87.3\% for Qwen~3.8 Flash, whose rate rests on the reduced population described above, and Muse Glimmer 30B had the second-lowest rate, 40.4\%.
% src: tables/domain_math.tex Strict column (main cohort)

\paragraph{Needs.}
Persona-needs scores ranged from 58.0\% for Muse Glimmer 30B to 90.5\% for Claude Opus~5.5.
% src: data/cells.csv needs_value (domain=math, main_cohort=True)
Math is one of the domains in which task and needs scores are positively associated across models: the rank correlation between tutor correctness and needs score was $\rho=0.56$ ($n=15$, $p=0.032$).
% src: data/task_vs_needs.csv math main_cohort spearman_rho=0.5607, spearman_p_perm=0.0319
Pooled over the main cohort, the needs with the lowest credit were help preference and explanation detail, which earned 79.7\% and 79.8\% of the available credit; both require the tutor to judge how much of the reasoning to supply and which step to leave to the learner.
% src: data/math_needs_by_need.csv main cohort pooled: pref_help_agency (16,540 scored), pref_detail_brief_vs_full (8,106 scored), credit=(satisfied+0.5*partial)/scored
Emotional responsiveness and problem clarification earned 95.7\% and 94.8\%, but problem clarification was scored for only 6.4\% of the applicable items, mostly because students rarely expressed it.
% src: data/math_needs_by_need.csv main cohort pooled: emotional_responsiveness, problem_statement_clarification (scored 375 of 5,873 applicable; not_disclosed 5,458)

\subsection{Persona Effects}
\label{app:math-effects}

\paragraph{Direction and consistency.}
Persona effects on tutor correctness were small (\tabref{tab:math-personas}).
The mean persona-minus-neutral change ranged from $-0.6$ to $+1.7$ percentage points across the six conditions, and for each condition at most one of the 15 models had an interval that excluded zero.
% src: data/persona_effects.csv math main cohort (mean delta per condition; below/above counts)
Only the detail-oriented checker shifted correctness in the same direction for most models: its change was positive for 13 of the 15 models, and the 95\% $t$-interval of the mean across models, $+0.6$ to $+2.7$ percentage points, lay above zero (\figref{fig:persona}); as for every Math condition, this change includes the effects of the persona-written opening and of an independently generated first reply.
% src: data/previews/persona_effects_values.csv math-p02 (mean 1.652, ci_lo 0.595, ci_hi 2.710, n_models_above 13 of 15)
Pooled over all six personas, the per-model change ranged from $-1.6$ to $+3.5$ percentage points, and only the interval of Claude Opus~5.5 excluded zero, lying below it.
% src: data/math_cells.csv delta_persona_vs_neutral_task, delta_ci_low, delta_ci_high (main cohort; Claude Opus 5.5 -0.016 [-0.029, -0.004])
Tutor correctness depends on the mathematical content of the final solution rather than on a commitment or an ending that the user controls, and the small effects are consistent with the observation that persona effects on native grades concentrate in domains where the grade depends on what the user leaves with.

\paragraph{Pairing.}
Because the Math pairs share the problem and the student's starting knowledge but not the opening or the tutor's first reply, the paired differences include both the effect of a persona-conditioned opening and the variation of an independently generated first reply, and they cannot be attributed to the later conversation alone.

\paragraph{Needs by persona.}
The anxious starter expressed the smallest share of its needs, 46.9\%, and the intuitive demonstration seeker the largest, 76.8\%.
% src: data/math_needs.csv needs_expressed_rate, main-cohort mean per condition
Needs scores varied little across personas, from 80.3\% to 85.3\%, with the detail-oriented checker highest.
% src: data/persona_effects.csv math needs_value, main-cohort mean per condition

\subsection{Domain-Specific Failures and Caveats}
\label{app:math-caveats}

\paragraph{Generation failures.}
For GLM~5.3 Flash and Qwen~3.8 Flash, the primary pass used a 10,000-token tutor cap, which long reasoning exhausted, with the highest failure rate on proof problems.
% src: data/math_cells.csv output_budget_tokens=10000 and notes (primary pass, teacher cap 10000); data/math_episodes.csv.gz failure_kind by dataset (IMO 159/203 and 169/203 failed vs HARP 121/973 and 276/973)
A separate recovery at a 32,768-token cap reran 175 and 231 of the failed conversations and completed 64 and 133 of them; it is reported separately and never pooled with the primary outcome.
% src: data/math_cells.csv recovery_cap32k_records, recovery_cap32k_completed (GLM 5.3 Flash 175/64, Qwen 3.8 Flash 231/133); notes
Qwen~3.8 27B returned an empty answer in 94 conversations.
% src: data/failures.csv math Qwen 3.8 27B empty_answer=94
For the two locally served models, tutor calls interrupted by an unplanned server stop were resent once through the benchmark's native recovery script under the recorded recovery plan r1, and the original attempts are retained (Appendix~\ref{app:local-serving}).
% src: output/results/math/{qwen-3-8-27b,muse-glimmer-30b}/*/manifest.json notes ("Recovery r1 resent the ... teacher calls per model interrupted by the driver-upgrade stop, using the native scripts/recover_run.py") and recovery.transport_recovery
Grok~4.6, Kimi~K3, MiniMax~M3 and DeepSeek~V4.1 Flash each had between 30 and 41 failures without a recorded reason.
% src: data/failures.csv math other (Grok 4.6 37, Kimi K3 32, MiniMax M3 41, DeepSeek V4.1 Flash 30)

\paragraph{Judge policy.}
For the two Gemini models, 14 evaluations each failed under the original validated grading and remain missing in the headline; the raw-judge score update in their packages scores them, with the values given in the caption of \tabref{tab:domain-math}.
% src: data/failures.csv math Gemini 3.7 / 3.8 Flash (protocol_format 9, tool_transport 5); tables/domain_math.tex caption
The needs score of Muse Glimmer 30B includes eight conversations whose needs judgment was only partially validated but carries a score, as in its package headline.
% src: data/verification.md reproduction notes (Math, Muse Glimmer 30B: 8 partial_validation episodes)
The Claude Haiku~5.5 and Claude Sonnet~5.5 packages recovered grading and transport gaps by replaying accepted calls and by bounded retries, without citation repair.
% src: data/math_cells.csv notes (legacy_evidence packages)

\paragraph{Self-judging.}
In the GPT-6 Luna cell, the tested tutor is also the student simulator and every judge, which is a self-evaluation caveat for both its tutor-correctness grade and its needs score~\citep{panickssery2024selfpreference}.
