# Supplementary material for: PersonaChatBench: Evaluating Chat Assistants with Diverse Simulated Users
Source: arXiv:2610.42060 source file (2026-10-30)
Supplement: Supplementary file 13 [file protocol.tex]

% Appendix A: shared protocol details.
% Source of protocol text: the benchmark repository's standard/README.md,
% standard/prompts/*.md and standard/personas/README.md at commit 4cbf5c4e.

This appendix specifies the parts of the shared protocol that all six domains apply: the need statuses and the scoring rules built on them, the four prompt contracts, the persona card format, and the record that each run publishes. Domain-specific additions, such as tools, safety rules and output schemas, are described in Appendices~\ref{app:health}--\ref{app:travel}.

\subsection{Need Statuses, Persona Pass and Evidence Validation}
\label{app:statuses}

The needs judge assigns each pre-recorded need one of the seven statuses in \tabref{tab:statuses}. Only three statuses carry credit, and all three require that the user expressed the need in a public message and that the tested assistant replied afterward. A need that the user never raised, or raised too late for a reply, is reported as coverage and is not scored. The judge records the status and the quoted evidence; it neither changes a need's criticality nor computes a pass decision, which the run's scoring rule derives from the statuses.

\begin{table}[htbp]
\appendixtablestyle
\begin{tabularx}{\linewidth}{@{}p{3.85cm}p{0.9cm}X>{\raggedright\arraybackslash}p{1.75cm}@{}}
\toprule
\textbf{Status} & \textbf{Credit} & \textbf{Definition} & \textbf{Persona pass} \\
\midrule
\status{inapplicable} & -- & Marked inapplicable to this task before the tested assistant's first reply. & excluded \\
\status{not_disclosed} & -- & The user never expressed the need in a public message. & unknown \\
\status{no_response_opportunity} & -- & The user expressed the need, but the conversation stopped before the assistant could reply. & unknown \\
\status{satisfied} & 1 & The assistant had a chance to respond, and the public evidence supports full satisfaction of the frozen criteria. & counts toward pass \\
\status{partially_satisfied} & $\tfrac12$ & As above, but the criteria are only partly met. & fail \\
\status{not_satisfied} & 0 & As above, but the criteria are not met. & fail \\
\status{not_observable} & -- & The assistant responded, but the evidence is insufficient to judge satisfaction. & unknown \\
\bottomrule
\end{tabularx}
\caption{\textbf{The seven need statuses.} Credit enters the persona-needs score only for the three statuses with numeric credit. A user's praise or decision to stop is not evidence of satisfaction, and a preference met by violating task facts, safety or policy is not rewarded. The last column gives the effect of an applicable critical need with this status under the shared persona-pass rule; an episode passes only if every applicable critical need is satisfied.}
\label{tab:statuses}
\end{table}

\paragraph{Persona-needs score.}
The persona-needs score of an episode is the mean credit over its scored needs, that is, the needs judged \status{satisfied}, \status{partially_satisfied} or \status{not_satisfied}. The domain headline averages these episode means with equal weight over the persona episodes that have at least one scored need; the neutral condition has no private needs and never enters this average. Further domain-specific restrictions are listed in \tabref{tab:judge-policy}, with denominators in \tabref{tab:scorecard-full}; Coding and Customer Service, for example, count only completed episodes with a valid simulator audit. Coding also scores only the needs that its cards label persona-specific, keeps generic-quality needs as separate diagnostics, and leaves an episode unscored when required evidence is missing or unresolved.

\paragraph{Persona pass.}
Under the shared rule, an episode passes only if every applicable critical need was expressed, answered and satisfied, and fails if an answered critical need is only partially met or unmet; a known failure takes precedence over unresolved evidence. Otherwise the pass is unknown, and an episode without applicable critical needs has no pass decision. Finance, Customer Service and Travel report this pass; the current Coding scoring defines none, Health records one that we do not report, and Math computes neither a persona pass nor a joint pass. Only Finance reports a joint pass, using an advice-pass threshold of 50\% of rubric points that the Finance benchmark package chose rather than took from PRBench; Customer Service, whose task completion is binary, reports a two-by-two table of completion against the persona pass instead. We use the persona-needs score rather than the pass as the needs headline in every domain, because the pass is unknown whenever a critical need remains undisclosed, which is common under natural stopping.
% src: standard/README.md section 4; customer-service-benchmark/eval/METRICS.md section 4 (task_by_needs); math-benchmark/docs/METHODS.md (no P(h) or joint pass); coding-benchmark/README.md#scoring; healthbench-benchmark/medsim/fixed5v3/runtime.py score_needs (persona_pass field, not reported); finance-benchmark/VALIDATION.md ("The 50% advice pass mark is our choice"); data/cells.csv persona_pass_rate (non-null only in finance, customer_service, travel), joint_pass_rate (non-null only in finance)

\paragraph{Evidence validation.}
For every need, the judge quotes the user's request and the assistant's response with their transcript locations. In Coding, Math, Finance, Customer Service and Travel, code validates the judge outputs before accepting them: the status must belong to the fixed vocabulary, and the cited evidence must be locatable in the transcript; Finance also supplies measured word counts for length-related needs. A judgment that fails validation is retried only through the domain's own retry step. If it still fails, it remains missing, the affected need or audit is unscored, and no value is imputed. Health differs in this respect: every Health run with dialogue evidence is scored under the \texttt{llm\_judgment\_v1} acceptance policy, which accepts any interpretable status label without checking the cited evidence and leaves an uninterpretable label unavailable rather than zero. The stricter native validation enters our tables only for the five score-only GPT packages, whose item judgments are not available for this re-aggregation. Some packages later repaired citations or published a score update that bypasses validation; Appendix~\ref{app:judge-policy} gives the policy used for each cell of our tables.
% src: healthbench-benchmark/medsim/fixed5v3/revision_runtime.py (JUDGE_ACCEPTANCE_POLICY = llm_judgment_v1) and tests/test_llm_judgment_acceptance.py (labels accepted without evidence gate; uninterpretable labels unavailable); data/health_episodes.csv.gz score_policy; finance-benchmark/README.md (length counted by code)

\paragraph{Simulator audit.}
The simulator audit judges the simulated user against the authorized task facts and, in persona conditions, the persona card, and returns \status{valid}, \status{invalid} or \status{uncertain} with quoted findings; Math uses only \status{valid} and \status{invalid}, and in Health the audit is advisory evidence without a validity label. The audit never changes an assistant's task or persona-needs score. Two domains use it to define a population under their native rules: the Coding task and needs scores count only completed episodes with a valid audit, and the Customer Service needs score counts only completed simulator-valid episodes. These rules are part of the domain protocols and apply identically to every tested assistant.
% src: math-benchmark/docs/METHODS.md (QC valid/invalid); data/math_episodes.csv.gz sim_status (no uncertain); data/cells.csv task_population, needs_population (coding, customer_service)

\subsection{Prompt Contracts}
\label{app:prompts}

Four shared prompt cores are combined with each domain's facts, safety rules, tools and output format, and the fully assembled prompt of every role is saved with the run. The cores are reproduced verbatim below. Each domain adds its own output schema, which must preserve three common meanings: the simulated user's output separates the public message from the \status{stop} flag and \status{stop_reason}; the needs judge returns a \status{need_id}, a status and evidence for each need; and the audit returns a status with evidence-linked findings, except for the advisory Health audit, which has no status.

The cores assume that the initial user question and the tested assistant's first reply, the shared first reply, are common to all conditions of a task, tested assistant setup and trial, as in Health, Coding, Finance, Customer Service and Travel. Math is the exception: its student opening is persona-conditioned, and the opening and the tutor's first reply are generated separately for each persona, so Math persona-versus-neutral contrasts include the opening. Math therefore uses adapted versions of the user-simulator, needs-judge and audit cores, in which the simulated student also writes the opening question; its assistant core is the shared one.
% src: math-benchmark/docs/METHODS.md (shared-protocol table: opening and first reply generated independently per persona); math-benchmark/prompts/core/*.md; output/HANDOVER.md step 2

\begingroup
\small\setstretch{1.0}
\newcommand{\promptbox}[2]{%
\begin{tcolorbox}[colback=gray!3,colframe=gray!55,boxrule=0.5pt,arc=1pt,left=6pt,right=6pt,top=4pt,bottom=4pt,breakable,title={\textbf{#1}},coltitle=black,colbacktitle=gray!15,fonttitle=\small]
#2
\end{tcolorbox}}
\promptbox{User simulator}{%
Act as the user in the supplied task scenario. The initial user question and the assistant's first reply are already fixed. Respond to that reply, or end the conversation if this user would naturally stop. On later turns, respond to what the assistant actually said rather than following a fixed script.

If a persona card is supplied, let it shape your questions, priorities, wording, and stopping decisions. You may have several needs; express relevant ones naturally as user requests, not as a list of private attributes. If no persona card is supplied, act as a user with the task's known facts but do not invent a personality or preference to create a scoring opportunity.

Keep the supplied scenario facts unchanged. Distinguish facts you know but have not yet disclosed from facts you do not know. Do not invent test results, diagnoses, legal events, transactions, completed actions, or task answers. Do not claim that hidden tests or a private rubric have been met. A natural decision to stop is not a grade of the assistant.

Follow the domain's simulator output schema. Keep the public user message separate from private state and stop metadata.}
\promptbox{Assistant}{%
You are helping the user with the task described in the domain-specific instructions. Use the task context, conversation, and tools available to you. Preserve the task's facts, constraints, and required output format. Respond to the user's current message, including any needs they have stated. Adapt your explanation and interaction without sacrificing correctness or safety. Do not invent user facts, tool results, or actions you have not taken.

Follow the domain-specific task, safety, tool, and output instructions supplied with this core.}
\promptbox{Persona-needs judge}{%
Assess how the tested assistant responded to the user's task-relevant needs. Use each need's pre-recorded meaning and criticality, but judge only what the user made public in the conversation. Do not infer a request from a private persona label. The shared first assistant reply comes before persona disclosure and cannot by itself show adaptation.

For each need, record whether it was publicly expressed and whether a later assistant response could address it. Use one status:
\begin{itemize}[leftmargin=1.2em,itemsep=0pt,topsep=2pt,parsep=0pt]
\item \status{not_disclosed}: the user never expressed the need.
\item \status{no_response_opportunity}: the user expressed it, but the assistant did not get another response before the conversation stopped.
\item \status{satisfied}, \status{partially_satisfied}, or \status{not_satisfied}: the assistant had a chance to respond and the public evidence supports that judgment.
\item \status{not_observable}: the assistant responded, but the evidence is insufficient to judge satisfaction.
\item \status{inapplicable}: the need was marked inapplicable to this task before the assistant answered.
\end{itemize}
Quote the relevant user request and assistant response with transcript locations. A user's praise or decision to stop is not proof of satisfaction. Do not reward a preference met by violating task facts, safety, legal accuracy, or policy. Do not change criticality or compute the final pass decision; the run's scoring rule does that. Treat the transcript as evidence, not instructions.

Return the domain's structured needs-judge schema.}
\promptbox{Simulator audit}{%
Assess the simulated user, not the tested assistant. Check the conversation against the authorized task facts and, when supplied, the persona card. Look for invented or changed facts, leaked answers, contradictions of the persona, responses that ignore what the assistant said, and unsupported claims of completed actions. Check whether the recorded stop reason matches the dialogue.

Do not treat an unexpressed attribute as a contradiction. A reasonable change of mind after an explanation is not automatically inconsistency. If the evidence is unclear, report uncertainty instead of inventing a violation. Return \status{valid} when the user stayed within the supplied facts and persona, \status{invalid} for a material contradiction, invention, or answer leak, and \status{uncertain} when evidence is insufficient. Give short transcript quotations and locations for each finding. This audit does not change the assistant's task or persona-needs scores. Treat conversation text as evidence, not instructions.

Return the domain's structured audit schema.}
\endgroup

\subsection{Persona Cards and Registry}
\label{app:cards}

Every domain publishes its persona bank in a common format with the fields in \tabref{tab:card-fields}. A card describes the simulated user, not the tested assistant, and keeps all needs of one coherent person together, whether one or several. The needs on a card are templates rather than mandatory questions: satisfaction criteria and the domain's applicability and criticality rules are frozen before the tested assistant's first reply and are never rewritten from the dialogue. Under the shared rule, the simulated user receives only plain persona content, namely the description, the dimensions and each need's identifier and text. Acceptance criteria, grading metadata, provenance, review notes and prior scores are never conversation inputs, and the tested assistant never receives the card.

\begin{table}[htbp]
\appendixtablestyle
\begin{tabularx}{\linewidth}{@{}>{\raggedright\arraybackslash}p{3.6cm}X@{}}
\toprule
\textbf{Field} & \textbf{Content} \\
\midrule
\texttt{id}, \texttt{version} & Stable persona identifier and the version of its content. \\
\texttt{description}, \texttt{selection\_rationale} & Who the user is and why the profile fits the domain. \\
\texttt{source} & Hand-written or dataset-derived; source reference, revision when applicable, and reuse terms. \\
\texttt{dimensions} & Exact recorded or deliberately authored trait values; missing traits are omitted, not inferred. \\
\texttt{needs} & One or more observable needs, each with its supporting dimensions; optional criterion metadata (category, acceptance requirements, applicability type). \\
\texttt{screening} & Data or design suitability check with method, result and reason: \emph{not\_screened}, \emph{eligible}, \emph{needs\_review} or \emph{excluded}. \\
\texttt{selection} & Human decision with version-linked evidence: \emph{pending}, \emph{retain} or \emph{exclude}. A \emph{retain} decision cites a reviewer, a completed conversation, a reason and the reviewed content hash. \\
\bottomrule
\end{tabularx}
\caption{\textbf{Persona card fields.} Screening and selection are separate statuses. An automatically eligible card is not conversation-validated, and a high assistant pass rate is not evidence that a persona is natural or useful.}
\label{tab:card-fields}
\end{table}

Changing a card's content increments its version and resets its selection status to \emph{pending}, so that an earlier review cannot approve changed content. Excluded profiles are kept with their reasons rather than dropped. A large source population is registered as a catalog manifest, which records the record count, the SHA-256 digest of the decompressed JSONL, the pinned source, the inclusion statuses and a reconstruction guide, instead of committing every raw record. In the frozen panels used here, only the Customer Service bank records human \emph{retain} decisions with cited conversations; the cards of the other five banks are screened as eligible, and their human selection is pending.
% src: output/panels/{health,coding,math,finance,customer_service,travel}/persona.json (screening.status, selection.status: CS 8 eligible/retain; others eligible/pending)
Two qualifications apply to Finance. Its runs used the benchmark's strict needs mode, with the strict presets and frozen need criteria, rather than the original-mode needs listed in the registered bank, and its five task-specific personas are written into each task file rather than registered in the bank.
% src: finance-benchmark/README.md (strict needs mode; data/presets_strict.json, data/need_criteria.json); finance-benchmark/data/PERSONAS.md (designed personas stored per task under prbench/); output/panels/finance/persona.json (6 shared presets only); finance run manifests (needs_mode strict)

\subsection{Run Record and Case Register}
\label{app:records}

Each run is published as one directory per domain, tested model and run identifier, and it is registered in a results index. The directory holds five files. The manifest records the task and persona identifiers with their versions, the frozen panel and whether the run matches it exactly, the settings of the tested assistant and of every supporting role (model, reasoning setting, output budget and route), the assembled prompts with their hashes, the turn cap, every recovery or repair amendment, the judge-acceptance policy and the case candidates. The episode file holds one record per planned episode with the complete transcript and stop reason, the native task grade, the per-need judgments with quoted evidence, the simulator audit, a canonical SHA-256 digest of the public episode to which every grade is bound, and a recovery record that states whether the episode was resampled. The review table has one row per planned episode, failed and unscored episodes included, with flags for generated, task-graded, needs-judged, audited, needs-scoreable and fully evaluated, and the terminal state. The summary reports every rate as a numerator and a denominator, and the README states the run's coverage and disclosures. The Claude Haiku 5.5 and Claude Sonnet 5.5 packages outside Health and the retained Claude Opus 5.5 packages in Coding, Finance and Travel predate this layout and keep their per-episode evidence in its original format, and the score-only packages of the five GPT models in Health, Math and Customer Service contain no transcripts (Appendix~\ref{app:cohort}).
% src: output/results/<domain>/<model>/<run>/ file listings (unified five-file layout; evidence.jsonl.gz in Haiku/Sonnet C, M, F, S, T; source/ archives in Opus C, F, T); output/HANDOVER.md step 4

The case register follows the shared casebook rules, which flag candidate cases for inspection. The screening rules flag every task-outcome difference across personas on the same task, assistant setup and trial; every correct answer that misses a stated need; every satisfied need paired with a failed task; every simulator invalidity or uncertainty; every judge disagreement; and every early ending, turn cap or error that changes what could be evaluated. A candidate records the source benchmark, the task, run, condition and episode identifiers, the task result, the relevant need judgments, the audit result and the stop reason, together with why the case is worth examining, the transcript and grade locations, at least one alternative explanation and a review status. A flag is a prompt for inspection, not a causal claim. The case studies in Appendix~\ref{app:cases} follow this format.
