# Supplementary material for: PersonaChatBench: Evaluating Chat Assistants with Diverse Simulated Users
Source: arXiv:2610.42060 source file (2026-10-30)
Supplement: Supplementary file 14 [file runs.tex]

% Appendix B: models, runs, coverage, judge policies and local serving.
% Numbers come from data/cells.csv, data/models.csv, data/failures.csv,
% data/tables_key_numbers.json, data/verification.md and data/build_manifest.json;
% local-serving facts come from the run manifests of the twelve local runs.

This appendix documents how each of the 119 runs, one per tested model and domain, was configured and executed, which cells form the main cohort, how many of the planned episodes produced evidence, which judge-output policy each cell uses, and how the two open-weight models were served.
% src: data/tables_key_numbers.json domains.runs = 119

\subsection{Tested Models and Per-Domain Configuration}
\label{app:config}

The 20 tested assistants are listed in \tabref{tab:models}. They are Claude Haiku 5.5, Claude Sonnet 5.5 and Claude Opus 5.5 \citep{anthropic2026claude55}, Fable 5.1 \citep{anthropic2026fable51}, GPT-5.5 \citep{openai2026gpt55}, GPT-5.6 Sol and GPT-5.6 Terra \citep{openai2026gpt56}, GPT-6 Luna, GPT-6 Sol and GPT-6 Astra \citep{openai2026gpt6}, Gemini 3.7 Flash and Gemini 3.8 Flash \citep{google2026gemini37flash,google2026gemini38flash}, Grok 4.6 \citep{xai2026grok46}, Kimi K3 \citep{moonshot2026kimik3}, MiniMax M3 \citep{minimax2026m3}, DeepSeek V4.1 Flash \citep{deepseek2026v41flash}, GLM 5.3 Flash \citep{zhipu2026glm53flash}, Qwen 3.8 Flash \citep{qwen2026qwen38flash}, and the open-weight Qwen 3.8 27B and Muse Glimmer 30B, whose weights we take from the Hugging Face repositories cited in Appendix~\ref{app:local-serving}.
% src: data/models.csv label (20 rows)
Eighteen models were queried through hosted endpoints: the Anthropic models through AWS Bedrock, the Gemini models through a GCP-routed endpoint, GLM 5.3 Flash and Qwen 3.8 Flash through a hosted OpenAI-compatible gateway, and the remaining models through hosted APIs whose route the packages record only partly or not at all.
% src: data/models.csv serving_route
Qwen 3.8 27B and Muse Glimmer 30B were served locally with vLLM, as described in Appendix~\ref{app:local-serving}.

The configuration was not uniform across models, and we report it rather than harmonize it after the fact. The tested assistant's reasoning setting was medium in every cell except in four groups: MiniMax M3 ran with thinking off and DeepSeek V4.1 Flash with low effort in all six domains, Grok 4.6 ran at high effort in Health and Finance, and Claude Opus 5.5 ran at high effort in every domain except Math.
% src: data/models.csv thinking_<domain>; data/cells.csv thinking
Output budgets were set by each package's runner and were not harmonized, and 54 of the 119 runs record no budget (\tabref{tab:models}). The recorded budgets range from 8,192 tokens, used in Travel by the two Gemini packages, three Claude packages and five GPT packages, to 128,000 tokens, used in Coding by Claude Opus 5.5 and five GPT packages.
% src: data/models.csv output_budget_<domain>; data/cells.csv output_budget_tokens (54 missing among the 119 runs; 8192 in travel for Gemini 3.7/3.8 Flash, Claude Opus/Haiku/Sonnet 5.5, GPT-5.5, GPT-5.6 Sol/Terra, GPT-6 Astra/Sol; 128000 in coding for Claude Opus 5.5, GPT-5.5, GPT-5.6 Sol/Terra, GPT-6 Astra/Sol)
The two local models had a budget of 65,536 tokens, reasoning included, in every domain (Appendix~\ref{app:local-serving}).
% src: data/models.csv output_budget_<domain> for qwen-3-8-27b and muse-glimmer-30b
The supporting roles, that is, the simulated user, the task judge where the domain uses one, the needs judge and the simulator audit, were played by GPT-6 Luna at medium effort in every cell except those marked in \tabref{tab:exceptions}. GPT-6 Luna therefore also simulated and judged its own conversations in all six domains, and its needs scores carry a self-judging caveat.
% src: data/cells.csv support_roles (gpt-6-luna rows)

\subsection{Main Cohort and Marked Exceptions}
\label{app:cohort}

A cell belongs to the main cohort if its run matches the frozen task and persona panel exactly, every supporting role is GPT-6 Luna at medium effort, the registry lists the run as complete, and the package contains full dialogue evidence rather than score rows only. The rule also requires the registry's final-data flag; the Claude Haiku 5.5 and Claude Sonnet 5.5 packages outside Health predate that flag and are admitted on the other four conditions.
% src: data/verification.md section E (expected main_cohort rule); data/cells.csv final_data_missing_old_format
The rule admits 92 of the 119 cells: 12 in Health, 14 in Coding, 15 in Math, 18 in Finance, 14 in Customer Service and 19 in Travel.
% src: data/build_manifest.json main_cohort_sizes; data/tables_key_numbers.json non_main_cells.main = 92
Twelve models are in the main cohort of all six domains.
% src: data/build_manifest.json main_cohort_all6 (12 models)
The remaining 27 cells comprise 7 cells with different supporting models, 15 score-only packages and 5 runs registered as partial; the one remaining combination of model and domain, Fable 5.1 in Health, has no run.
% src: data/tables_key_numbers.json non_main_cells = {support 7, scoreonly 15, partial 5, norun 1}
\tabref{tab:exceptions} lists every marked configuration. Tables in the paper print these cells in gray with the same markers, and the headline rank statistics use only main-cohort cells.

\begin{table}[htbp]
\appendixtablestyle\footnotesize
\begin{tabularx}{\linewidth}{@{}p{0.3cm}>{\raggedright\arraybackslash}p{3.1cm}>{\raggedright\arraybackslash}p{1.45cm}>{\raggedright\arraybackslash}X@{}}
\toprule
& \textbf{Models} & \textbf{Cells} & \textbf{Difference from the main-cohort configuration} \\
\midrule
$^{\dagger}$ & Claude Opus 5.5 & H, C, F, S, T & Tested at high effort. Supporting roles Sol-h in C, F and T; mixed by condition in H (Sol-h for the neutral user, P1, P2 and P5; Luna-m for P3 and P4) and mixed by episode in S. The Health package judges three needs instead of the panel's two for P1, P2 and P5. The Math run (medium effort, Luna-m) is in the main cohort. \\
$^{\dagger}$ & Grok 4.6 & H, F & Tested at high effort; all supporting roles Sol-h. The Health package judges three needs instead of the panel's two for P1, P2 and P5. The other four domains use medium effort and Luna-m. \\
$^{\ddagger}$ & GPT-5.5, GPT-5.6 Sol, GPT-5.6 Terra, GPT-6 Astra, GPT-6 Sol & H, M, S & Score-only packages without full dialogue evidence; registry status unverified. Health reports native-strict judge acceptance because the item judgments needed for the common acceptance policy are absent. Math additionally lacks an exact panel record and uses GPT-6 Luna at high or unrecorded effort by role. Math provides item-level judgments without transcripts, and Customer Service per-episode scores without transcripts or item-level judgments. \\
$^{\S}$ & the same five GPT models & C & Registered as partial; full dialogues are present, but failed judge calls remain missing (for GPT-6 Astra, 69 of 700 episodes have an audit). \\
-- & Fable 5.1 & H & No run. \\
& MiniMax M3; DeepSeek V4.1 Flash & all & Thinking off; low effort. Both remain in the main cohort. \\
& Claude Haiku 5.5, Claude Sonnet 5.5 & all & GPT-6 Luna reached through AWS Bedrock rather than the Azure route used for the local models. Older package format in C, M, F, S and T; citation repair in C and F and evaluation catch-up in T (Appendix~\ref{app:judge-policy}). \\
$^{\circ}$ & MiniMax M3; Claude Haiku 5.5; GLM 5.3 Flash; Qwen 3.8 Flash & H; H; C; C and M & Fewer than 80\% of planned episodes generated: 932, 657, 443, 364 and 985 episodes, in the order listed. Their failed episodes remain in the planned totals. \\
\bottomrule
\end{tabularx}
\caption{\textbf{Configurations outside the main cohort and other marked differences.} Domains: H Health, C Coding, M Math, F Finance, S Customer Service, T Travel. Markers match \tabref{tab:scorecard} and \tabref{tab:coverage}. Rows without a marker and the low-generation row ($^{\circ}$) describe cells that remain in the main cohort but differ in a recorded setting. Sol-h: GPT-5.6 Sol at high effort; Luna-m: GPT-6 Luna at medium effort.}
\label{tab:exceptions}
\end{table}
% src: data/cells.csv cohort_exclusion_reason, support_roles, thinking, notes (Grok 4.6 and Claude Opus 5.5 health: 3 needs for P1/P2/P5), audited (GPT-6 Astra coding 69); data/models.csv route_<domain> (Haiku/Sonnet support us.openai.gpt-6-luna); local run manifests notes (Luna through Azure); data/tables_key_numbers.json low_generation_main_cells

GLM 5.3 Flash and Qwen 3.8 Flash are listed as partial in the benchmark's progress table for Health and Coding, although their registered runs are closed and every planned episode has a terminal state. These cells meet the main-cohort rule and carry the low-generation marker where it applies.
% src: data/cells.csv progress_table_status = Partial, registry_status = complete (GLM 5.3 Flash, Qwen 3.8 Flash; health, coding)

\subsection{Planned and Generated Episodes}
\label{app:coverage}

\tabref{tab:coverage} reports, for every cell, how many of the planned episodes were generated, task-graded, needs-judged, needs-scoreable and audited. Over the 119 runs, 126,460 episodes were planned and 122,569 (96.9\%) were generated.
% src: data/tables_key_numbers.json coverage.total (planned 126460, generated 122569)
The planned total is 20 models times 6,383 episodes per model, less the 1,200 episodes of the missing Fable 5.1 Health run.
% src: data/tables_key_numbers.json domains.<d>.episodes_per_model (1200+700+1435+1164+1452+432 = 6383); 20*6383-1200 = 126460
Generation rates were 93.5\% in Health (21,309 of 22,800), 94.4\% in Coding (13,218 of 14,000), 96.6\% in Math (27,731 of 28,700), 97.8\% in Finance (22,778 of 23,280), 99.9\% in Customer Service (29,019 of 29,040) and 98.5\% in Travel (8,514 of 8,640).
% src: data/tables_key_numbers.json coverage.<domain>.All runs (generated / planned)
Within the main cohort, 91,380 of 95,213 planned episodes (96.0\%) were generated.
% src: data/cells.csv sum of generated and planned over main_cohort == True
Over all runs, 78,846 of the 95,450 persona episodes with a needs judgment (82.6\%) had at least one scoreable need under the domain's native rule, that is, a need that the user expressed, that the assistant had a chance to answer and that the judge could score.
% src: data/tables_key_numbers.json coverage.total (needs_judged 95450, needs_scoreable 78846)

The coverage counts follow each domain's native definitions, which differ in three respects. First, Health grades the recorded part of a dialogue whose generation failed, so its task-graded count can exceed its generated count. Second, Coding, Finance and Customer Service count a conversation that reached the turn cap as completed, whereas Travel leaves a capped episode without a primary task score, so it is neither generated nor task-graded there, and Health records its single capped conversation as a failure but grades it. Third, an accepted needs judgment is missing for most Coding persona episodes: only 4,120 of the 12,000 planned Coding persona episodes have one. In the packages that record the reason, most missing judgments failed the evidence check, the most frequent reason being a quotation that did not match the cited transcript message exactly; in the GPT-6 Astra package, most needs-judge calls failed outright. These judgments remained missing under the policies described in Appendix~\ref{app:judge-policy}.
% src: data/<domain>_episodes.csv.gz terminal_state (coding cap stops 'completed'; finance turn_cap 1,566 and customer_service turn_cap 23 generated; travel turn_cap 30 + tool_cap 3 not generated; health turn_cap 1, Claude Sonnet 5.5, not generated, task-graded); data/failures.csv turn_cap, tool_cap
% src: data/tables_key_numbers.json coverage.coding.All runs.needs_judged = 4120; 20 runs x 100 tasks x 6 personas = 12000; output/results/coding/*/data.jsonl.gz grades.errors.needs (recorded in the five GPT, Qwen 3.8 27B and Muse Glimmer 30B packages; leading message "Evidence must quote the indexed transcript message exactly"; GPT-6 Astra "judge: request failed")
Every failed, capped or unscored episode is counted in the planned totals of \tabref{tab:coverage}. Failures were kept as recorded, except where a package reran or continued failed generations under a documented recovery amendment; each amendment is recorded in the package manifest and summarized in \tabref{tab:judge-policy} and Appendix~\ref{app:local-serving}.

\tabref{tab:persona-effects} collects, for every persona condition of the six domains, the distribution over main-cohort models of the paired persona-minus-neutral change in the native task grade that \figref{fig:persona} plots; the persona tables of Appendices~\ref{app:health}--\ref{app:travel} give the corresponding needs scores, and their persona-effects subsections the mechanisms.
% src: tables/persona_effects.tex (generated by scripts/make_tables.py from data/persona_effects.csv, main-cohort rows)

\input{tables/scorecard}
\input{tables/coverage}
\input{tables/scorecard_full}
\input{tables/persona_effects}

\subsection{Judge-Output Policies}
\label{app:judge-policy}

The packages did not handle judge outputs that failed validation in the same way, and these differences change the size of the needs populations. \tabref{tab:judge-policy} gives, for each domain, the headline populations and every package-specific departure from the default policy. The default policy is the domain's native in-run retry, after which a judgment that still fails validation stays missing.

Two policy differences matter most for interpretation. First, the Gemini 3.7 Flash and Gemini 3.8 Flash packages publish a score update built from raw judge decisions with the code validation bypassed. Our headline uses their original validated judge outputs, as for every other model, and the domain tables report the raw-judge values as alternates. The choice matters most in Coding, where the original validation rejected 540 and 525 needs judgments, respectively, so the headline needs scores rest on 54 and 64 episodes, against 578 and 584 under the raw-judge update.
% src: data/cells.csv repaired_judges (coding Gemini: original_judgment_rejected:needs 540 / 525), needs_den 54 / 64, needs_den_alt_policy 578 / 584
Second, the Claude Haiku 5.5 and Claude Sonnet 5.5 packages went through a separate citation-repair and criterion catch-up pass, and the Fable 5.1 and Claude Opus 5.5 packages through bounded evidence corrections, which no other package received. In Coding, these four packages have 585 to 591 needs-scored episodes, whereas every other run has between 19 and 190.
% src: data/cells.csv coding needs_den (Fable 585, Sonnet 586, Haiku 590, Opus 591; others 19-190)
Coding needs scores are therefore not comparable in coverage across packages, and we do not interpret Coding needs rankings.

\begin{table*}[t]
\tablestyle{3pt}{1.12}\scriptsize
\begin{tabularx}{\linewidth}{@{}>{\raggedright\arraybackslash}p{1.45cm}>{\raggedright\arraybackslash}p{5.2cm}>{\raggedright\arraybackslash}X@{}}
\toprule
\textbf{Domain} & \textbf{Headline populations} & \textbf{Package-specific judge-output policies and recovery amendments} \\
\midrule
Health & Task: all planned episodes with a task score, including graded partial dialogues of failed episodes. Needs: P1--P5 episodes with at least one expressed, answered and observable need. Audit advisory. & Every run with dialogue evidence uses the \texttt{llm\_judgment\_v1} acceptance of the saved judgments (offline re-aggregation without model calls), which accepts any interpretable judge label without checking the cited evidence; the five score-only GPT packages ($^{\ddagger}$) report native-strict acceptance. Gemini raw-judge and original values are identical. Claude Haiku 5.5 and Claude Sonnet 5.5: a separate recovery continued the failed episodes from their accepted prefix with schema-constrained doctor calls; it is not pooled, and the headline uses the primary run. \\
\addlinespace[2pt]
Coding & Task: completed episodes with a valid simulator audit; a missing or malformed submission scores 0. Needs: persona-specific needs under the native scoreability rule, in completed simulator-valid persona episodes. Simulator validity: valid over audited episodes. & Claude Haiku 5.5 and Claude Sonnet 5.5: exact-citation revision on 493 and 482 episodes plus bounded corrective judgments. Fable 5.1: bounded evidence corrections. Claude Opus 5.5: scoring repair and score overlay. Gemini: original validated outputs; raw-judge update as alternate. The five GPT packages ($^{\S}$): captured judgments unchanged, failed calls missing. Local models: native retry, at most two passes. Generation recovery: Gemini, Claude Haiku 5.5 and Claude Sonnet 5.5 reran failed generations with the budget raised to 65,536 tokens; GLM 5.3 Flash and Qwen 3.8 Flash resumed twice with retries of failed requests at an unchanged budget. \\
\addlinespace[2pt]
Math & Task: persona episodes with a tutor grade; the neutral condition is reported separately. Needs: persona episodes with at least one scored need. & Muse Glimmer 30B: eight episodes whose needs judgment is marked partially validated but carries a score are included. Gemini: original validated outputs; raw-judge update as alternate. Generation recovery: Qwen 3.8 27B and Muse Glimmer 30B resent the 32 tutor calls per model interrupted by a server stop (recovery r1); Claude Haiku 5.5 and Claude Sonnet 5.5 closed grading and transport gaps by exact replay of accepted calls and bounded retries at 65,536 tokens; Fable 5.1 retried failed requests and technical grading failures; GLM 5.3 Flash and Qwen 3.8 Flash regenerated failed scenes once at the same budget, all of which failed again, and reran fully failed tasks at 32,768 tokens as a separate recovery cohort that the headline does not use. \\
\addlinespace[2pt]
Finance & Task: all recorded episodes with an advice percent and no advice-validation error, neutral included. Advice pass: persona conditions only. Needs: all recorded persona episodes with at least one scoreable need, any audit status. & Claude Haiku 5.5 and Claude Sonnet 5.5: citation repair and criterion catch-up on 28 and 40 graded episodes; two Claude Haiku 5.5 episodes regenerated in a generation-gap recovery. Fable 5.1: technical grading-failure recovery on 93 episodes. Claude Opus 5.5: three blocked tasks (36 conditions) regenerated at 65,536 tokens and 30 transport-failed episodes continued. Qwen 3.8 27B and Muse Glimmer 30B: five and eight tasks that were in flight at an interruption regenerated on resume, final attempt kept. GLM 5.3 Flash and Qwen 3.8 Flash: three and 18 fully failed tasks rerun at 32,768 tokens as a separate recovery cohort that the headline does not use. Kimi K3: 49 advice judgments that failed validation are excluded. Gemini: the package headline bypasses validation and word-count caps; we use the original grades. \\
\addlinespace[2pt]
Customer Service & Task: all planned episodes; an incomplete episode counts as not complete. Persona effects: graded completed episodes. Needs: completed persona episodes with a valid simulator audit. & Episodes that stopped with an agent or simulator error count as not complete even when they carry a rule-based outcome: four for DeepSeek V4.1 Flash, four for GPT-5.6 Sol, six for Grok 4.6 and seven for Kimi K3 (four agent and three simulator errors). Claude Haiku 5.5 and Claude Sonnet 5.5: generation and grading gap repair with replay of accepted calls. Fable 5.1: technical grading recovery. Gemini raw-judge and original values are identical. \\
\addlinespace[2pt]
Travel & Task: all recorded official-task episodes with a native score; capped and failed episodes are null, not imputed; authored revision tasks are scored separately. Needs: all recorded persona episodes with at least one expressed and answered need. & Claude Haiku 5.5 and Claude Sonnet 5.5: evaluation catch-up on 32 and 29 episodes. Claude Opus 5.5: deterministic quotation repair on four needs judgments and transport-timeout continuation on three episodes. Fable 5.1: grade recovery on 27 episodes. GLM 5.3 Flash and Qwen 3.8 Flash: the eight and seven error episodes of the first pass archived and generated again on resume at the unchanged cap; judge errors kept. Gemini: task and audit identical under both policies; needs differ (headline 251 and 254 episodes, raw-judge 289 and 287). \\
\bottomrule
\end{tabularx}
\caption{\textbf{Headline populations, judge-output policies and recovery amendments by domain.} The default policy, not repeated in the table, is the domain's native in-run retry; a judgment that still fails validation stays missing and is not imputed. Recovery amendments that reran or continued failed generations are listed with the package. Gemini values refer to Gemini 3.7 Flash and Gemini 3.8 Flash in that order. The domain appendices report the alternate (raw-judge) Gemini values.}
\label{tab:judge-policy}
\end{table*}
% src: data/cells.csv task_population, needs_population, repaired_judges, headline_judge_policy, needs_den, needs_den_alt_policy, notes (incl. GLM/Qwen Flash math "primary pass only ... recovery cohort never pooled"; Fable/Haiku/Sonnet math recovery notes); data/verification.md (reproduction notes: Math Muse partial_validation 8 episodes; Finance Kimi K3 49 exclusions) and addendum items 1-3; data/customer_service_episodes.csv.gz terminal_state (agent_error: DeepSeek V4.1 Flash 4, GPT-5.6 Sol 4, Grok 4.6 6, Kimi K3 4; simulator_error: Kimi K3 3; every one with a task_complete_rule value) and data/failures.csv customer_service; data/health_episodes.csv.gz score_policy; data/persona_effects.csv task_population (customer_service: graded completed episodes); health Haiku/Sonnet manifests primary_and_recovery (primary_is_default true); local math manifests ("Recovery r1 resent the 32 teacher calls per model"); local finance manifests recovery.native_resume.regenerated_task_ids (5, 8; interrupted_in_flight); GLM/Qwen Flash finance and math manifest notes (3 and 18 tasks; 111 and 219 scenes re-failed; 32,768-token recovery cohort); travel manifests output/results/travel/{glm-5-3-flash,qwen-3-8-flash}/*/manifest.json resume (original_pass error 8 and 7; run.py run --resume --retry-errors; pre_resume_episodes_archived true)

\subsection{Local Serving of Qwen 3.8 27B and Muse Glimmer 30B}
\label{app:local-serving}

The two open-weight models were served on local GPUs with vLLM 0.30.0 \citep{kwon2023vllm} in BF16. The weights are those of the Hugging Face repositories Qwen/Qwen3.8-27B at revision \texttt{1d4bf0f2ff60} \citep{hf2026qwen38_27b} and meta-models/Muse-Glimmer-30B at revision \texttt{a4e59da52a7b} \citep{hf2026museglimmer30b}, verified against a recorded model manifest before the runs.
% src: data/models.csv weights_hf_repo, weights_revision; run manifests setup.lineage.tested_model (hf_repo, revision, dtype, weights_verified_at)
The servers used a maximum context of 131,072 tokens, a fixed seed and each model's default generation configuration.
% src: run manifests setup.lineage.serving.serve_command (--max-model-len 131072, --seed 0, --generation-config auto)
The reasoning setting was medium in every domain and was set per request through a chat-template variable, \texttt{reasoning\_effort} for Qwen 3.8 27B and \texttt{reasoning\_strength} for Muse Glimmer 30B.
% src: data/models.csv thinking_health; run manifests notes ("Reasoning settings were set per request by the router")
In Health and Customer Service, the local router raised the runners' native caps of 12,000 and 6,000 tokens to the common budget of 65,536 tokens, and the request log keeps both the requested and the enforced budget.
% src: run manifests notes ("Output caps: ... raised the native Customer Service (6,000) and Health (12,000) caps"); data/models.csv output_budget_<domain>
All supporting roles were played by GPT-6 Luna at medium effort through Azure OpenAI, whereas the Claude Haiku 5.5 and Claude Sonnet 5.5 packages reached GPT-6 Luna through AWS Bedrock. Every GPT-6 Luna call in the local campaign received at least 8,192 output tokens, a floor that exceeds the native supporting-role budgets only in Customer Service, where they are 500 to 1,200 tokens.
% src: run manifests notes ("GPT-6 Luna medium ran through Azure, not Bedrock"; "Luna minimum output: every Luna call had at least 8,192 output tokens ... 500-1,200")

Several serving settings are intended to affect only throughput and latency and leave the prompts and decoding parameters unchanged. They are speculative decoding (multi-token prediction for Qwen 3.8 27B and a draft model for Muse Glimmer 30B), prefix caching, priority scheduling, a keepalive that sent leading whitespace before the JSON body of long responses, and, from the resumption described below, up to three identical Qwen 3.8 27B replicas with the same weights, flags and seed behind a queue-based balancer.
% src: run manifests setup.lineage.serving.serve_command (--speculative-config mtp / dflash, --enable-prefix-caching, --scheduling-policy priority); notes (keepalive; replicas)
Three output-handling settings can affect what a reply contains. Muse Glimmer 30B ran with an answer-gate reasoning parser, so that structured-output constraints apply to the answer channel and not to the reasoning. Runs of whitespace inside JSON-object replies were capped at 32 characters, and strict JSON schemas used compact whitespace, as hosted strict-output modes do. Finally, a call whose final answer contained reasoning markers failed at the router, so reasoning text could not enter transcripts, tool parsing or judges.
% src: run manifests notes (answer-gate plugin; JSON whitespace plugin, 32 characters; compact strict JSON; reasoning leak policy)
A first Health run was voided because compact JSON whitespace corrupted about 4\% of the Qwen 3.8 27B doctor replies; both models were rerun in full, and only the rerun is reported.
% src: health run manifests notes ("The first Health run (r1) is void ... about 4% of Qwen doctor replies ... rerun in full under the -r2 run id")

An automatic GPU-driver upgrade stopped every local job on 2026-10-15 between 18:24 and 18:26 CDT, and the runs resumed at 23:52 CDT under each benchmark's native resume rules. Health recorded the doctor calls in flight at the stop, eight per model, as interrupted and did not resample them. Math resent the 32 interrupted tutor calls per model once through its native recovery script.
% src: run manifests notes ("Incidents: an automatic NVIDIA driver upgrade stopped every job on 2026-10-15 at 18:24-18:26 CDT ... resumed at 23:52 CDT"; Health "8 per model ... interrupted_inflight_no_resample"; Math "Recovery r1 resent the 32 teacher calls per model"); data/failures.csv interrupted (health: 8 per model)
A planned router restart of 3.5 seconds on 2026-10-16 deployed new timeouts and failover. In Finance, the native runner regenerated on resume the tasks that had been in flight at an interruption, five for Qwen 3.8 27B and eight for Muse Glimmer 30B, and kept only the final attempt of each; the earlier attempts survive only in the router log.
% src: run manifests notes ("A planned router restart on 2026-10-16 at 12:53 CDT (3.5 s)"; finance "Regenerated tasks (5)" / "Regenerated tasks (8)"; "earlier attempts survive only in the router ledger"); finance manifests recovery.native_resume.invocations (interrupted_in_flight) and recovery.native_resume.regenerated_task_ids
Apart from these recovery steps, the local runs kept every failure as recorded: no other episode was resampled, and no answer or score was substituted.

The recorded failures of the two local models are concentrated in a few cells (\tabref{tab:coverage}). Qwen 3.8 27B often ended a long reasoning trace without an answer or reached the output budget: in Coding, 117 episodes ended with an empty or incomplete assistant output, 112 of them because the shared first reply of 16 tasks was never produced; in Math, 94 tutor answers were empty and six were truncated; and in Health, 129 episodes failed with protocol or format errors in the structured output.
% src: data/failures.csv (coding qwen empty_answer 117; math qwen empty_answer 94, truncated 6; health qwen protocol_format 129); coding run manifest notes ("112 of them have no shared first reply (16 units x 7 conditions)")
Muse Glimmer 30B produced 170 Finance conversations that stopped on an API error, 169 of them on a tested-model reply, and 24 empty outputs in Travel.
% src: data/failures.csv (finance muse other 170; travel muse empty_answer 24); finance run manifest notes ("169 tested-model replies, 1 Luna user-simulator turn")
In Customer Service, 660 of Muse Glimmer 30B's 1,452 conversations contain no tool call, and the model often announced an action in prose without writing the required tool marker; token accounting against the serving logs identifies this as model behavior under the shared text-marker protocol rather than a serving artifact (Appendix~\ref{app:service-caveats}; case study in Appendix~\ref{app:case-service}).
% src: data/muse_tool_diagnosis.md sections 1, 4 and 8 (660 zero-tool episodes of 1,452; token accounting; discarded channels at most about 1.6% of calls, reported in Appendix app:service-caveats, with the case study in app:case-service)
Judge retries used only the benchmarks' own retry steps, so the persona-judgment coverage of the local runs is not directly comparable with that of the repaired Claude Haiku 5.5 and Claude Sonnet 5.5 packages.

\subsection{Sensitivity of the Cross-Domain Rank Statistics}
\label{app:rank-sensitivity}

The cross-domain task statistics of \secref{sec:consistency} rest on the 12 models in the main cohort of all six domains, so single models can move them. \tabref{tab:rank-sensitivity} recomputes Kendall's $W$ and the Spearman correlations of Health with the other five domains after leaving out MiniMax M3, Muse Glimmer 30B, both of them, or any one of the other ten models.
Leaving out MiniMax M3 or Muse Glimmer 30B alone lowered $W$ over the five domains other than Health from 0.64 to 0.56, and leaving out both lowered it to 0.44 ($n=10$, $p=0.010$), whereas $W$ over all six domains stayed between 0.35 and 0.46 under every exclusion.
The mean correlation of Health with the other domains rose from $-0.19$ to 0.02 without either model and to 0.32 without both, whereas leaving out any other single model kept it between $-0.31$ and $-0.16$.
% src: recomputed from data/cells.csv task_value (main_cohort=True in all six domains, 12 models) with the kendall_w and corr_perm statistics of scripts/build_dataset.py (10,000 permutations, seed 0); the all-model row reproduces data/rank_consistency.csv (task W 0.421 and 0.641); not stored in data/
The agreement among the five domains other than Health therefore survives every exclusion, but its strength, and the extent to which Health disagrees, depend on these two models.

\begin{table}[htbp]
\appendixtablestyle\footnotesize
\begin{tabular}{@{}lrcccc@{}}
\toprule
\textbf{Models left out} & $n$ & \textbf{$W$, six domains} & \textbf{$W$, without Health} & \textbf{Mean $\rho$ of Health} & \textbf{$\rho$ of Health with C / M / F / S / T} \\
\midrule
None & 12 & 0.42 (0.001) & 0.64 ($<$0.001) & $-$0.19 & $-$0.07 / $-$0.14 / 0.11 / $-$0.60 / $-$0.24 \\
MiniMax M3 & 11 & 0.42 (0.002) & 0.56 ($<$0.001) & 0.02 & 0.21 / 0.12 / 0.27 / $-$0.48 / $-$0.02 \\
Muse Glimmer 30B & 11 & 0.42 (0.002) & 0.56 ($<$0.001) & 0.02 & 0.21 / 0.12 / 0.42 / $-$0.48 / $-$0.16 \\
Both & 10 & 0.42 (0.003) & 0.44 (0.010) & 0.32 & 0.61 / 0.49 / 0.70 / $-$0.31 / 0.12 \\
\addlinespace[2pt]
One of the other ten & 11 & 0.35--0.46 & 0.59--0.70 & $-$0.31 to $-$0.16 & -- \\
\bottomrule
\end{tabular}
\caption{\textbf{Sensitivity of the cross-domain task-rank statistics to the models included.} Kendall's $W$ of the native task headline over all six domains and over the five domains without Health, with the one-sided permutation $p$ (10,000 permutations) in parentheses, and Spearman's $\rho$ between the Health task ranking and that of each other domain, with their mean. Domains: C Coding, M Math, F Finance, S Customer Service, T Travel. Base population: the 12 models in the main cohort of all six domains. The last row gives the range over the ten recomputations that each leave out one of the other models; the largest permutation $p$ of any $W$ in these recomputations is 0.010.}
\label{tab:rank-sensitivity}
\end{table}
% src: same recomputation as above (W six domains p_perm 0.0013, 0.0016, 0.0021, 0.0031, other ten 0.0003-0.0102; W five domains p_perm 0.0001, 0.0004, 0.0003, 0.0100, other ten <=0.0002; Spearman with two-sided permutation p)
