# Supplementary material for: PersonaChatBench: Evaluating Chat Assistants with Diverse Simulated Users
Source: arXiv:2610.42060 source file (2026-10-30)
Supplement: Supplementary file 15 [file service.tex]

% Customer Service domain appendix. Every number is taken from data/ in this repository;
% protocol facts follow the benchmark checkout listed in data/domain_facts.json.
% Main cohort only for comparisons; marked configurations are described as such.

The Customer Service domain evaluates a tested assistant that acts as a support agent with a written policy and a set of tools in conversations with a simulated customer.
The cases are built on the subflows and agent guidelines of the Action-Based Conversations Dataset (ABCD)~\citep{chen2021abcd}, and the native task grade asks whether the agent handled the case correctly and in accordance with the policy.
What varies is how the customer talks, what the customer asks for and how the customer reacts to a refusal.

\subsection{Source and Task Panel}
\label{app:service-panel}

\paragraph{Case construction.}
Because ABCD provides agent guidelines and transcripts but no grading rubric, the benchmark quotes the policy text from the ABCD guidelines and takes customer identities from ABCD scenarios, whereas the deciding facts, the pre-recorded tool results and the correct outcome of each case were written and computed by hand.
The cases cover five policy classes: cases in which the agent must approve or refuse by rule, cases in which it must escalate, cases whose correct action depends on whether the customer keeps pushing, cases in which the customer misremembers a fact that the record contradicts, and cases in which the agent must verify the customer's identity before acting.
Some policy texts contain sentences that are not in ABCD, such as an offer to escalate to a manager after a refusal or the timing of a refund; the benchmark records each such sentence as its own addition.

\paragraph{Task panel.}
The panel contains 132 policy items.
% src: data/tables_key_numbers.json domains.customer_service.tasks=132; data/domain_facts.json domains.customer_service.task_note
Most cases exist in two policy variants, with and without an escalation route, and the panel keeps the variant with the route.
This rule does not look at any score, but it was chosen because an earlier full run had located the persona effect on that side; the eight persona cards were likewise chosen from earlier results, on two axes: the change in completion relative to the neutral customer and the share of critical needs left unmet.
The panel is therefore a case-study panel selected using earlier results, and its scores do not estimate performance on customer service in general.

\paragraph{Tools.}
Tools are text markers: the agent writes \texttt{[tool | arguments]} on its own line, and a listed tool returns a pre-recorded result that only the agent sees.
The customer receives the agent's messages with the markers removed.
An executed tool constitutes the decision, so approving in words without the tool is not approval.

\paragraph{Roles and protocol.}
Each item is run once under each of eight persona cards and three times under the neutral condition, which gives 1,452 planned conversations per model.
% src: data/tables_key_numbers.json domains.customer_service (persona_conditions=8, neutral_trials=3, episodes_per_model=1452); data/domain_facts.json domains.customer_service.condition_note
A fixed greeting precedes a persona-free opening that states the goal and the customer's identity but withholds the deciding facts.
The agent's first reply, including any tool calls and results, is shared within a trial: each of the three neutral trials has its own first reply, and the persona conditions reuse that of the first trial.
% src: customer-service-benchmark/eval/PROTOCOL.md section 3 items 7 and 12 (each trial has its own shared first reply; neutral 3 trials, personas 1) -- benchmark checkout
The conversation ends when the customer stops or after 24 agent messages, counting tool follow-ups.
% src: data/domain_facts.json domains.customer_service.turn_cap=24, turn_cap_unit
The agent sees the policy, the tool list, the public conversation and its own tool results, but not the persona card or the correct outcome.
The customer sees its goal, the facts it knows and does not know and its persona card, but not the policy, the tools, the tool results or the correct outcome.

\paragraph{Cohort.}
The main cohort in Customer Service comprises 14 models: the 12 models that belong to the main cohort in every domain, together with Grok~4.6 and Fable~5.1.
% src: data/customer_service_cells.csv main_cohort (14 True); data/tables_key_numbers.json scorecard.main_n.customer_service
The five remaining GPT packages are score-only deliveries without transcripts or item-level judgments, and the Claude Opus~5.5 package mixes GPT-5.6 Sol at high effort and GPT-6 Luna at medium effort across conversations (Appendix~\ref{app:cohort}).
% src: data/customer_service_cells.csv notes (score-only delivery; per-episode support configurations for Claude Opus 5.5)

\subsection{Persona Bank and Needs}
\label{app:service-personas}

\paragraph{Cards.}
Each of the eight cards perturbs one attribute from a shared set of common user attributes, adapted to customer service, and describes behavior rather than adjectives (\tabref{tab:service-personas}).
The neutral condition is an empty card.
Customer Service is the only domain whose persona bank has recorded human selection decisions: the domain owner retained all eight cards after reading two conversations per card, whereas in the other domains selection is pending.
% src: output/panels/customer_service/persona.json (needs; selection status retain); customer-service-benchmark/eval/personas.json (critical flags)

\paragraph{Needs and criticality.}
Seven cards carry one critical need, and the frustrated-on-refusal card also carries a non-critical need to have the frustration acknowledged.
The gives-up-early card has no need, because it changes what the customer does after a refusal, and its effect is read from the native task grade alone.

\begin{table}[!tb]
% src: data/persona_effects.csv (domain=customer_service, main_cohort=True); data/customer_service_needs.csv (population=valid_completed) needs_expressed_rate; data/customer_service_episodes.csv.gz audit_status, failure_bucket; output/panels/customer_service/persona.json
\centering\footnotesize\setlength{\tabcolsep}{3pt}\renewcommand{\arraystretch}{1.15}
\begin{tabularx}{\linewidth}{@{}>{\raggedright\arraybackslash}p{3.0cm}>{\raggedright\arraybackslash}Xrrrrrrrr@{}}
\toprule
Condition & Critical need & Expr. & Needs & Inv. & End & Compl. & $\Delta$ & Below & Above \\
\midrule
Neutral & none & -- & -- & 0.5 & 1.3 & 72.5 & -- & -- & -- \\
P2: Frustrated on refusal & reason and recourse after a refusal & 75.9 & 87.9 & 9.9 & 1.9 & 72.1 & $-$0.5 & 1 & 0 \\
C2: Self-doubt & facts checked against the record & 55.8 & 37.1 & 1.5 & 1.0 & 73.2 & $+$0.7 & 0 & 0 \\
C3: Gives up early & none (behavior only) & -- & -- & 6.3 & 7.7 & 65.3 & $-$7.2 & 7 & 0 \\
A03: Money matters & exact amount and timing & 61.7 & 62.0 & 9.3 & 2.5 & 71.8 & $-$0.7 & 2 & 1 \\
A09: Wants the reason & rule behind the outcome & 99.8 & 75.3 & 6.7 & 9.0 & 65.1 & $-$7.5 & 7 & 0 \\
A10: Bundles questions & every question answered & 100.0 & 63.7 & 14.4 & 3.4 & 67.9 & $-$4.6 & 4 & 0 \\
A11: Risk-sensitive & side effects explained & 97.5 & 78.5 & 1.5 & 5.9 & 68.8 & $-$3.8 & 2 & 0 \\
A12: Wants options & options offered & 94.1 & 77.9 & 8.8 & 3.9 & 70.8 & $-$1.8 & 1 & 0 \\
\bottomrule
\end{tabularx}
\captionsetup{position=bottom}
\caption{\textbf{Customer Service persona conditions in the main cohort.}
Numeric columns other than \emph{Inv.}, \emph{Below} and \emph{Above} are unweighted means of per-model values over the 14 main-cohort models, in percent except $\Delta$.
\emph{Expr.}: share of pre-recorded needs expressed, among simulator-valid completed conversations.
\emph{Needs}: persona-needs score.
\emph{Inv.}: invalid share of audited conversations, pooled over the main cohort.
\emph{End}: share of planned conversations that failed only because of the ending.
\emph{Compl.}: task completion over graded completed conversations, the population of the persona-effect estimates; the neutral row covers all three neutral trials.
$\Delta$: paired persona-minus-neutral change in completion, in percentage points, over 130 to 132 items per model, against the item's mean over its graded neutral trials, up to three, of which only the first shares the persona conditions' first reply.
\emph{Below}/\emph{Above}: number of models whose 95\% task-cluster bootstrap interval lies entirely below or above zero.
Following the domain's reporting rule, persona conditions are not pooled.}
\label{tab:service-personas}
\end{table}

\subsection{Native Task Grade, Persona-Needs Score and Simulator Audit}
\label{app:service-grading}

\paragraph{Native task grade.}
The native task grade is rule-based task completion.
A conversation is complete when the agent reached the policy-correct decision, made every required look-up before deciding, executed tools that match the decision, entered no wrong membership tier, verified the customer's identity where required, and reached the ending that the policy class requires.
For example, under a policy that allows escalation after a refusal, closing the case and entering the escalation after a correct refusal are both complete endings, whereas an escalation that is promised but never entered is not; under a policy that requires escalation, every escalation step must have run.
The rules read tool calls first and wording second, and an LLM task judge provides a cross-check that does not enter the headline.
The headline population is all planned conversations, and a conversation that failed to finish counts as not complete.
% src: data/domain_facts.json domains.customer_service.task_metric, task_population; data/cells.csv task_population (domain=customer_service)
Every incomplete graded conversation falls into exactly one of three failure types, tested in order: a wrong decision; a process gap, in which the decision was right but a required look-up came after it or the execution did not match; and a wrong ending.

\paragraph{Persona-needs score.}
Each pre-recorded need is scored 1, $\tfrac12$ or 0 when the customer expressed it and the agent had a chance to answer, and the persona pass requires every critical need to be met.
The persona-needs score of a model is the mean over simulator-valid completed persona conversations with a numeric needs score; the needs judge sees the conversation without tool lines and never sees the policy or the correct outcome.
% src: data/domain_facts.json domains.customer_service.needs_metric, needs_scope; data/cells.csv needs_population (domain=customer_service)

\paragraph{Simulator audit.}
The audit returns valid, invalid or uncertain with quoted evidence.
It does not change the task headline, which covers all planned conversations, but invalid and uncertain conversations leave the needs population.
% src: data/domain_facts.json domains.customer_service.audit, audit_filters_headline (needs score uses valid episodes)
In the main cohort, the valid share of audited completed conversations ranged from 92.6\% for Muse Glimmer 30B to 95.6\% for Qwen~3.8 Flash.
% src: data/cells.csv sim_valid_rate (domain=customer_service, main_cohort=True): Muse Glimmer 30B 1344/1452 = 0.9256, Qwen 3.8 Flash 1388/1452 = 0.9559
Invalid verdicts concentrated in some cards: pooled over the main cohort, 14.4\% of audited conversations of the customer who bundles questions were invalid, against 0.5\% for the neutral condition (\tabref{tab:service-personas}).
% src: data/customer_service_episodes.csv.gz audit_status by condition, main cohort pooled (A10_uncertainty_low 264/1838; neutral 30/5542)

\subsection{Per-Model Results}
\label{app:service-results}

\input{tables/domain_customer_service}

\paragraph{Task.}
\tabref{tab:domain-customer-service} reports every model.
In the main cohort, task completion ranged from 22.7\% for MiniMax~M3 to 94.1\% for Gemini~3.8 Flash, followed by Gemini~3.7 Flash at 92.6\%.
% src: data/cells.csv task_value (domain=customer_service, main_cohort=True)
The policy decision alone was correct in 90.8\% to 97.4\% of planned conversations for 12 of the 14 models, so most of the variation in completion among them lies in the process and the ending rather than in the decision.
% src: tables/domain_customer_service.tex Decision column (main cohort; Kimi K3 90.8 to Grok 4.6 97.4; exceptions Muse Glimmer 30B 52.9, MiniMax M3 82.2)
MiniMax~M3, which ran with reasoning disabled, had the most process gaps, 836 conversations, followed by GLM~5.3 Flash with 492 and Qwen~3.8 Flash with 433.
% src: data/customer_service_cells.csv process_gap (MiniMax M3 836, GLM 5.3 Flash 492, Qwen 3.8 Flash 433); thinking off
Muse Glimmer 30B had the lowest decision accuracy, 52.9\%, for the reason described in Appendix~\ref{app:service-caveats}.
% src: data/cells.csv outcome_correct_value (Muse Glimmer 30B 0.529)

\paragraph{Needs.}
Persona-needs scores ranged from 47.5\% for Muse Glimmer 30B to 80.2\% for Fable~5.1, and the persona pass rate from 32.8\% to 66.3\%.
% src: data/cells.csv needs_value, persona_pass_rate (domain=customer_service, main_cohort=True)
Task completion and needs score were positively associated across the main cohort, $\rho=0.54$ ($n=14$, $p=0.048$).
% src: data/task_vs_needs.csv customer_service main_cohort spearman_rho=0.5429, spearman_p_perm=0.0481

\subsection{Persona Effects}
\label{app:service-effects}

\paragraph{Direction and consistency.}
Two cards lowered completion, measured over graded completed conversations, by more than 7 percentage points on average (\tabref{tab:service-personas}).
The customer who wants the reason behind the outcome lowered completion by 7.5 percentage points, and the customer who gives up early by 7.2; for each, the interval lay below zero for seven of the 14 main-cohort models.
% src: data/persona_effects.csv customer_service A09_depth_high (mean -0.0747; below 7), C3_give_up_early (mean -0.0721; below 7)
The customer who bundles questions lowered completion by 4.6 percentage points, with intervals below zero for four models, and the risk-sensitive customer by 3.8, with two such models.
% src: data/persona_effects.csv customer_service A10_uncertainty_low (mean -0.0463; below 4), A11_risk_high (mean -0.0377; below 2)
The frustrated, self-doubting, money-conscious and option-seeking customers changed completion by less than 2 percentage points on average.
% src: data/persona_effects.csv customer_service P2, C2, A03, A12 main-cohort mean deltas (-0.5, +0.7, -0.7, -1.8)
Following the domain's reporting rule, the cards are not pooled, because cards can move completion in opposite directions on the same items.
% src: customer-service-benchmark/eval/METRICS.md (rule: completion is never pooled across personas) -- benchmark checkout

\paragraph{Mechanism: the ending.}
The two largest decreases are associated mainly with how conversations end rather than with the decision.
Averaged over the main cohort, 1.3\% of planned neutral conversations failed only because of a wrong ending, against 9.0\% for the customer who wants the reason, 7.7\% for the customer who gives up early and 5.9\% for the risk-sensitive customer.
% src: data/customer_service_episodes.csv.gz failure_bucket=wrong_ending by condition, per-model share of planned episodes averaged over 14 main-cohort models
The share of wrong decisions changed much less, from 8.3\% for the neutral condition to between 7.7\% and 11.5\% for the cards, the largest being for the customer who gives up early.
% src: data/customer_service_episodes.csv.gz failure_bucket=wrong_decision by condition, same aggregation
Process gaps ranged from 15.5\% to 20.3\% across the cards, against 17.9\% for the neutral condition.
They were most frequent for the customer who bundles questions, for whom they rose about as much as wrong endings did.
% src: data/customer_service_episodes.csv.gz failure_bucket=process_gap by condition, same aggregation (C3 15.48, A10 20.35, neutral 17.947; A10 wrong_ending 3.41 vs neutral 1.28)
A wrong ending arises, for example, when the customer leaves before a required callback number is taken, when an offered escalation is accepted but never entered, or when the agent hands off a case that the policy does not allow it to hand off.
The customer who gives up early leaves at the first refusal, before a required escalation can be entered; the customers who keep asking why or what could go wrong extend the conversation after the decision, which may create more occasions to promise an escalation without entering it.
We did not attribute each failed conversation to a single cause.

\paragraph{Needs by persona.}
The self-doubting customer had the lowest needs score, 37.1\%: the need requires the agent to check the record and state what it shows, rather than accept the customer's self-correction, and in most scored conversations the agent did not do so.
% src: data/persona_effects.csv customer_service C2_self_doubt needs_value (main-cohort mean 0.371); data/customer_service_needs.csv C2_self_doubt (population=valid_completed: satisfied 316, partial 57, not satisfied 562, main cohort)
The customer who bundles questions expressed its need in every simulator-valid completed conversation but had a needs score of 63.7\%; most of its scored needs were only partially satisfied, which suggests that the agent answered some, but not all, of the questions bundled in a message.
% src: data/customer_service_needs.csv A10_uncertainty_low (population=valid_completed) needs_expressed_rate=1.000, satisfied 583, partial 803, not satisfied 155 (main cohort); data/persona_effects.csv needs_value mean 0.637

\subsection{Domain-Specific Failures and Caveats}
\label{app:service-caveats}

\paragraph{Generation failures.}
Grok~4.6, Kimi~K3 and DeepSeek~V4.1 Flash had six, seven and four conversations, respectively, that stopped with an agent or simulator error, and GPT-5.6 Sol, outside the main cohort, had four; they count as incomplete in the headline.
% src: data/failures.csv customer_service (Grok 4.6 other 6; Kimi K3 other 4 + simulator_error 3; DeepSeek V4.1 Flash other 4; GPT-5.6 Sol tool/transport 4); data/customer_service_episodes.csv.gz terminal_state agent_error (GPT-5.6 Sol 4)

\paragraph{Muse Glimmer 30B and the tool marker.}
Muse Glimmer 30B often announced a look-up in prose, for example by saying that it would pull up the account, and ended its turn without writing the bracketed tool marker that the protocol requires.
In 660 of its 1,452 conversations it made no tool call at all, whereas every other model with rule-level records had between zero and nine such conversations.
% src: data/muse_tool_diagnosis.md section 1 (660/1,452; other 17 models with native rule fields 0-9; Gemini packages not comparable)
Across its 16,427 assistant turns, 5,186 announced an action without a marker, against 142 of the 11,608 turns of Qwen~3.8 27B, which was served through the same local path.
% src: data/muse_tool_diagnosis.md section 3 (5,186 of 16,427 = 31.6%; Qwen 3.8 27B 142 of 11,608 = 1.2%)
The behavior did not appear to depend on the persona: 154 of the 396 neutral conversations and 409 of the 1,056 persona conversations ended with an unclear outcome and no tool call.
% src: data/muse_tool_diagnosis.md section 1
The shared first reply appears to have propagated it: when the shared reply contained a marker, none of the 293 following conversations lacked a tool call, whereas when it only announced an action, 310 of 431 did.
% src: data/muse_tool_diagnosis.md section 3 (0/293; 310/431 = 71.9%)
Token accounting against the local serving logs shows that, apart from at most about 1.6\% of calls, the visible replies are the model's complete answer-channel output.
% src: data/muse_tool_diagnosis.md section 4
The low completion of Muse Glimmer 30B therefore reflects model behavior under the shared text-marker protocol rather than a serving artifact.
Native function calling was not tested.
Among the conversations of Muse Glimmer 30B with at least one tool call, completion was 65.2\%, against 71.3\% for Qwen~3.8 27B over all of its conversations.
% src: data/muse_tool_diagnosis.md section 1 (516/792 = 65.2%; Qwen 3.8 27B 1,035/1,452 = 71.3%)

\paragraph{Output budgets and judge policy.}
For the two locally served models, the local router raised the native tested-model cap of 6,000 tokens to 65,536 and gave every GPT-6 Luna support call at least 8,192 output tokens, whereas the native support budgets are 500 to 1,200 tokens (Appendix~\ref{app:local-serving}).
% src: data/customer_service_cells.csv notes (Qwen 3.8 27B, Muse Glimmer 30B)
In the GPT-6 Luna cell, 31 completed persona conversations have no needs judgment and 17 completed conversations have no simulator audit, and in the Kimi~K3 cell 27 and 7, respectively; these conversations are excluded from the needs score.
% src: data/customer_service_cells.csv GPT-6 Luna notes (31 / 17) and Kimi K3 notes (27 / 7)

\paragraph{Self-judging.}
In the GPT-6 Luna cell, the tested agent is also the customer simulator and every judge, which is a self-evaluation caveat for its needs score~\citep{panickssery2024selfpreference}.
