# Supplementary material for: PersonaChatBench: Evaluating Chat Assistants with Diverse Simulated Users
Source: arXiv:2610.42060 source file (2026-10-30)
Supplement: Supplementary file 16 [file travel.tex]

% Travel domain appendix. Every number is taken from data/ in this repository;
% protocol facts follow the benchmark checkout listed in data/domain_facts.json.
% Main cohort only for comparisons; marked configurations are described as such.

The Travel domain evaluates a tested assistant that acts as a travel agent with search and selection tools in conversations with a simulated traveler who holds the trip preferences.
It retains the official tasks, catalogs and choice rewards of the Travel-44 environment of UserBench~\citep{qian2025userbench} and adds five authored tasks in which the traveler revises a requirement during the conversation; the scores are a protocol adaptation and not a reproduction of the original UserBench leaderboard.
What varies is how the traveler wants to decide: step by step or efficiently, with plain explanations or detailed comparisons, and with support or evidence.

\subsection{Source and Task Panel}
\label{app:travel-panel}

\paragraph{Task panel.}
The panel contains the 67 official test tasks of UserBench Travel-44 and five authored revision tasks.
% src: data/tables_key_numbers.json domains.travel.tasks_by_kind (userbench 67, manual_revision 5); data/domain_facts.json domains.travel.sources
Each official task asks for two travel aspects, such as a flight and a hotel, and the traveler holds several preferences for each.
The catalogs are the synthetic source catalogs: every correct option, up to 10 wrong options and up to five noise options, shuffled deterministically and stripped of their hidden labels.
Because the panel is the complete official test split, it is not selected on model outcomes.
The authored tasks cover a change of departure time, hotel budget, party size or objective priority, and the revocation of an earlier change; they use small catalogs and are not intended to be difficult.

\paragraph{Tools.}
The assistant acts through typed actions: a search returns the complete source catalog for an aspect, a reply speaks to the traveler, and a choice commits one option for an aspect.
On official tasks, each aspect can be committed only once; the commitment is final and returns only a neutral receipt.
% src: travel-benchmark/README.md (native once-per-aspect final commitment; neutral receipt) and engine.py (an aspect's single final choice cannot be revised) -- benchmark checkout
On authored tasks, a choice is a replaceable recommendation, and a predeclared revision event enters the conversation only when the simulated traveler chooses to raise it after a recommendation.

\paragraph{Roles and protocol.}
Each task is run once under five persona conditions and once under the neutral condition, which gives 432 planned conversations per model.
% src: data/tables_key_numbers.json domains.travel (persona_conditions=5, neutral_trials=1, episodes_per_model=432)
The source opening is used verbatim, and every condition of a task reuses the shared first reply together with any preceding tool results and choice state.
Natural persona conversations replace the scheduled preference reveals of the original environment.
A conversation ends when the traveler stops or after 10 assistant replies; tool steps are capped separately.
% src: data/domain_facts.json domains.travel.turn_cap=10, turn_cap_unit
The assistant sees the opening, its own actions and the catalog results; the traveler sees only its authorized preferences, its persona card and the public dialogue, and never sees the correct options or the grading rules.

\paragraph{Cohort.}
The main cohort in Travel comprises 19 models: every tested model except Claude Opus~5.5, whose simulator and judges were GPT-5.6 Sol at high effort.
% src: data/travel_cells.csv main_cohort (19 True); data/tables_key_numbers.json scorecard.main_n.travel

\subsection{Persona Bank and Needs}
\label{app:travel-personas}

\paragraph{Cards.}
The persona bank uses three binary axes: a stepwise or efficient decision pace, an explanation depth of plain language or comparative detail, and a trust style that seeks support or evidence.
Five of the eight combinations were prespecified as cards: the careful planner, the skeptical comparer and the concise decider from an earlier pilot, and the efficient comparer and the concise planner, added in a later revision of the bank (\tabref{tab:travel-personas}).
The cards are neither exhaustive nor randomly sampled.
All five cards passed automated screening, and human selection is pending.
% src: output/panels/travel/persona.json (dimensions, needs, screening eligible, selection pending); travel-benchmark/data/personas.json (critical flags)

\paragraph{Needs and criticality.}
Each card carries three needs, two of them critical, and every need is phrased as a response to an explicit request, for example handling one aspect at a time, comparing a proposed option with an alternative, or giving a brief reason and a chance to respond before an irrevocable selection.
Applicability and criticality are frozen per task kind before the shared first reply; for example, a single-aspect authored task cannot test pacing between aspects.
The neutral traveler has no card and no needs.

\begin{table}[!tb]
% src: data/persona_effects.csv (domain=travel, main_cohort=True); data/travel_needs.csv needs_expressed_rate (19 main-cohort models; the file has no main_cohort column, so Claude Opus 5.5 is dropped); data/travel_episodes.csv.gz (task_kind=userbench, task_score not null: task_score==0 share and assistant_turns, per-model means averaged); output/panels/travel/persona.json; travel-benchmark/data/personas.json
\centering\footnotesize\setlength{\tabcolsep}{3pt}\renewcommand{\arraystretch}{1.15}
\begin{tabularx}{\linewidth}{@{}>{\raggedright\arraybackslash}p{2.3cm}>{\raggedright\arraybackslash}Xrrrrrrrr@{}}
\toprule
Condition & Needs (critical in italics) & Expr. & Needs & Zero & Turns & Reward & $\Delta$ & Below & Above \\
\midrule
Neutral & none & -- & -- & 12.6 & 3.53 & 73.4 & -- & -- & -- \\
Careful planner & \emph{paced questions}; \emph{plain terms}; recap before committing & 53.6 & 94.5 & 19.9 & 4.72 & 62.8 & $-$10.4 & 13 & 0 \\
Skeptical comparer & \emph{comparison}; \emph{price breakdown}; facts versus assumptions & 98.8 & 97.9 & 33.5 & 4.14 & 49.5 & $-$24.1 & 19 & 0 \\
Concise decider & \emph{concise}; \emph{answer first}; reason before committing & 34.7 & 64.8 & 21.1 & 4.23 & 56.8 & $-$16.7 & 16 & 0 \\
Efficient comparer & \emph{comparison}; \emph{answer first}; facts versus assumptions & 66.0 & 96.9 & 21.7 & 3.79 & 60.1 & $-$13.3 & 13 & 0 \\
Concise planner & \emph{concise}; \emph{plain terms}; recap before committing & 8.2 & 88.6 & 12.9 & 3.83 & 72.0 & $-$1.4 & 3 & 2 \\
\midrule
All personas pooled & & 51.0 & 88.6 & -- & -- & 60.2 & $-$13.1 & 16 & 0 \\
\bottomrule
\end{tabularx}
\captionsetup{position=bottom}
\caption{\textbf{Travel persona conditions in the main cohort.}
Numeric columns other than \emph{Below} and \emph{Above} are unweighted means of per-model values over the 19 main-cohort models, in percent except \emph{Turns} and $\Delta$.
\emph{Expr.}: share of applicable needs expressed.
\emph{Needs}: persona-needs score.
\emph{Zero}: share of scored official-task conversations with zero choice reward.
\emph{Turns}: mean assistant replies in scored official-task conversations.
\emph{Reward}: choice reward on official tasks.
$\Delta$: paired persona-minus-neutral change in choice reward, in points on the 0--100 scale, over 47 to 67 official tasks per model.
\emph{Below}/\emph{Above}: number of models whose 95\% task-cluster bootstrap interval lies entirely below or above zero.
Pooled row: each model's persona conditions combined into one paired contrast.}
\label{tab:travel-personas}
\end{table}

\subsection{Native Task Grade, Persona-Needs Score and Simulator Audit}
\label{app:travel-grading}

\paragraph{Native task grade.}
On official tasks, a committed option earns 1 if it is the best option for the aspect, 0.8 if it is another correct option and 0 if it is wrong, and the native task grade, the choice reward, is the mean over the two requested aspects.
An aspect that was never committed earns 0, so a conversation that ends before the assistant commits scores 0 for that aspect.
% src: data/domain_facts.json domains.travel.task_metric (1 / 0.8 / 0 per aspect); tables/domain_travel.tex caption
The headline is the mean reward over all recorded official-task conversations with a score, including the neutral condition; conversations that end at a cap or with an error have no primary score and are not imputed.
% src: data/domain_facts.json domains.travel.task_metric, task_population; data/cells.csv task_population (domain=travel)
The authored revision tasks are scored separately by final-state success, that is, whether the last recommendation is optimal under the latest public requirements, and are never pooled with the reward.

\paragraph{Persona-needs score.}
A need earns 1, $\tfrac12$ or 0 only when the traveler expressed it and the assistant had a chance to answer, with exact quotations validated against the transcript.
The persona-needs score of a model is the mean over persona conversations, on official and authored tasks, with at least one expressed and answered need.
The persona pass is true when every applicable critical need was expressed, answered and satisfied, false when an answered critical need was partially satisfied or unmet, and unknown otherwise.
% src: data/domain_facts.json domains.travel.needs_metric, needs_scope; data/cells.csv needs_population (domain=travel)

\paragraph{Simulator audit.}
The audit returns valid, invalid or uncertain and does not filter the headline; \tabref{tab:domain-travel} also reports the reward over simulator-valid completed conversations, which differs little from the headline.
% src: data/domain_facts.json domains.travel.audit, audit_filters_headline=false; tables/domain_travel.tex Valid only column
Pooled over the main cohort, the invalid share of audited conversations was between 6.8\% and 9.1\% in every persona condition and 7.0\% for the neutral condition, so invalid verdicts did not concentrate in particular personas.
% src: data/travel_episodes.csv.gz audit_status by condition, main cohort pooled

\subsection{Per-Model Results}
\label{app:travel-results}

\input{tables/domain_travel}

\paragraph{Task and needs.}
\tabref{tab:domain-travel} reports every model.
In the main cohort, the choice reward ranged from 38.4 for MiniMax~M3 to 86.6 for Gemini~3.7 Flash, followed by Fable~5.1 at 79.7 and Claude Sonnet~5.5 at 79.3.
% src: data/cells.csv task_value (domain=travel, main_cohort=True)
Persona-needs scores lay in a narrower range, from 84.2\% for Claude Sonnet~5.5 to 94.0\% for GPT-6 Astra, and the persona pass rate over conversations with a decided pass ranged from 64.7\% for MiniMax~M3 to 95.9\% for GPT-6 Astra.
% src: data/cells.csv needs_value (domain=travel, main_cohort=True); tables/domain_travel.tex Pass column
Travel is the only domain in which task and needs were significantly negatively associated across the main cohort, $\rho=-0.63$ ($n=19$, $p=0.005$).
% src: data/task_vs_needs.csv travel main_cohort spearman_rho=-0.6263, spearman_p_perm=0.0051
The authored revision tasks did not separate most models: 14 of the 19 main-cohort models succeeded on all 30 of their revision conversations.
% src: data/travel_cells.csv revision_num/revision_den (main cohort; 14 models at 30/30)

\paragraph{Commitment and reward.}
Across models, the reward tracks mainly whether the assistant commits an option at all.
The share of official-task aspects that remained uncommitted ranged from 7.5\% for Gemini~3.7 Flash to 59.5\% for MiniMax~M3 and was almost perfectly negatively correlated with the reward across the main cohort, $r=-0.99$ ($n=19$, $p<0.001$); this association holds largely by construction, because an uncommitted aspect earns no reward.
% src: data/previews/mechanisms_values.csv (panel_domain=travel, x_noncommit, main cohort); data/previews/mechanisms_stats.csv panel b, travel, main_cohort (pearson_r=-0.9907, p_perm=0.0001); travel-benchmark/README.md (a naturally terminated missing choice contributes 0) -- benchmark checkout
When an option was committed, it earned between 83.8\% and 95.5\% of the available credit for every main-cohort model.
% src: data/previews/mechanisms_values.csv committed_credit_pct (main cohort; GPT-5.5 83.8 to Gemini 3.8 Flash 95.5)
Models that leave more aspects open, for example while they ask, compare or confirm, therefore lose reward, and they tend to score higher on needs that ask for exactly that behavior: the uncommitted share was positively correlated with the persona-needs score, $r=0.61$ ($n=19$, $p=0.006$), which is consistent with the negative association between the two grades (\figref{fig:mechanisms}).
% src: data/previews/mechanisms_stats.csv supp, travel, x_noncommit vs needs_value, main_cohort (pearson_r=0.6078, p_perm=0.0057)

\subsection{Persona Effects}
\label{app:travel-effects}

\paragraph{Direction and consistency.}
Four persona conditions lowered the choice reward consistently relative to the neutral condition, whereas the concise planner left it almost unchanged (\tabref{tab:travel-personas}).
The skeptical comparer lowered it by 24.1 points on average, and the interval lay below zero for all 19 main-cohort models.
% src: data/persona_effects.csv travel skeptical_comparer (mean -0.2412; below 19 of 19)
The concise decider, the efficient comparer and the careful planner lowered it by 16.7, 13.3 and 10.4 points, with intervals below zero for 16, 13 and 13 models.
% src: data/persona_effects.csv travel concise_decider (-0.1670; 16), efficient_comparer (-0.1333; 13), careful_planner (-0.1043; 13)
Pooled over the five personas, the reward fell by 13.1 points, with intervals below zero for 16 of the 19 models.
% src: data/persona_effects.csv travel all_personas (mean -0.1314; below 16)

\paragraph{Mechanism: asking before committing.}
The personas' requests for comparisons, price breakdowns, recaps or a reason before an irrevocable selection are associated with longer conversations in which the assistant discusses options instead of committing them; when the traveler then stops, the uncommitted aspects earn nothing.
Persona conversations had more assistant replies than neutral ones, 3.79 to 4.72 against 3.53, and a larger share of official-task conversations with zero reward, up to 33.5\% for the skeptical comparer against 12.6\% for the neutral condition.
% src: data/travel_episodes.csv.gz (task_kind=userbench) assistant_turns and task_score==0 by condition, per-model shares averaged over 19 main-cohort models
Almost all zero-reward conversations lacked a full commitment rather than containing a wrong choice: pooled over the main cohort, 1,497 of the 1,501 zero-reward official-task conversations left at least one aspect uncommitted, and 1,407 committed nothing.
% src: data/travel_episodes.csv.gz (main cohort, task_kind=userbench, task_score==0) joined by episode_id with output/results/travel/*/{data,evidence}.jsonl.gz episode.choices (number of committed aspects vs aspects in task_id) -- benchmark checkout
The concise planner, which expressed only 8.2\% of its applicable needs and at least one need in 14.1\% of its needs-judged conversations, behaved much like the neutral traveler and left the reward almost unchanged.
% src: data/travel_needs.csv concise_planner needs_expressed_rate (mean 0.082) and episode_expressed_rate (mean 0.141), main cohort
The decrease was largest for the persona that voiced its requests most often and nearly absent for the persona that rarely voiced them, which is consistent with reading the Travel persona effect as a change in what the user leaves with rather than in the quality of the assistant's choices.
% src: data/travel_needs.csv needs_expressed_rate (skeptical_comparer 0.988 highest, concise_planner 0.082 lowest); data/persona_effects.csv delta_vs_neutral_task (-0.241 largest, -0.014 smallest)

\paragraph{Needs by persona.}
The skeptical comparer and the efficient comparer had the highest needs scores, 97.9\% and 96.9\%, even though their reward decreases were among the largest.
% src: data/persona_effects.csv travel needs_value, main-cohort mean per condition
The concise decider had the lowest needs score, 64.8\%: its needs ask for compact replies that lead with a recommendation, which the assistants met less often than the requests for comparisons or explanations.
% src: data/persona_effects.csv travel concise_decider needs_value (main-cohort mean 0.648); data/travel_needs.csv concise_decider (satisfied 721, partial 301, not satisfied 314)
The needs score of the concise planner rests on few conversations, 189 across the 19 models, because its needs were rarely expressed.
% src: data/persona_effects.csv travel concise_planner needs_n summed over main cohort = 189

\subsection{Domain-Specific Failures and Caveats}
\label{app:travel-caveats}

\paragraph{Generation failures.}
Muse Glimmer 30B had 38 failures: 24 empty outputs, in which the model ended its turn inside the reasoning channel before the constrained answer channel opened; three choices without the required public explanation; eight conversations stopped at the reply cap; and three stopped at the tool cap.
% src: data/failures.csv travel Muse Glimmer 30B (empty_answer 24, protocol/format 3, turn_cap 8, tool_cap 3); data/travel_cells.csv notes; data/muse_tool_diagnosis.md section 5
Unlike in Customer Service, Travel actions are enforced by a schema rather than written as text markers, and the share of scored official-task conversations without any choice was 23.6\% for Muse Glimmer 30B, within the range of the API-served main-cohort models, 2.2\% to 47.3\%.
% src: data/muse_tool_diagnosis.md section 5 (Muse 86/364 = 23.6%); range recomputed from data/travel_episodes.csv.gz (main cohort, userbench, task_score not null) joined with output/results/travel/*/{data,evidence}.jsonl.gz episode.choices (Claude Sonnet 5.5 and Gemini 3.7 Flash 2.2%, MiniMax M3 47.3%) -- benchmark checkout
MiniMax~M3 had 66 failures, 61 of them model or protocol errors without a recorded reason and five conversations at the reply cap.
% src: data/failures.csv travel MiniMax M3 (other 61, turn_cap 5)
Two packages regenerated failed conversations: the first pass of GLM~5.3 Flash ended with eight error conversations and that of Qwen~3.8 Flash with seven, and the runner's resume option archived and regenerated these conversations at the unchanged 10,000-token cap.
% src: output/results/travel/{glm-5-3-flash,qwen-3-8-flash}/*/manifest.json resume (original_pass error 8 / 7; mechanism run.py run --resume --retry-errors; pre_resume_episodes_archived true) -- benchmark checkout; data/travel_cells.csv repaired_judges
Capped conversations have no primary score; GPT-5.6 Sol had six and GPT-6 Astra four of them.
% src: data/failures.csv travel turn_cap (GPT-5.6 Sol 6, GPT-6 Astra 4)

\paragraph{Output budgets and judge policy.}
The tested-model output budget was 8,192 tokens for the two Gemini packages, GPT-5.5, GPT-5.6 Sol, GPT-5.6 Terra, GPT-6 Astra, GPT-6 Sol and the Claude Haiku~5.5, Claude Sonnet~5.5 and Claude Opus~5.5 packages, 10,000 tokens for GLM~5.3 Flash and Qwen~3.8 Flash, and 65,536 tokens for the two locally served models and Fable~5.1; it is not recorded in five packages (Appendix~\ref{app:config}).
% src: data/travel_cells.csv output_budget_tokens (NA for GPT-6 Luna, Grok 4.6, Kimi K3, MiniMax M3, DeepSeek V4.1 Flash)
For the two Gemini models, the headline uses the original validated needs judgments; the raw-judge score update in their packages changes the needs score of 38 and 33 conversations and leaves every task score and audit unchanged.
% src: data/travel_cells.csv Gemini 3.7 / 3.8 Flash notes (0 task-score, 0 audit and 38 / 33 persona needs-score differences)
The caption of \tabref{tab:domain-travel} gives the alternative values, and Appendix~\ref{app:judge-policy} the needs populations under both policies.
The Claude Haiku~5.5 and Claude Sonnet~5.5 packages include a published evaluation catch-up on 32 and 29 conversations.
% src: data/travel_cells.csv repaired_judges (Claude Haiku 5.5 32, Claude Sonnet 5.5 29)

\paragraph{Self-judging.}
In the GPT-6 Luna cell, the tested agent is also the traveler simulator and every judge, which is a self-evaluation caveat for its needs score~\citep{panickssery2024selfpreference}.
