# Supplementary material for: PersonaChatBench: Evaluating Chat Assistants with Diverse Simulated Users
Source: arXiv:2610.42060 source file (2026-10-30)
Supplement: Supplementary file 17 [file appendix.tex]

% Appendix tables inherit the caption font of main.tex; every appendix table,
% generated or hand-written, places its caption below the tabular.
\captionsetup[table]{position=bottom}

% Appendix contents: every section and subsection;
% titles come from the headings themselves through \nameref.
\providecommand{\appcontentsentry}[2]{%
\par\begingroup\leftskip=#1\relax\rightskip=2.2em plus 1fil\parfillskip=-\rightskip
\hangindent=2.6em\hangafter=1\noindent
\makebox[2.6em][l]{\ref*{#2}}\nameref*{#2}\nobreak
\leaders\hbox{$\mkern4.5mu\hbox{.}\mkern4.5mu$}\hfill\nobreak\hbox to 2.2em{\hss\pageref*{#2}}\par\endgroup}
\section*{Appendix Contents}
\begingroup
\small\setstretch{1.0}\setlength{\parskip}{1.5pt plus 0.5pt}
\begin{multicols}{2}
\appcontentsentry{0em}{app:protocol}
\appcontentsentry{1em}{app:statuses}
\appcontentsentry{1em}{app:prompts}
\appcontentsentry{1em}{app:cards}
\appcontentsentry{1em}{app:records}
\appcontentsentry{0em}{app:runs}
\appcontentsentry{1em}{app:config}
\appcontentsentry{1em}{app:cohort}
\appcontentsentry{1em}{app:coverage}
\appcontentsentry{1em}{app:judge-policy}
\appcontentsentry{1em}{app:local-serving}
\appcontentsentry{1em}{app:rank-sensitivity}
\appcontentsentry{0em}{app:health}
\appcontentsentry{1em}{app:health-panel}
\appcontentsentry{1em}{app:health-personas}
\appcontentsentry{1em}{app:health-grading}
\appcontentsentry{1em}{app:health-results}
\appcontentsentry{1em}{app:health-effects}
\appcontentsentry{1em}{app:health-caveats}
\appcontentsentry{0em}{app:coding}
\appcontentsentry{1em}{app:coding-panel}
\appcontentsentry{1em}{app:coding-personas}
\appcontentsentry{1em}{app:coding-grading}
\appcontentsentry{1em}{app:coding-results}
\appcontentsentry{1em}{app:coding-effects}
\appcontentsentry{1em}{app:coding-caveats}
\appcontentsentry{0em}{app:math}
\appcontentsentry{1em}{app:math-panel}
\appcontentsentry{1em}{app:math-personas}
\appcontentsentry{1em}{app:math-grading}
\appcontentsentry{1em}{app:math-results}
\appcontentsentry{1em}{app:math-effects}
\appcontentsentry{1em}{app:math-caveats}
\appcontentsentry{0em}{app:finance}
\appcontentsentry{1em}{app:finance-panel}
\appcontentsentry{1em}{app:finance-personas}
\appcontentsentry{1em}{app:finance-grading}
\appcontentsentry{1em}{app:finance-results}
\appcontentsentry{1em}{app:finance-effects}
\appcontentsentry{1em}{app:finance-caveats}
\appcontentsentry{0em}{app:service}
\appcontentsentry{1em}{app:service-panel}
\appcontentsentry{1em}{app:service-personas}
\appcontentsentry{1em}{app:service-grading}
\appcontentsentry{1em}{app:service-results}
\appcontentsentry{1em}{app:service-effects}
\appcontentsentry{1em}{app:service-caveats}
\appcontentsentry{0em}{app:travel}
\appcontentsentry{1em}{app:travel-panel}
\appcontentsentry{1em}{app:travel-personas}
\appcontentsentry{1em}{app:travel-grading}
\appcontentsentry{1em}{app:travel-results}
\appcontentsentry{1em}{app:travel-effects}
\appcontentsentry{1em}{app:travel-caveats}
\appcontentsentry{0em}{app:cases}
\appcontentsentry{1em}{app:case-travel}
\appcontentsentry{1em}{app:case-service}
\appcontentsentry{1em}{app:case-finance}
\appcontentsentry{1em}{app:case-coding}
\end{multicols}
\endgroup

\section{Shared Protocol Details}
\label{app:protocol}
\input{appendix/protocol}

\clearpage
\section{Models, Runs and Coverage}
\label{app:runs}
\input{appendix/runs}

\clearpage
\section{Health: MedDialogRubrics}
\label{app:health}
\input{appendix/health}

\clearpage
\section{Coding: LiveCodeBench}
\label{app:coding}
\input{appendix/coding}

\clearpage
\section{Math: SimulatorArena-MATH, HARP and IMO-ProofBench}
\label{app:math}
\input{appendix/math}

\clearpage
\section{Finance: PRBench}
\label{app:finance}
\input{appendix/finance}

\clearpage
\section{Customer Service: ABCD Policy Cases}
\label{app:service}
\input{appendix/service}

\clearpage
\section{Travel: UserBench and Revision Tasks}
\label{app:travel}
\input{appendix/travel}

\clearpage
\section{Case Studies}
\label{app:cases}
\input{appendix/cases}
