# Supplementary material for: PersonaChatBench: Evaluating Chat Assistants with Diverse Simulated Users
Source: arXiv:2610.42060 source file (2026-10-30)
Supplement: Supplementary file 25 [file supp_coding.tex]

\begin{table}[H]
\centering
\caption{\textbf{Coding, 20 hard LiveCodeBench tasks.} Persona pass is conditional on publicly expressed critical needs (analysis version \emph{publicly-expressed-critical-needs-v1}); intervals are 95\% Wilson and treat episodes as independent. Critical needs counts are needs with a public request and an assistant reply over applicable critical needs. Source: examples/coding-hard20-paper-reference.}
\label{tab:supp-coding}
\begingroup
\scriptsize\setstretch{1.0}
\setlength{\tabcolsep}{3pt}
\renewcommand{\arraystretch}{1.15}
\begin{tabular}{@{}lrrrr@{}}
\toprule
\textbf{Card} & \textbf{Tests passed} & \textbf{Persona pass (\%)} & \textbf{Critical needs answered (\%)} & \textbf{Need credit} \\
\midrule
Detailed typed professional & 18/20 & 100.0 {\scriptsize [83.9, 100.0]} (20/20) & 87.0 (40/46) & 0.97 \\
Concise skeptical professional & 20/20 & 90.0 {\scriptsize [69.9, 97.2]} (18/20) & 92.0 (46/50) & 0.97 \\
Performance-focused student & 19/19 & 66.7 {\scriptsize [43.7, 83.7]} (12/18) & 71.4 (60/84) & 0.95 \\
Trade-off-focused professional & 19/19 & 89.5 {\scriptsize [68.6, 97.1]} (17/19) & 97.2 (35/36) & 0.97 \\
Maintainability-minded reviewer & 20/20 & 73.7 {\scriptsize [51.2, 88.2]} (14/19) & 83.1 (54/65) & 0.92 \\
Deadline-driven technologist & 20/20 & 73.7 {\scriptsize [51.2, 88.2]} (14/19) & 51.5 (51/99) & 0.96 \\
Simple-performance reviewer & 20/20 & 85.0 {\scriptsize [64.0, 94.8]} (17/20) & 69.7 (53/76) & 0.97 \\
Dependency-minimal explainer & 19/20 & 95.0 {\scriptsize [76.4, 99.1]} (19/20) & 73.2 (52/71) & 0.99 \\
Examples-first minimalist & 20/20 & 75.0 {\scriptsize [53.1, 88.8]} (15/20) & 95.0 (76/80) & 0.96 \\
Plain-language technologist & 19/19 & 89.5 {\scriptsize [68.6, 97.1]} (17/19) & 43.1 (25/58) & 0.90 \\
Test-oriented hobbyist & 20/20 & 72.2 {\scriptsize [49.1, 87.5]} (13/18) & 72.4 (55/76) & 0.96 \\
Examples-first learner & 19/19 & 68.4 {\scriptsize [46.0, 84.6]} (13/19) & 86.4 (89/103) & 0.95 \\
\midrule
\textbf{all 12 cards} & 233/236 & 81.8 {\scriptsize [76.3, 86.3]} (189/231) & 75.4 (636/844) & 0.96 \\
\bottomrule
\end{tabular}
\endgroup
\end{table}
