# Supplementary material for: PersonaChatBench: Evaluating Chat Assistants with Diverse Simulated Users
Source: arXiv:2610.42060 source file (2026-10-30)
Supplement: Supplementary file 26 [file supp_finance.tex]

\begin{table}[H]
\centering
\caption{\textbf{Finance, round 1 (all 361 tasks).} Values are gpt-5.6-sol / gpt-6-astra. Advice scores are PRBench rubric percentages over the whole conversation and over the last assistant message; persona pass and joint pass are percentages of conversations. Source: examples/persona-trials/README.md.}
\label{tab:supp-finance}
\begingroup
\scriptsize\setstretch{1.0}
\setlength{\tabcolsep}{3pt}
\renewcommand{\arraystretch}{1.15}
\begin{tabular}{@{}lrrrr@{}}
\toprule
\textbf{Condition} & \textbf{Advice, whole} & \textbf{Advice, last} & \textbf{Persona pass (\%)} & \textbf{Joint (\%)} \\
\midrule
neutral & 49.5 / 50.5 & 46.8 / 47.3 & -- & -- \\
skeptical questioner & 53.2 / 52.1 & 40.0 / 39.6 & 83 / 98 & 47 / 54 \\
designed (5 per task) & 54.2 / 53.5 & 39.6 / 38.4 & 74 / 94 & 44 / 55 \\
confident contrarian & 52.6 / 52.2 & 36.8 / 32.8 & 88 / 99 & 51 / 55 \\
concise pragmatist & 49.4 / 49.9 & 30.7 / 28.2 & 99 / 100 & 52 / 51 \\
decisive pusher & 49.4 / 50.9 & 25.2 / 25.0 & 95 / 100 & 49 / 49 \\
reassurance seeker & 49.3 / 50.4 & 23.8 / 22.4 & 97 / 100 & 50 / 52 \\
careful learner & 49.6 / 49.9 & 25.8 / 21.6 & 34 / 77 & 17 / 41 \\
\bottomrule
\end{tabular}
\endgroup
\end{table}
