# Supplementary material for: PersonaChatBench: Evaluating Chat Assistants with Diverse Simulated Users
Source: arXiv:2610.42060 source file (2026-10-30)
Supplement: Supplementary file 27 [file supp_health.tex]

\begin{table}[H]
\centering
\caption{\textbf{Health, 10 cases $\times$ (5 personas + neutral) $\times$ 2 anonymous doctor configurations.} Inquiry coverage is not diagnostic accuracy. Persona demonstration is the share of attribute items with an opportunity that were clearly shown. Need credit is conditional on a scoreable need (number of cases of 10 in parentheses). Source: healthbench-benchmark/examples/RESULTS.md.}
\label{tab:supp-health}
\begingroup
\scriptsize\setstretch{1.0}
\setlength{\tabcolsep}{3pt}
\renewcommand{\arraystretch}{1.15}
\begin{tabular}{@{}lrrrr@{}}
\toprule
\textbf{Persona / doctor} & \textbf{Inquiry} & \textbf{Facts} & \textbf{Demonstration} & \textbf{Need credit (scoreable)} \\
\midrule
P1 / Doctor A & 50.8 & 71.2 & 76.3 & 100.0 (7/10) \\
P1 / Doctor B & 46.7 & 77.5 & 76.7 & 90.6 (8/10) \\
P2 / Doctor A & 45.6 & 66.4 & 61.1 & 100.0 (1/10) \\
P2 / Doctor B & 47.9 & 78.2 & 65.8 & 100.0 (1/10) \\
P3 / Doctor A & 44.9 & 79.2 & 88.3 & 100.0 (7/10) \\
P3 / Doctor B & 49.5 & 78.6 & 85.2 & 100.0 (8/10) \\
P4 / Doctor A & 49.4 & 85.8 & 93.8 & 100.0 (10/10) \\
P4 / Doctor B & 60.0 & 86.8 & 91.5 & 100.0 (10/10) \\
P5 / Doctor A & 52.3 & 80.1 & 77.9 & 100.0 (4/10) \\
P5 / Doctor B & 47.0 & 77.9 & 65.1 & 100.0 (4/10) \\
NEUTRAL / Doctor A & 45.2 & 78.5 & -- & -- \\
NEUTRAL / Doctor B & 51.3 & 86.7 & -- & -- \\
\bottomrule
\end{tabular}
\endgroup
\end{table}
