# Supplementary material for: PersonaChatBench: Evaluating Chat Assistants with Diverse Simulated Users
Source: arXiv:2610.42060 source file (2026-10-30)
Supplement: Supplementary file 28 [file supp_help.tex]

\begin{table}[H]
\centering
\caption{\textbf{HelpBench, 450 tasks (v2 protocol).} Planned 2,250, completed 2,161, graded 2,086, valid 2,081. Task score is the trajectory rubric score; persona adherence is evaluated only after disclosure. Source: examples/gpt6-astra-attributes-v2-450-task/SUMMARY.md.}
\label{tab:supp-help}
\begingroup
\scriptsize\setstretch{1.0}
\setlength{\tabcolsep}{3pt}
\renewcommand{\arraystretch}{1.15}
\begin{tabular}{@{}lrrr@{}}
\toprule
\textbf{Condition} & \textbf{Valid / planned} & \textbf{Task score (\%)} & \textbf{Adherence (\%)} \\
\midrule
neutral\_multi / neutral & 417/450 & 81.82 (n=417) & -- \\
persona\_multi / careful\_learner & 412/450 & 82.75 (n=412) & 99.86 (n=365) \\
persona\_multi / concise\_pragmatist & 419/450 & 81.35 (n=419) & 99.48 (n=240) \\
persona\_multi / skeptical\_questioner & 406/450 & 81.77 (n=406) & 99.92 (n=396) \\
single\_turn / neutral & 427/450 & 79.77 (n=427) & -- \\
\bottomrule
\end{tabular}
\endgroup
\end{table}
