# Supplementary material for: PersonaChatBench: Evaluating Chat Assistants with Diverse Simulated Users
Source: arXiv:2610.42060 source file (2026-10-30)
Supplement: Supplementary file 29 [file supp_law.tex]

\begin{table}[H]
\centering
\caption{\textbf{Law, 59 cases $\times$ 5 archetypes (client gpt-5.6-sol).} Resolution $=\frac12$(Fact + Issue Resolution); adherence is the client persona judge's score and its components (percent). Means are taken within each jurisdiction and then across jurisdictions. Source: examples/gpt-5.6-sol-simulation-astra-judge-all-cases/SUMMARY.md.}
\label{tab:supp-law}
\begingroup
\scriptsize\setstretch{1.0}
\setlength{\tabcolsep}{2.4pt}
\renewcommand{\arraystretch}{1.15}
\begin{tabular}{@{}lrrrrrrrrr@{}}
\toprule
\textbf{Archetype} & \textbf{Res.} & \textbf{Fact} & \textbf{Issue} & \textbf{Adher.} & \textbf{Arch.} & \textbf{Attr.} & \textbf{Goal} & \textbf{Facts} & \textbf{Rules} \\
\midrule
Assured cooperator & 39.9 & 52.6 & 27.2 & 80.9 & 100.0 & 79.0 & 100.0 & 39.8 & 89.0 \\
Dependent and anxious & 34.7 & 49.7 & 19.8 & 76.8 & 87.3 & 76.2 & 100.0 & 27.0 & 93.2 \\
Avoidant and withdrawn & 39.2 & 51.8 & 26.6 & 76.5 & 83.0 & 76.3 & 100.0 & 28.7 & 90.7 \\
Controlling resister & 41.0 & 53.1 & 28.9 & 77.3 & 83.1 & 77.0 & 100.0 & 36.2 & 87.3 \\
Trusting but impatient & 34.8 & 47.9 & 21.6 & 76.2 & 63.5 & 78.0 & 98.3 & 33.1 & 93.2 \\
\midrule
overall & 37.9 & 51.0 & 24.8 & 77.5 & 83.4 & 77.3 & 99.7 & 32.9 & 90.7 \\
PRC cases & 37.3 & 41.8 & 32.9 & 77.8 & 83.1 & 78.0 & 100.0 & 26.2 & 92.4 \\
U.S. cases & 38.5 & 60.2 & 16.8 & 77.3 & 83.7 & 76.6 & 99.3 & 39.7 & 89.0 \\
\bottomrule
\end{tabular}
\endgroup
\end{table}
