# Supplementary material for: PersonaChatBench: Evaluating Chat Assistants with Diverse Simulated Users
Source: arXiv:2610.42060 source file (2026-10-30)
Supplement: Supplementary file 30 [file supp_needtypes.tex]

\begin{table}[H]
\centering
\caption{\textbf{Coding need types.} The classification is an analysis choice made for this paper. A need \emph{asks for content} if the user can request additional material in the conversation, and \emph{constrains form} if it states a property of the delivered code that a user would normally expect by default. Counts are for critical needs: expressed and answered over applicable, and satisfied / partially satisfied among answered.}
\label{tab:need-types}
\begingroup
\scriptsize\setstretch{1.0}
\setlength{\tabcolsep}{2.6pt}
\renewcommand{\arraystretch}{1.15}
\begin{tabular}{@{}p{2.6cm}rrr>{\raggedright\arraybackslash}p{7.2cm}@{}}
\toprule
\textbf{Class} & \textbf{Types} & \textbf{Answered / applicable} & \textbf{Sat. / partial} & \textbf{Need types} \\
\midrule
Asks for content & 10 & 574/617 & 526 / 48 & verification\_rationale, detailed\_explanation, concise\_explanation, public\_test\_cases, plain\_language, example\_walkthrough, decision\_tradeoffs, revision\_and\_checks, performance\_check, minimal\_test\_exposition \\
Constrains the artifact's form & 15 & 58/206 & 58 / 0 & type\_annotations, custom\_implementation, low\_complexity, readability, minimal\_dependencies, no\_comments, straightforward\_structure, object\_oriented\_structure, standard\_library\_tools, self\_documenting\_code, extensive\_comments, modular\_structure, compact\_names, docstrings, maintainability \\
Delivery and tone & 3 & 4/21 & 4 / 0 & deadline\_delivery, supportive\_tone, direct\_tone \\
\bottomrule
\end{tabular}
\endgroup
\end{table}
