# Supplementary material for: PersonaChatBench: Evaluating Chat Assistants with Diverse Simulated Users
Source: arXiv:2610.42060 source file (2026-10-30)
Supplement: Supplementary file 31 [file supp_variance.tex]

\begin{table}[H]
\centering
\caption{\textbf{Variance of the native score attributed to task, persona and interaction.} Shares are percentages of the total sum of squares ($\eta^2$, \secref{sec:stats}); the persona share is within task, with a 95\% task-cluster bootstrap interval, and the last column is the 97.5th percentile of its within-task permutation null (1{,}000 permutations). Finance uses round 1 and conversations with a valid simulator audit; HelpBench uses the neutral and the three persona multi-turn arms.}
\label{tab:supp-variance}
\begingroup
\scriptsize\setstretch{1.0}
\setlength{\tabcolsep}{2.6pt}
\renewcommand{\arraystretch}{1.15}
\begin{tabular}{@{}p{4.6cm}rrrrrr@{}}
\toprule
\textbf{Score} & \textbf{n} & \textbf{Tasks / conditions} & \textbf{Task} & \textbf{Persona} & \textbf{Interaction + noise} & \textbf{Null 97.5th} \\
\midrule
Finance, whole conversation, gpt-5.6-sol & 4,203 & 361 / 12 & 87.6 & 1.5 {\scriptsize [1.2, 2.0]} & 10.8 & 0.07 \\
Finance, whole conversation, gpt-6-astra & 4,225 & 361 / 12 & 91.4 & 0.6 {\scriptsize [0.5, 0.9]} & 7.9 & 0.05 \\
Finance, last message, gpt-5.6-sol & 4,215 & 361 / 12 & 50.2 & 12.4 {\scriptsize [10.7, 14.3]} & 37.4 & 0.28 \\
Finance, last message, gpt-6-astra & 4,227 & 361 / 12 & 51.4 & 13.4 {\scriptsize [11.5, 15.7]} & 35.2 & 0.26 \\
HelpBench, trajectory score, gpt-6-astra & 1,654 & 431 / 4 & 91.9 & 0.2 {\scriptsize [0.1, 0.3]} & 7.9 & 0.06 \\
Law, Resolution, client gpt-5.6-sol & 295 & 59 / 5 & 73.1 & 2.6 {\scriptsize [1.4, 5.6]} & 24.3 & 1.27 \\
Law, client adherence & 295 & 59 / 5 & 28.4 & 6.0 {\scriptsize [3.0, 12.1]} & 65.6 & 3.18 \\
Coding, tests passed (binary) & 236 & 20 / 12 & 12.8 & 7.2 {\scriptsize [4.2, 18.7]} & 80.0 & 7.46 \\
\bottomrule
\end{tabular}
\endgroup
\end{table}
